# Supplementary material for: Nebular Spectra of 111 Type Ia Supernovae Disfavor Single Degenerate Progenitors
Source: arXiv:1903.05115 ancillary file (2019-10-31)

**Hel-a**  
**5875 Å**

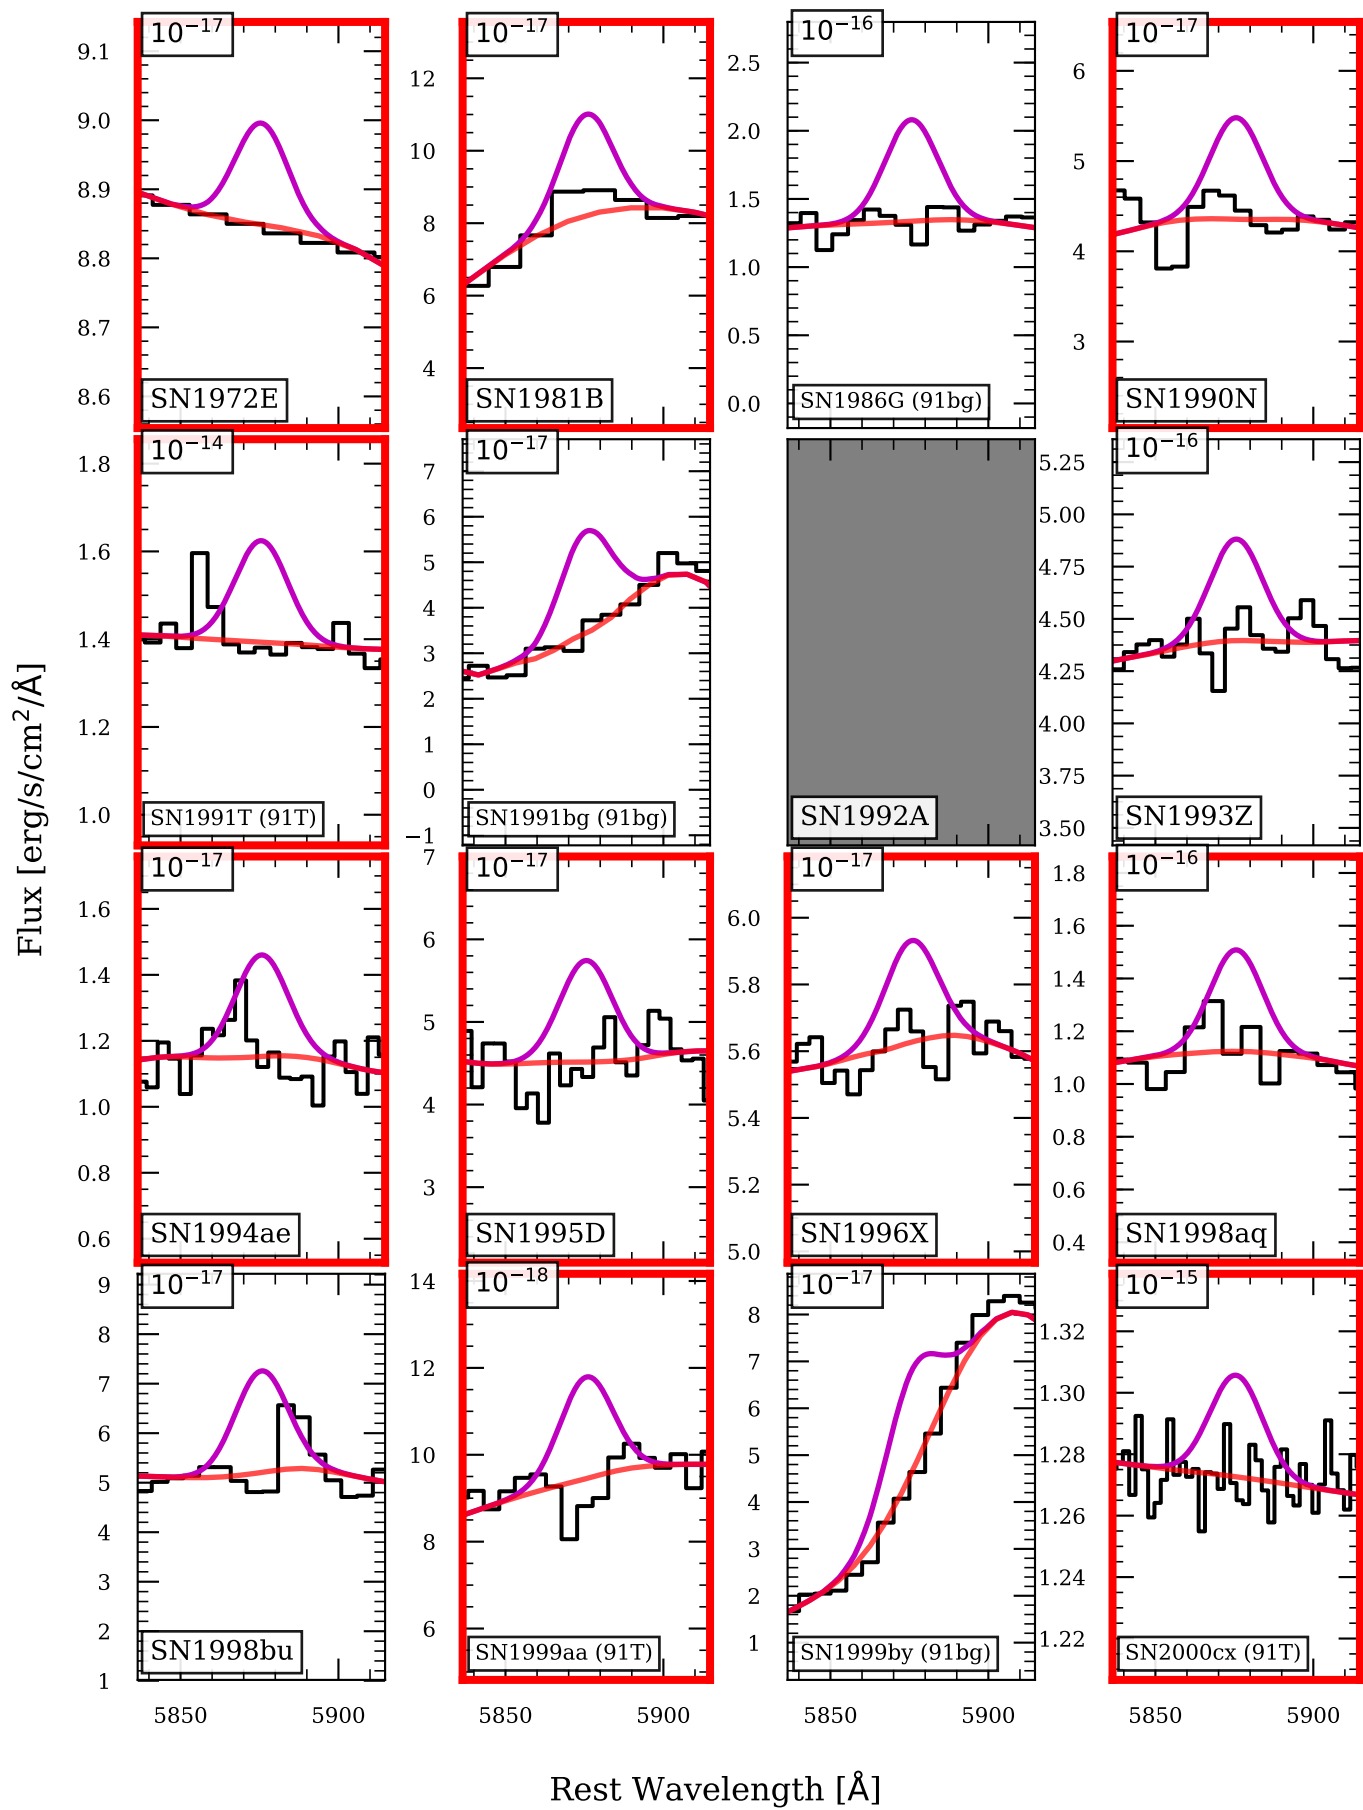

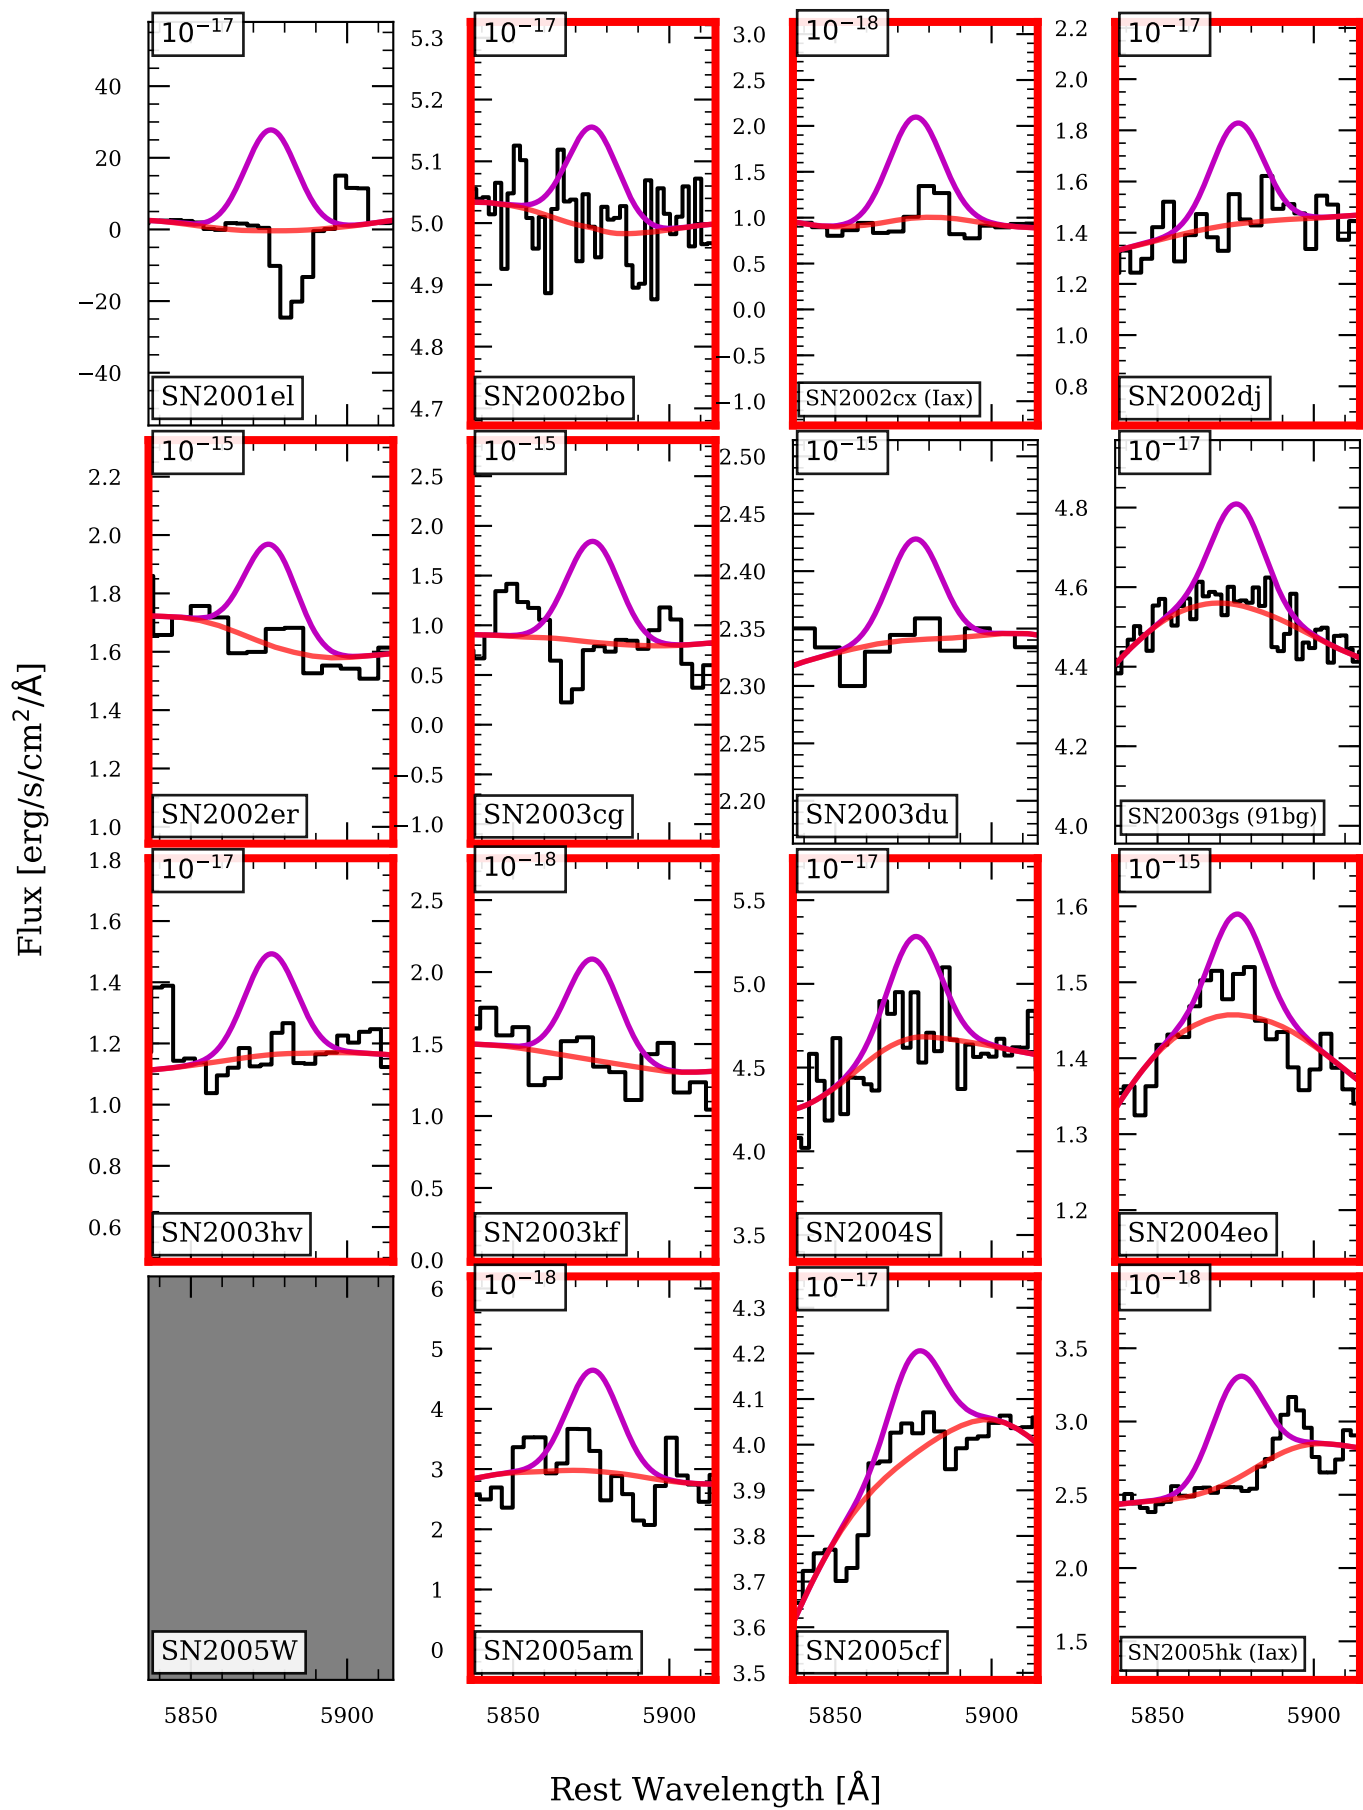

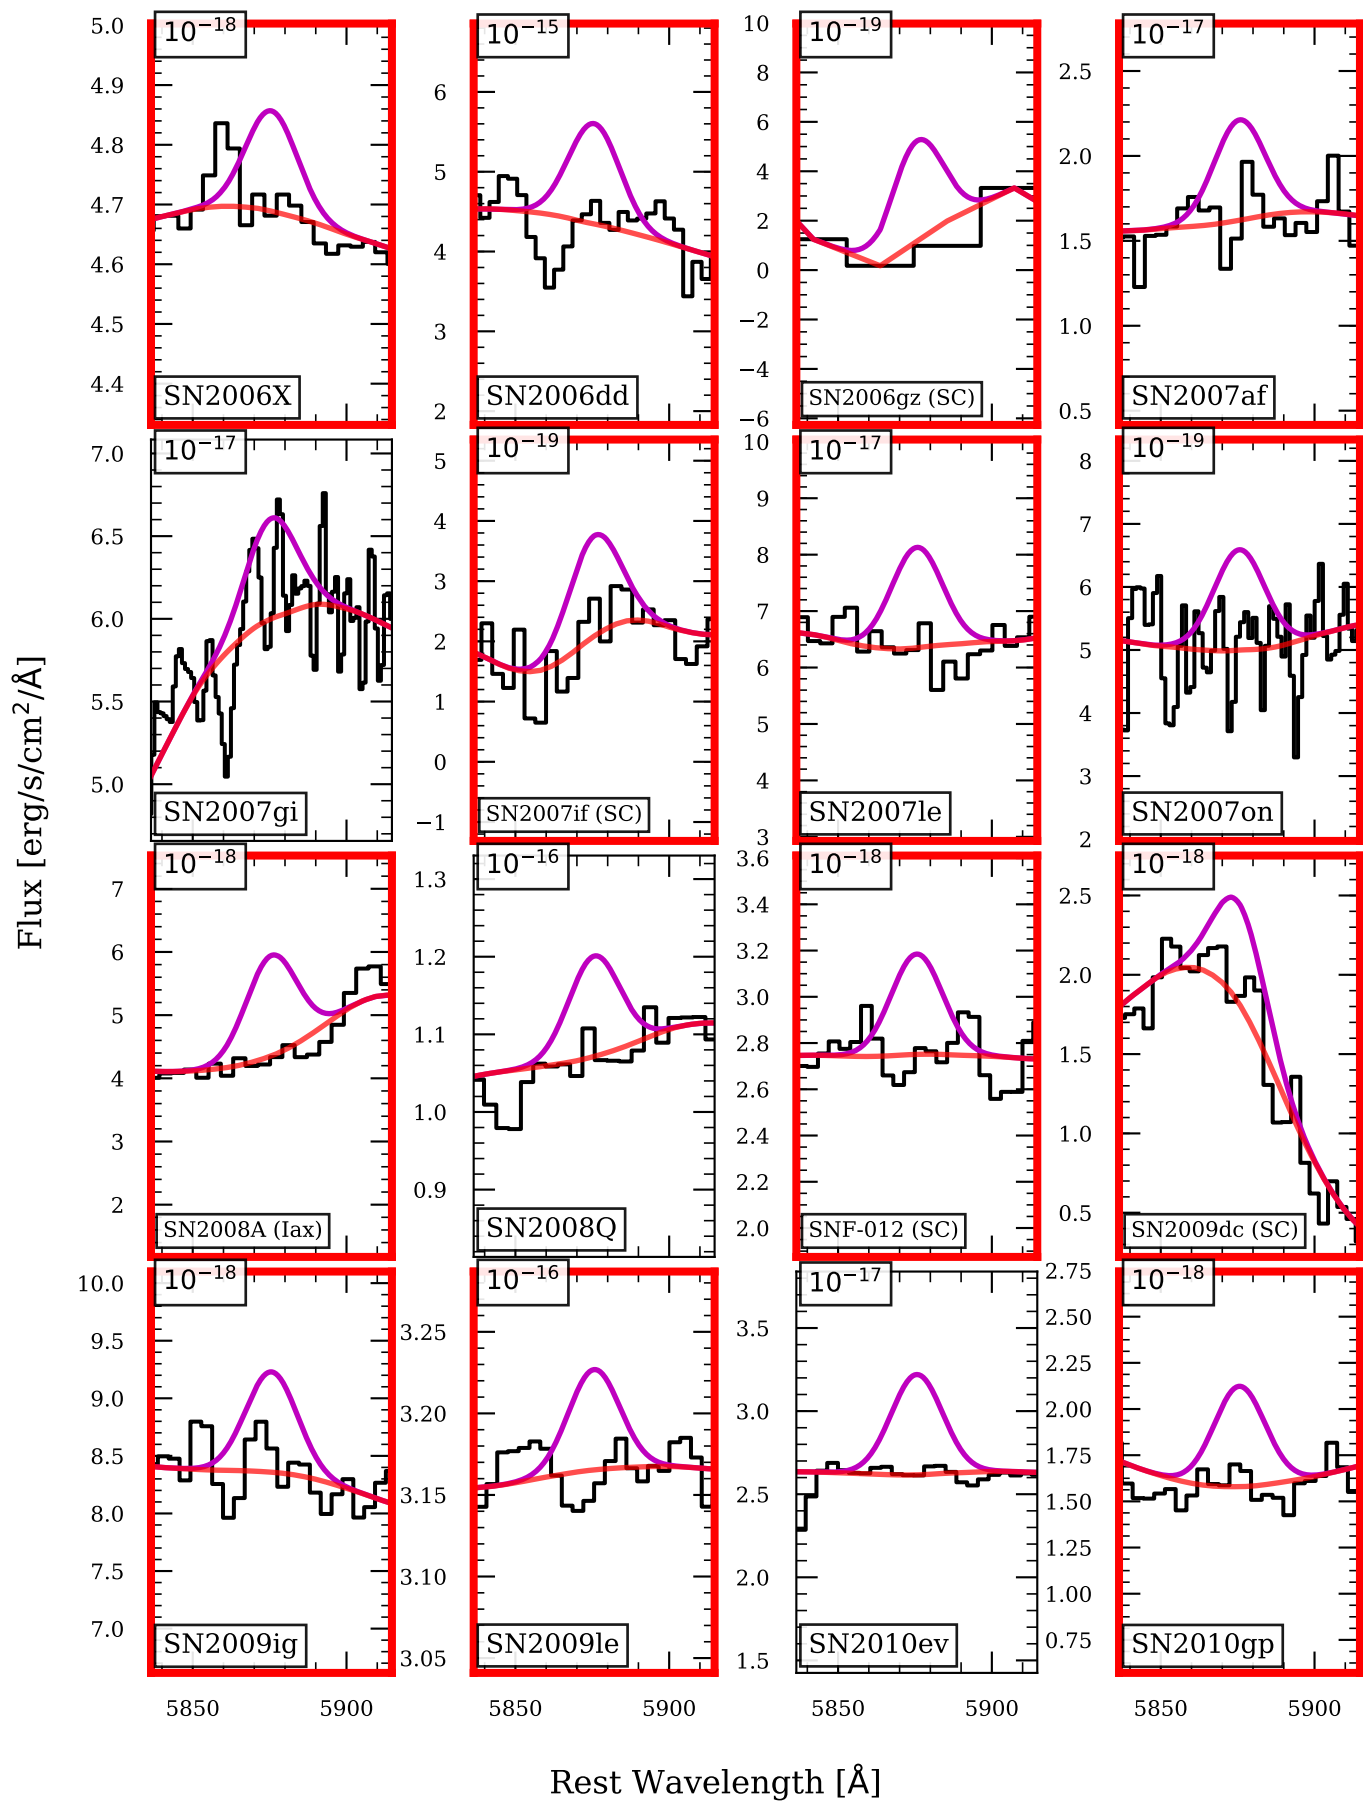

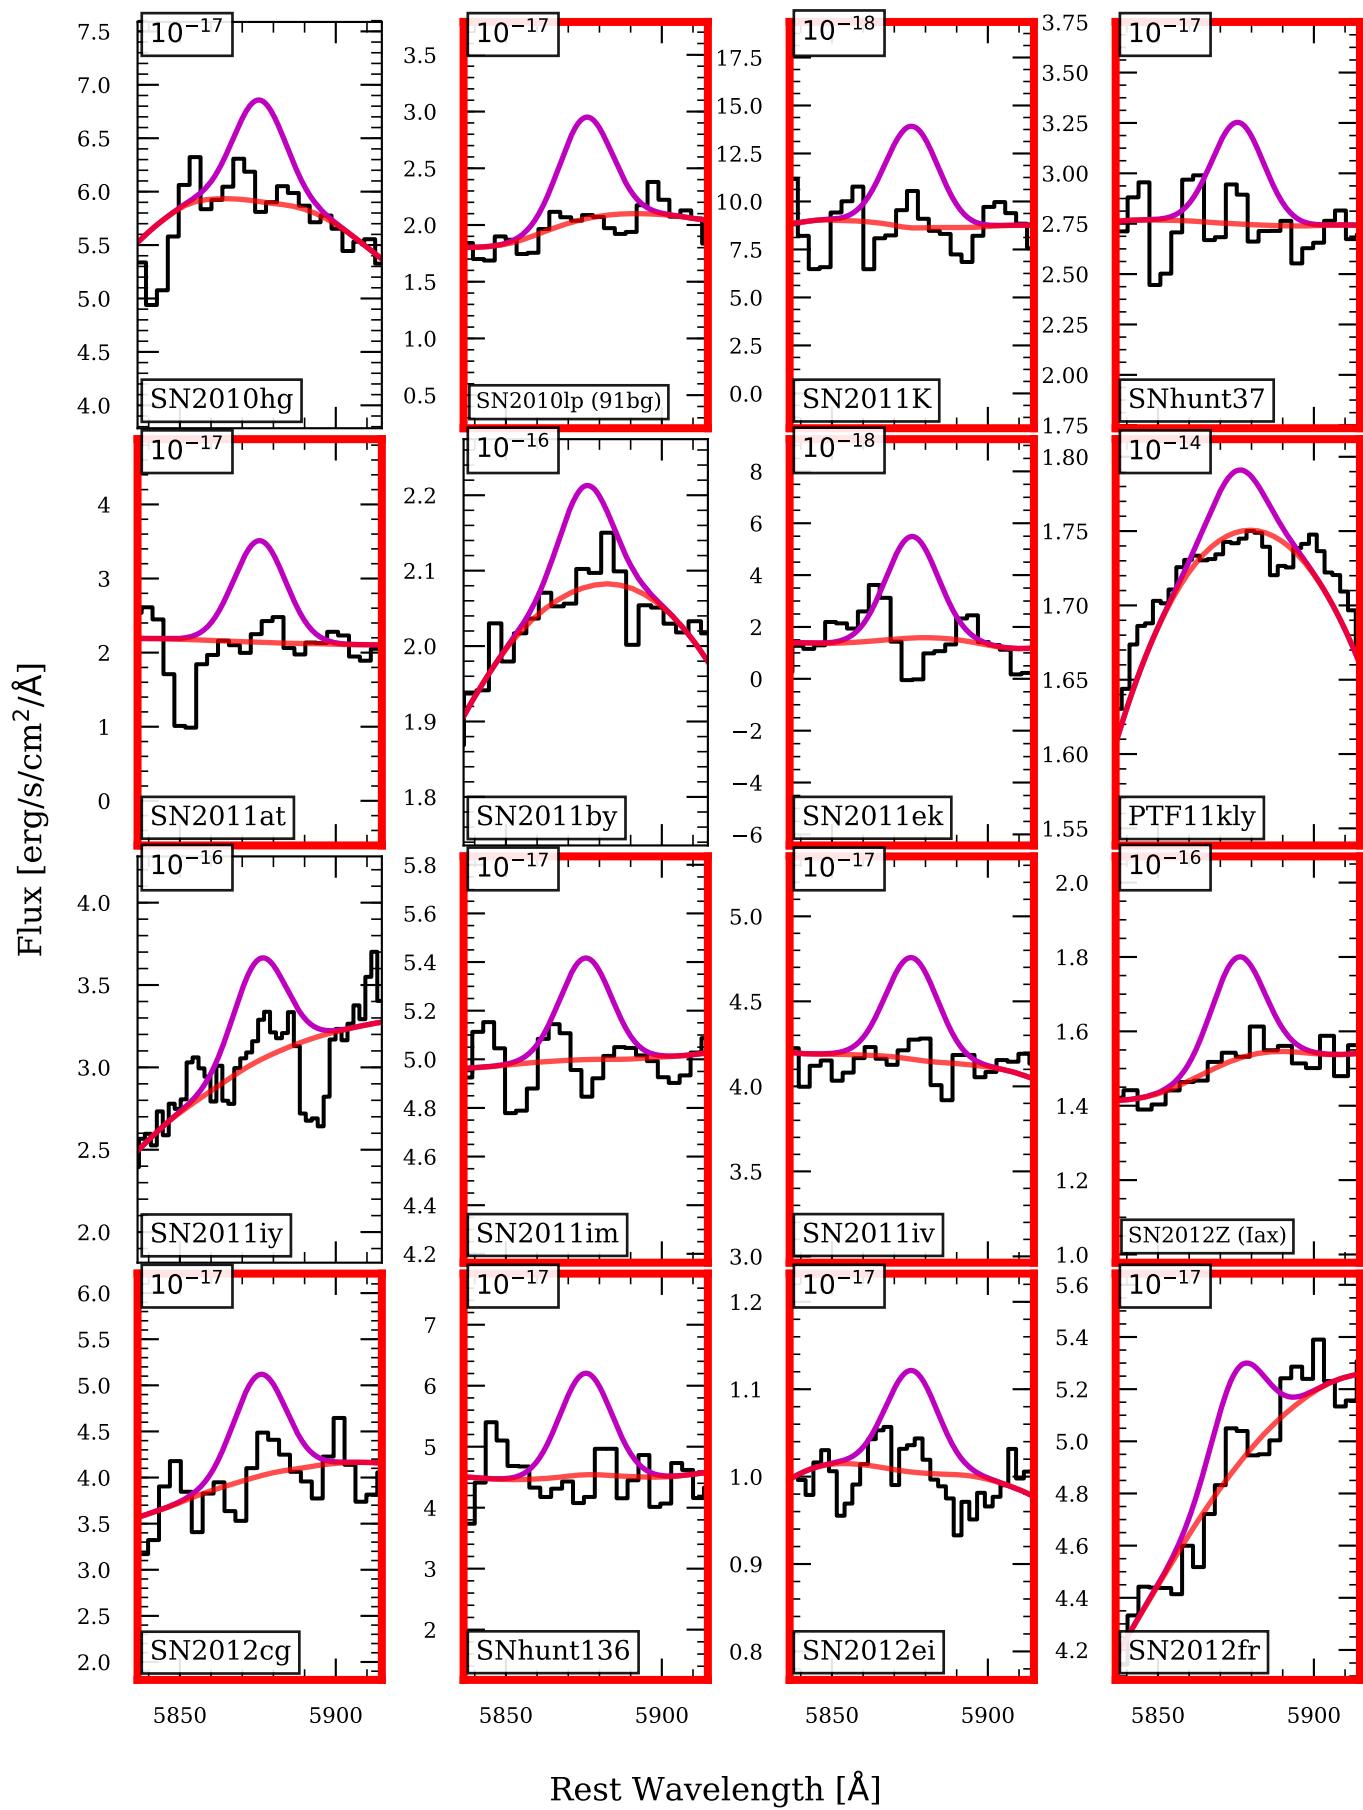

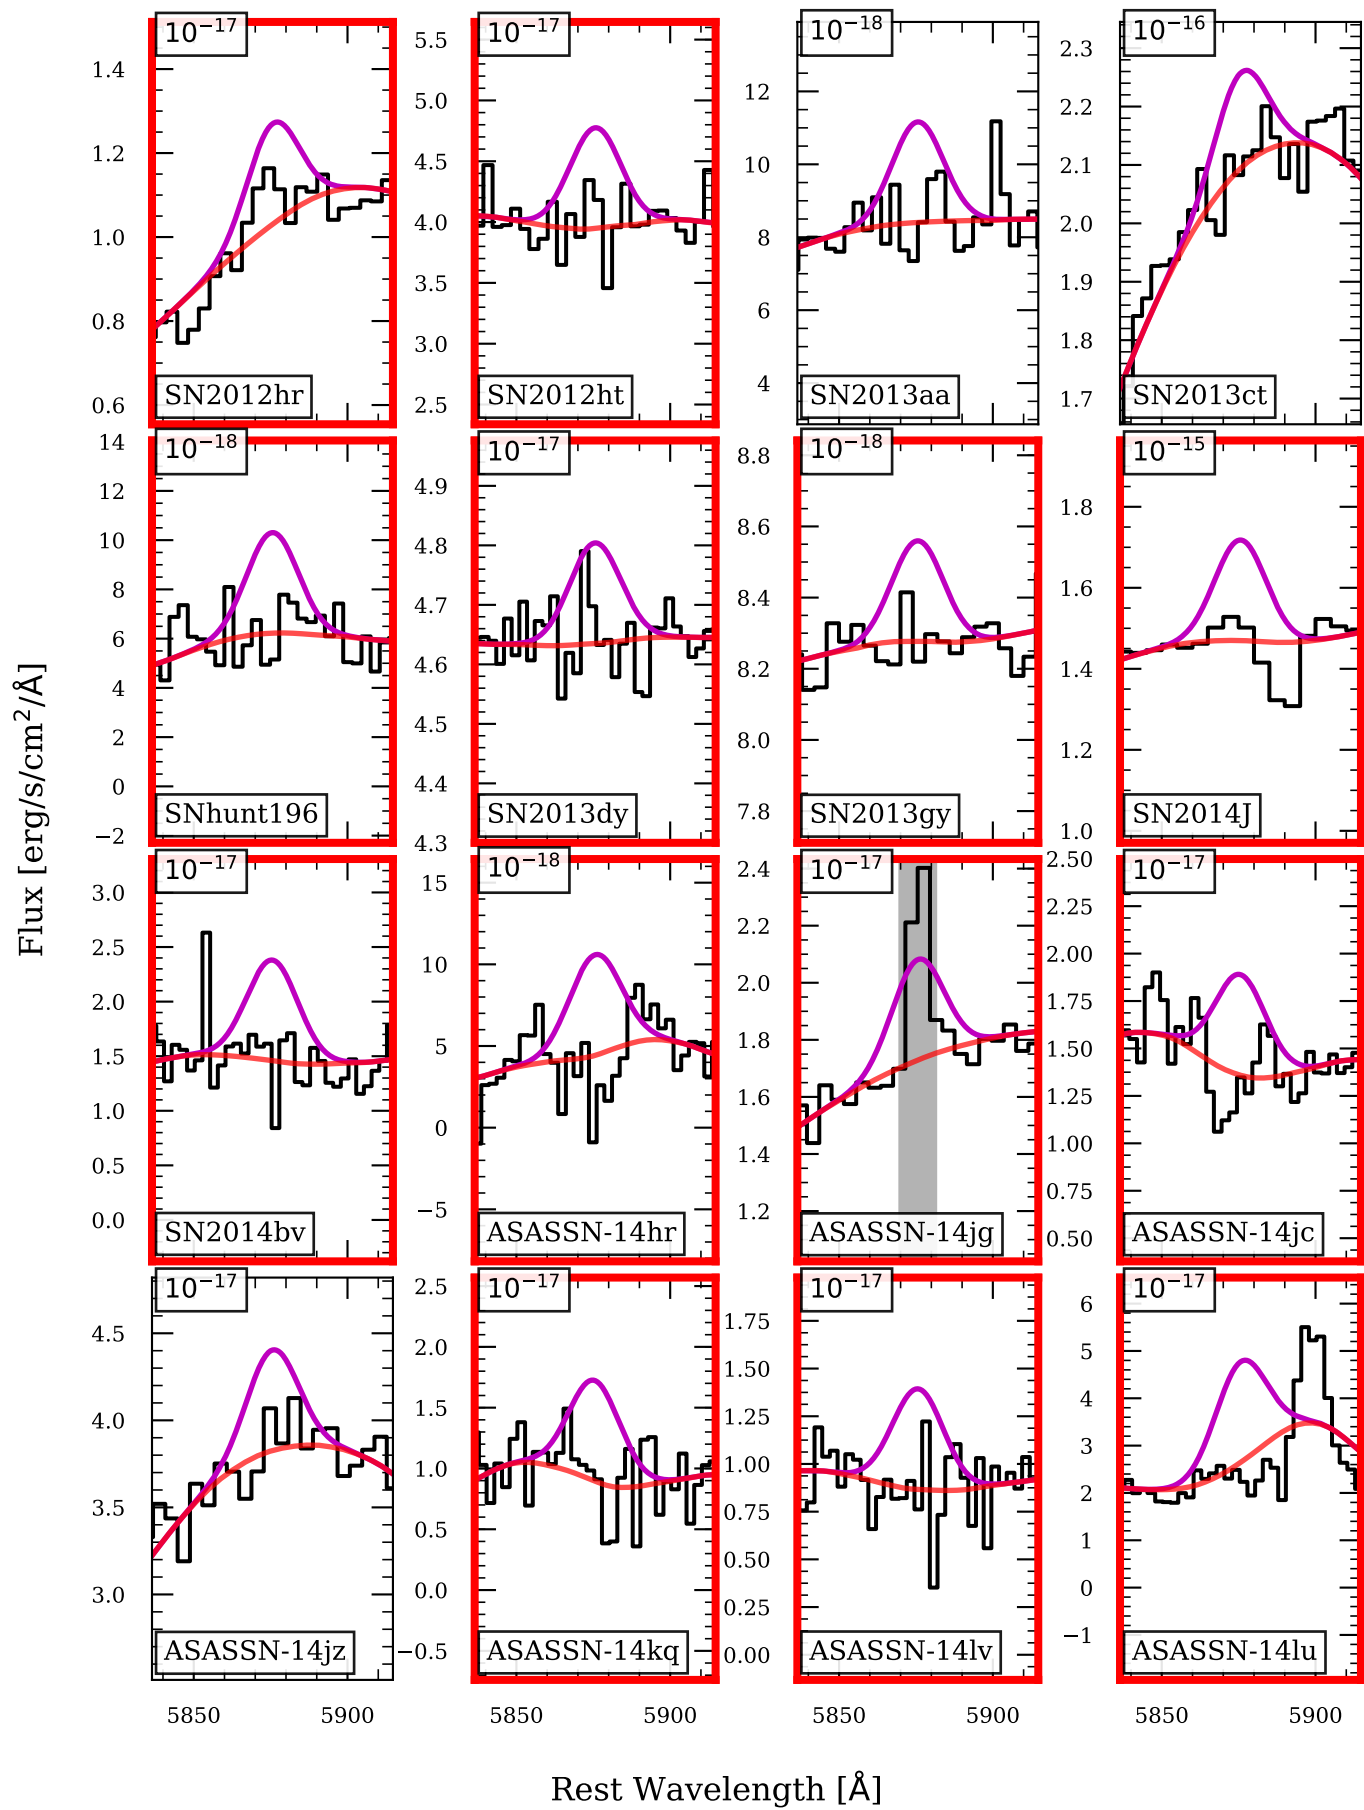

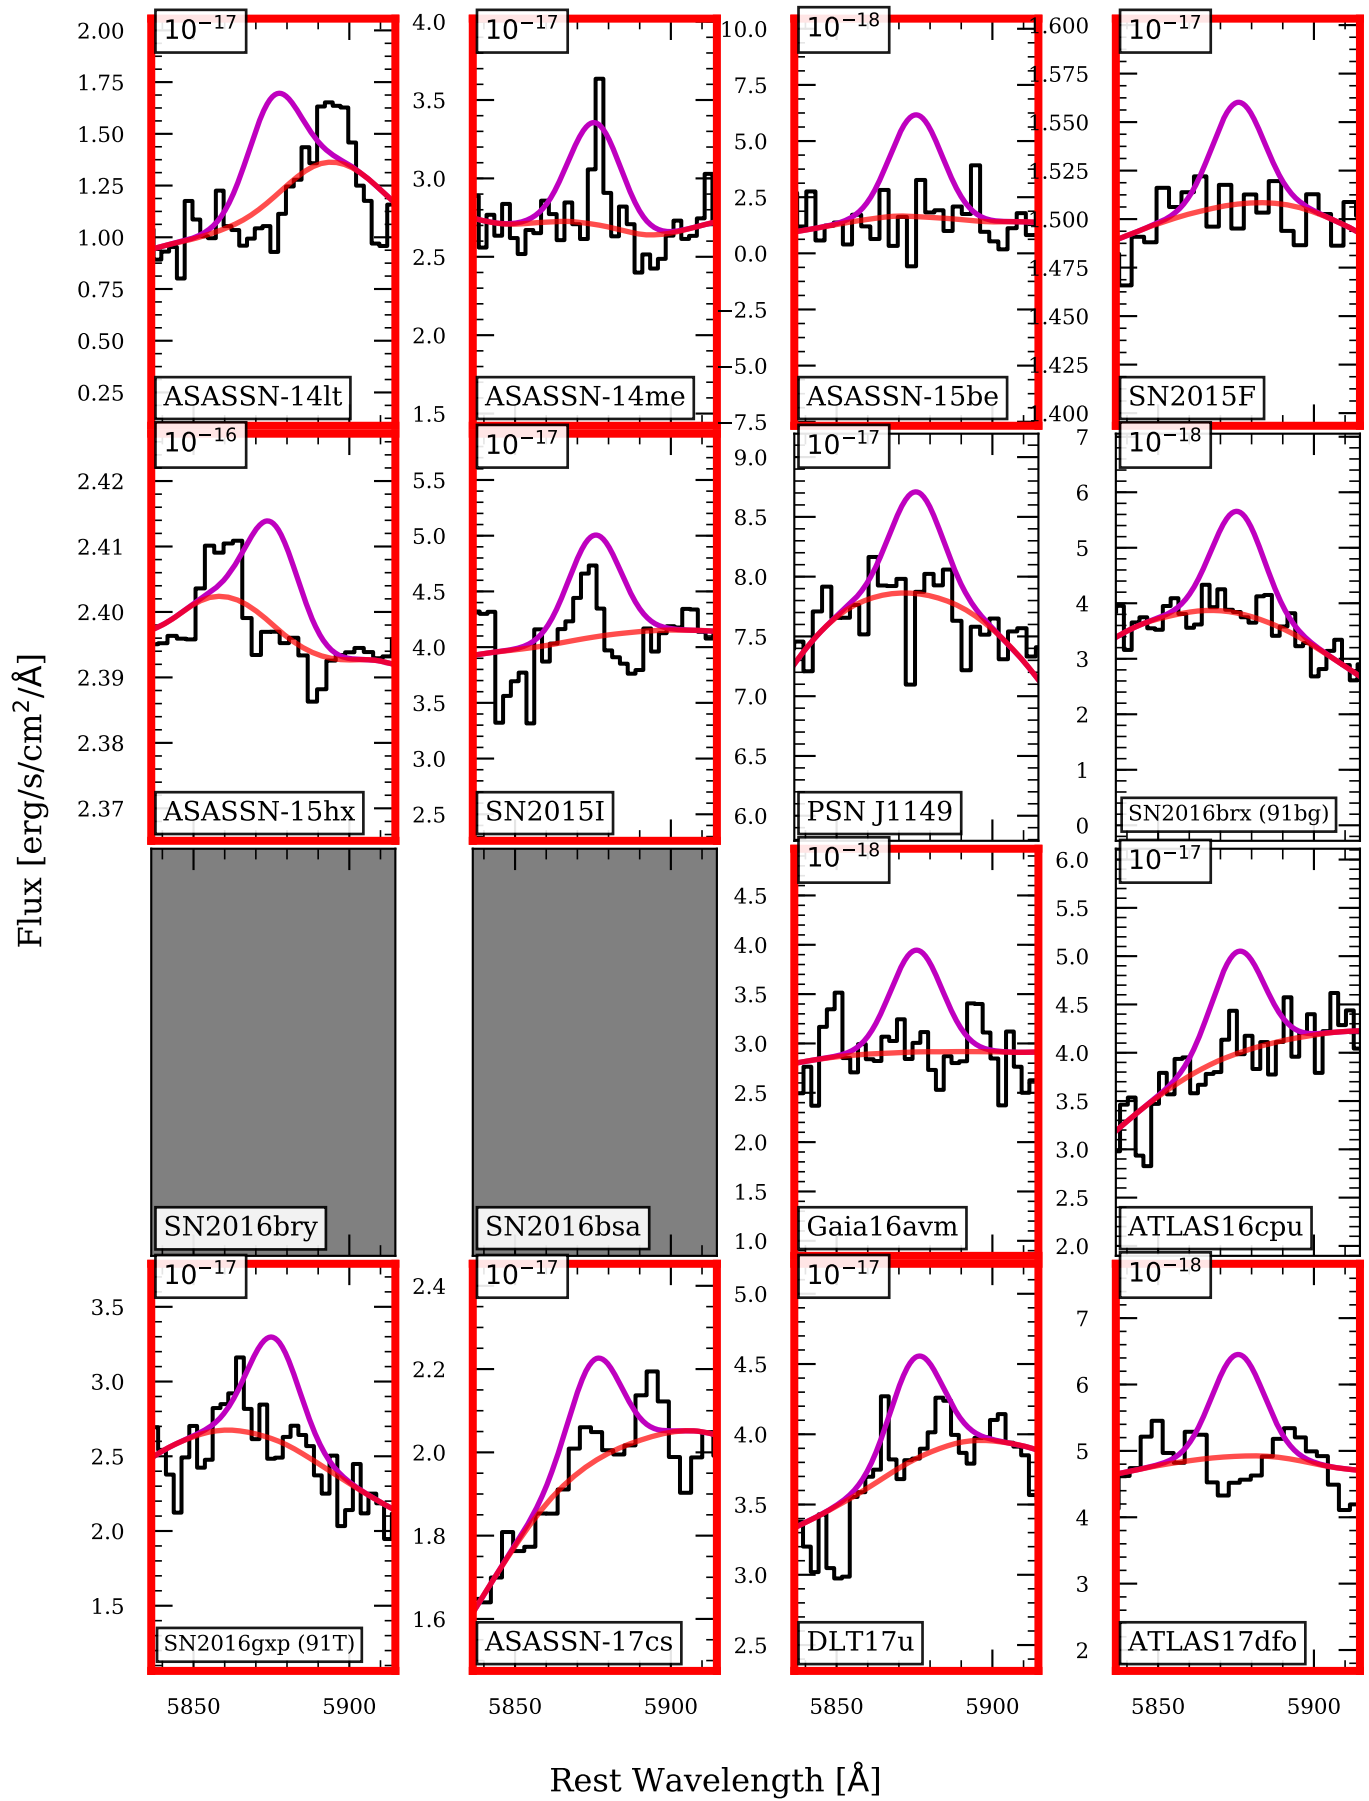

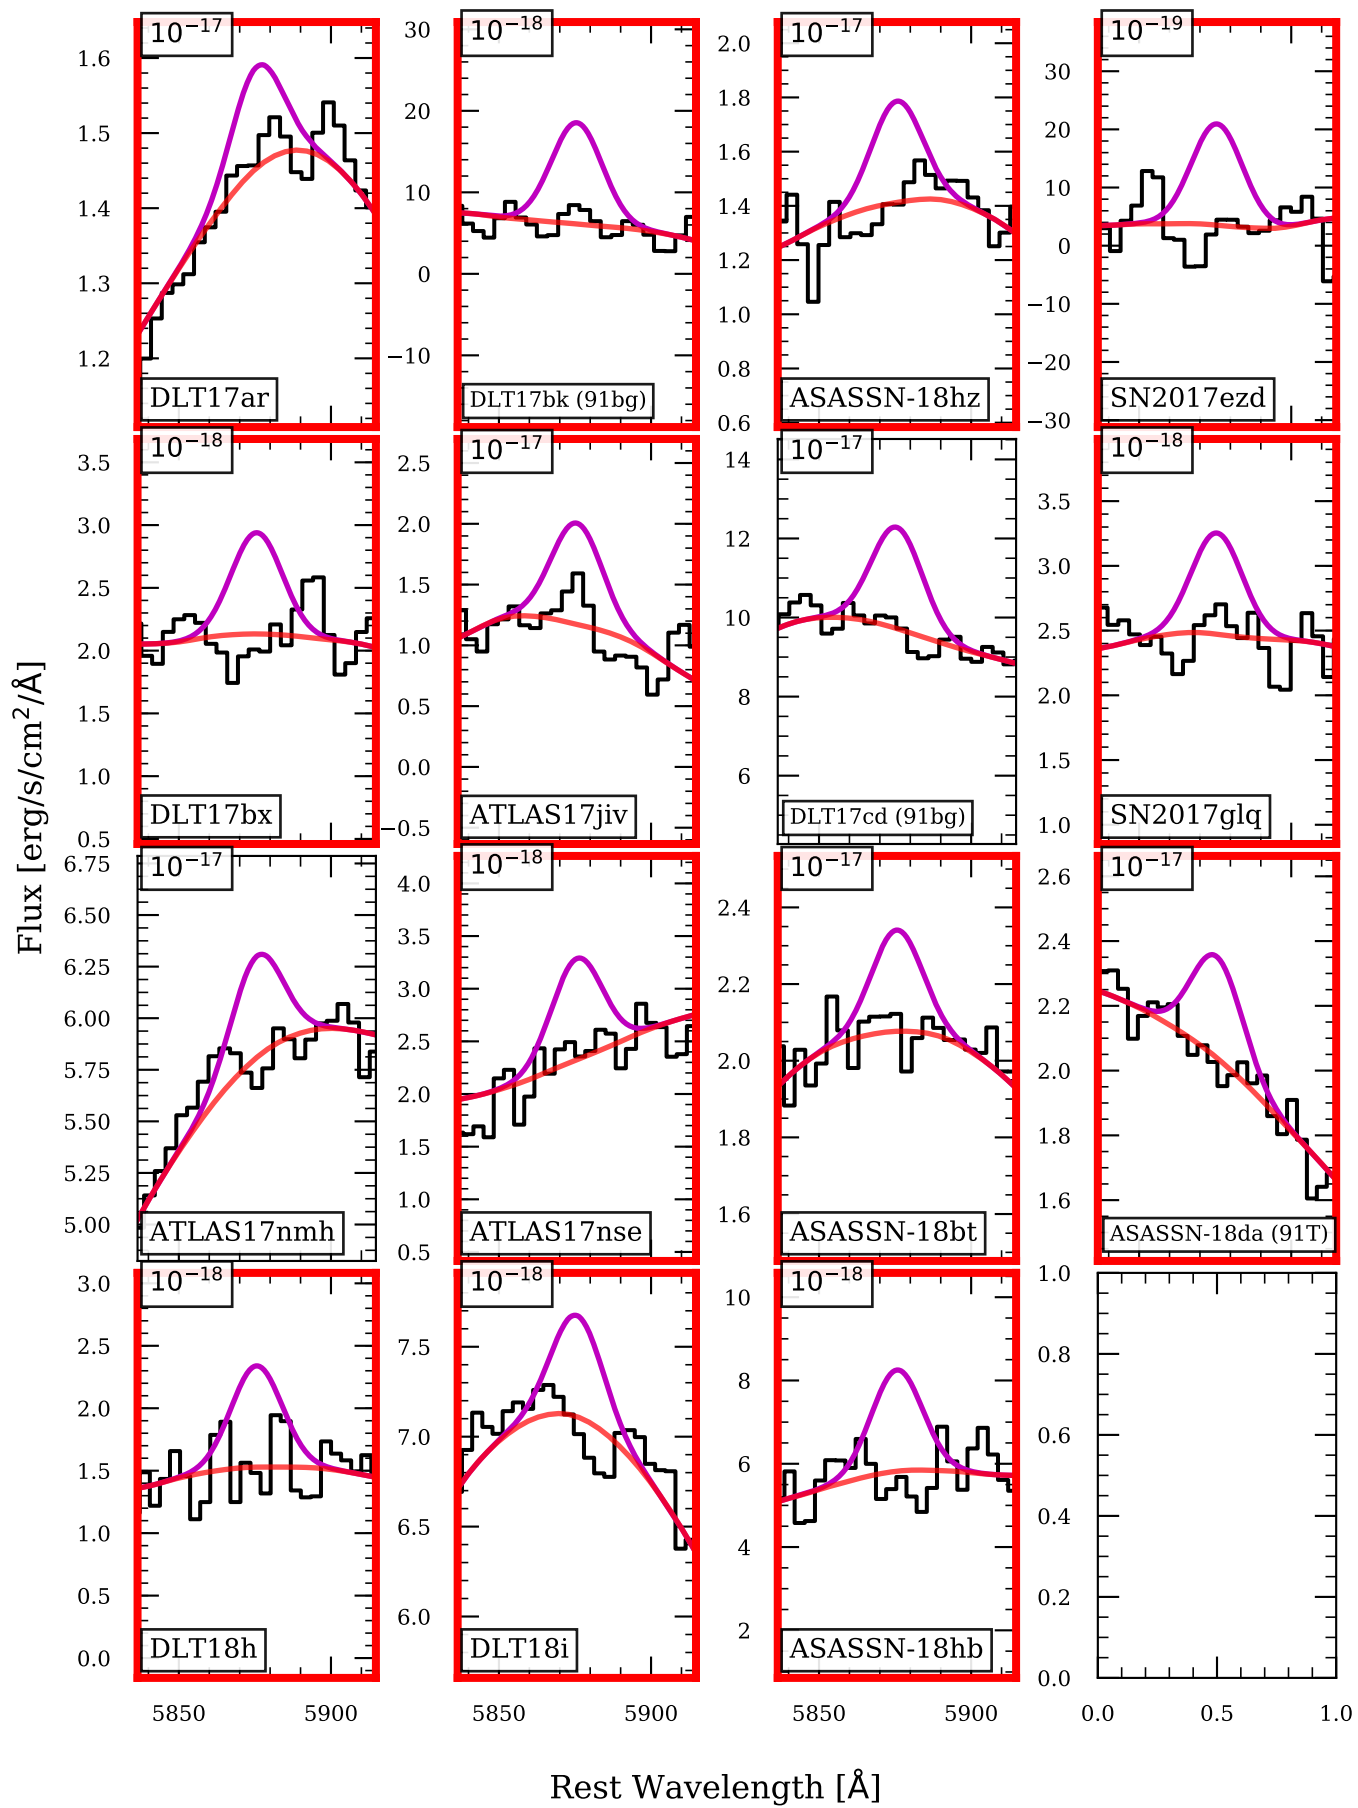

Supplement: Supplementary file 3 [file HeIa-final.pdf]
