# Supplementary material for: Nebular Spectra of 111 Type Ia Supernovae Disfavor Single Degenerate Progenitors
Source: arXiv:1903.05115 ancillary file (2019-10-31)

**HeI-c**  
**10850 Å**

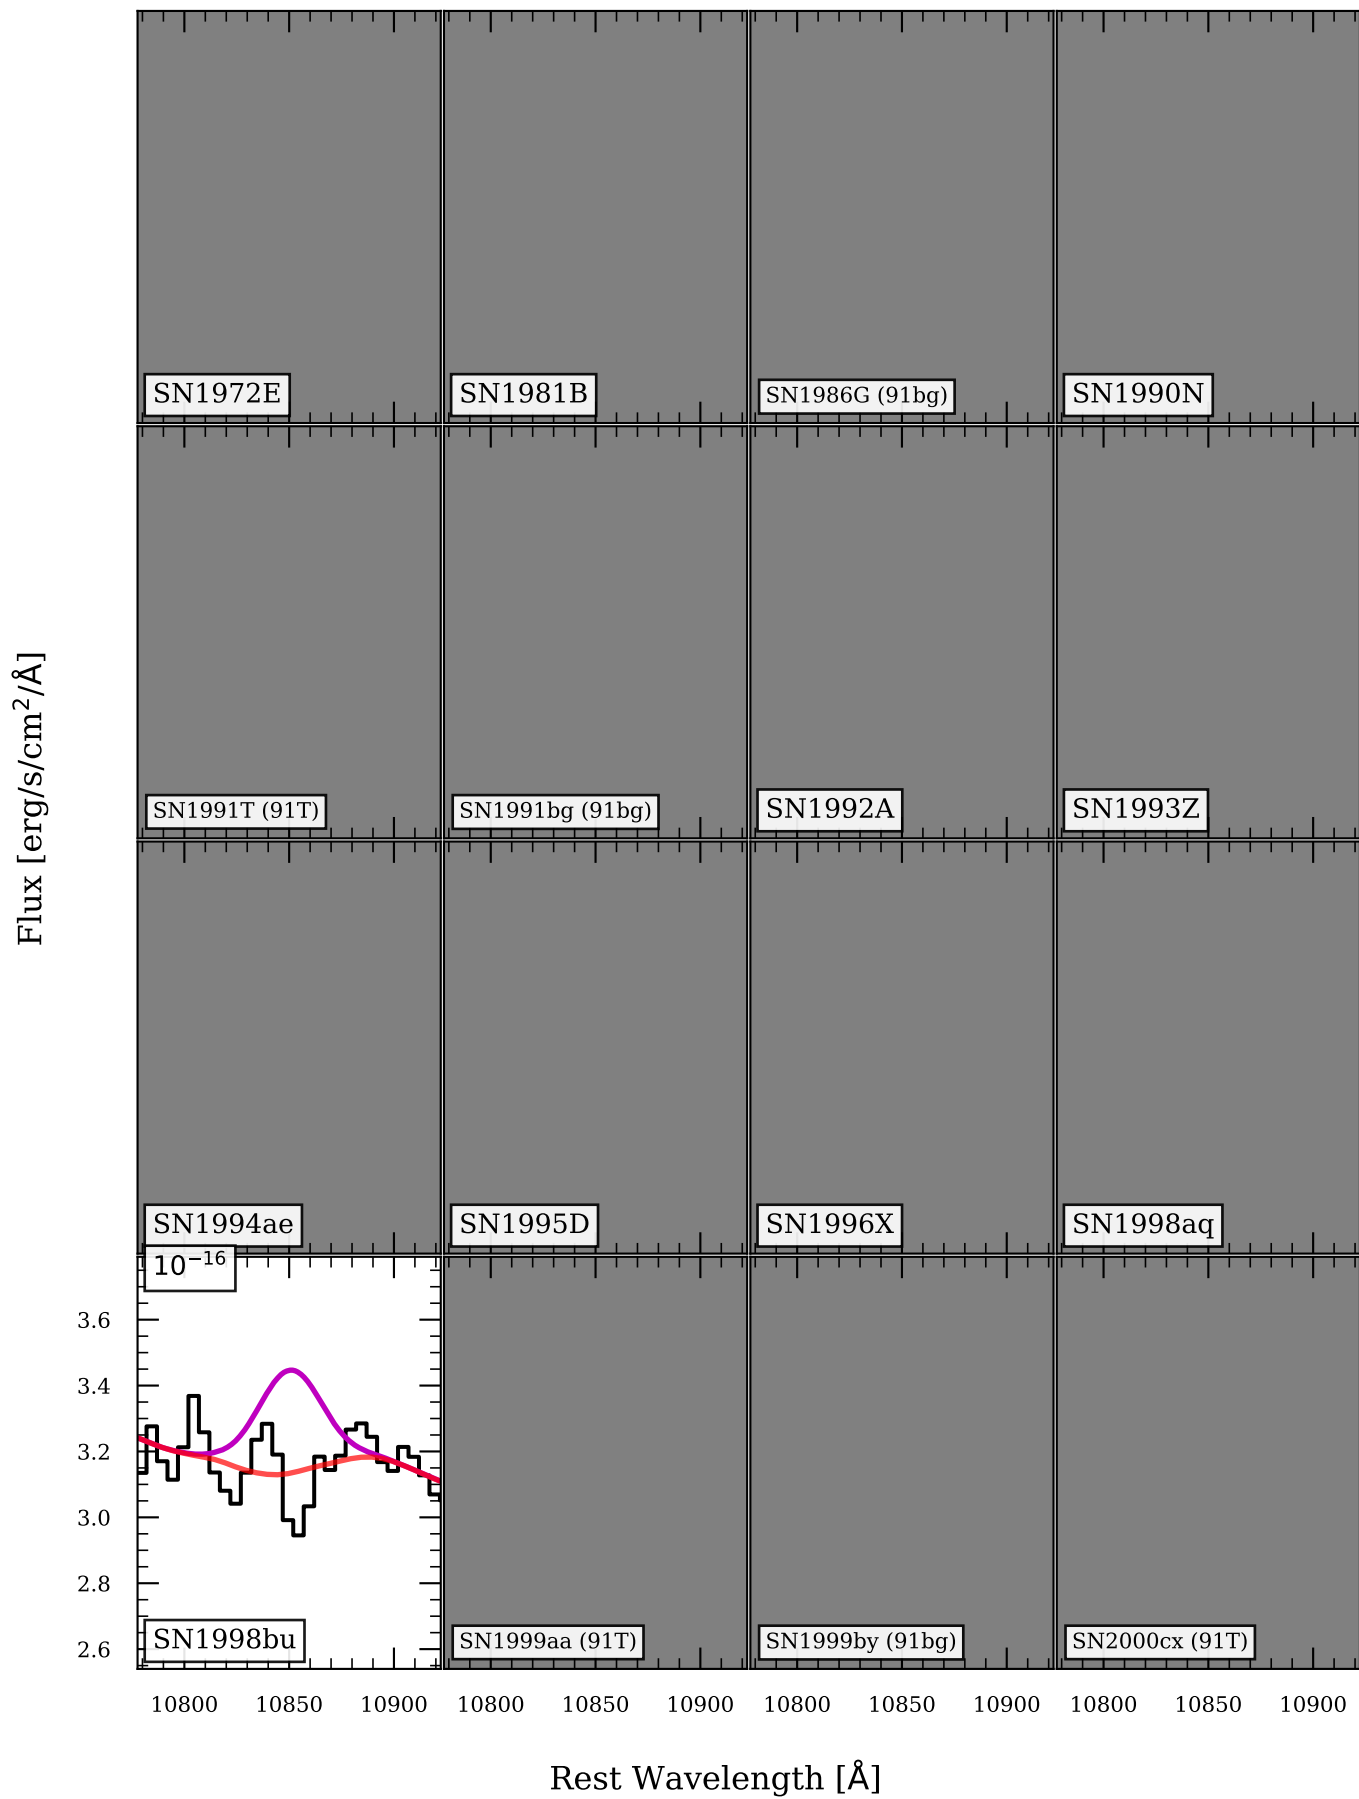

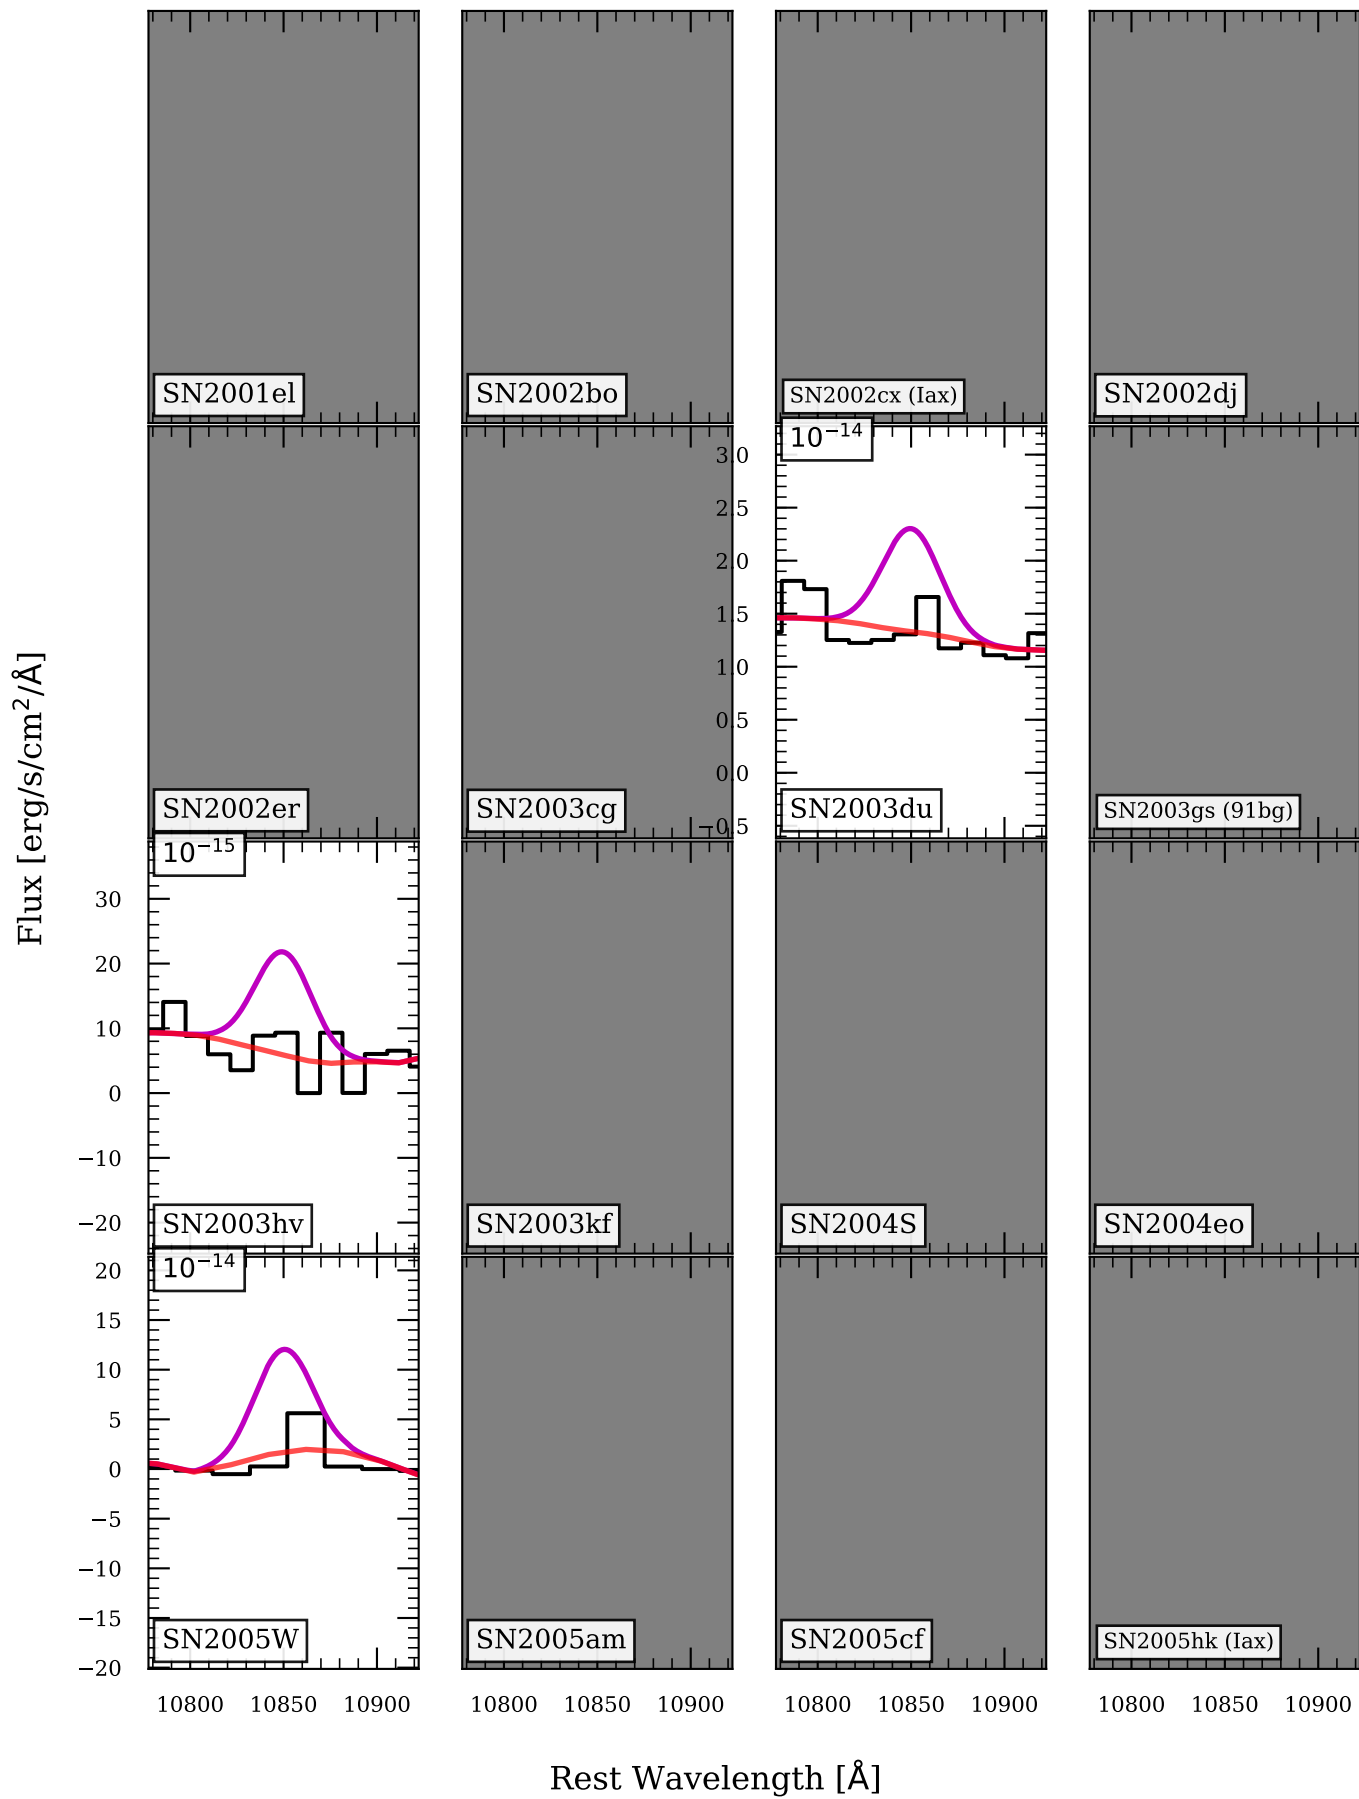

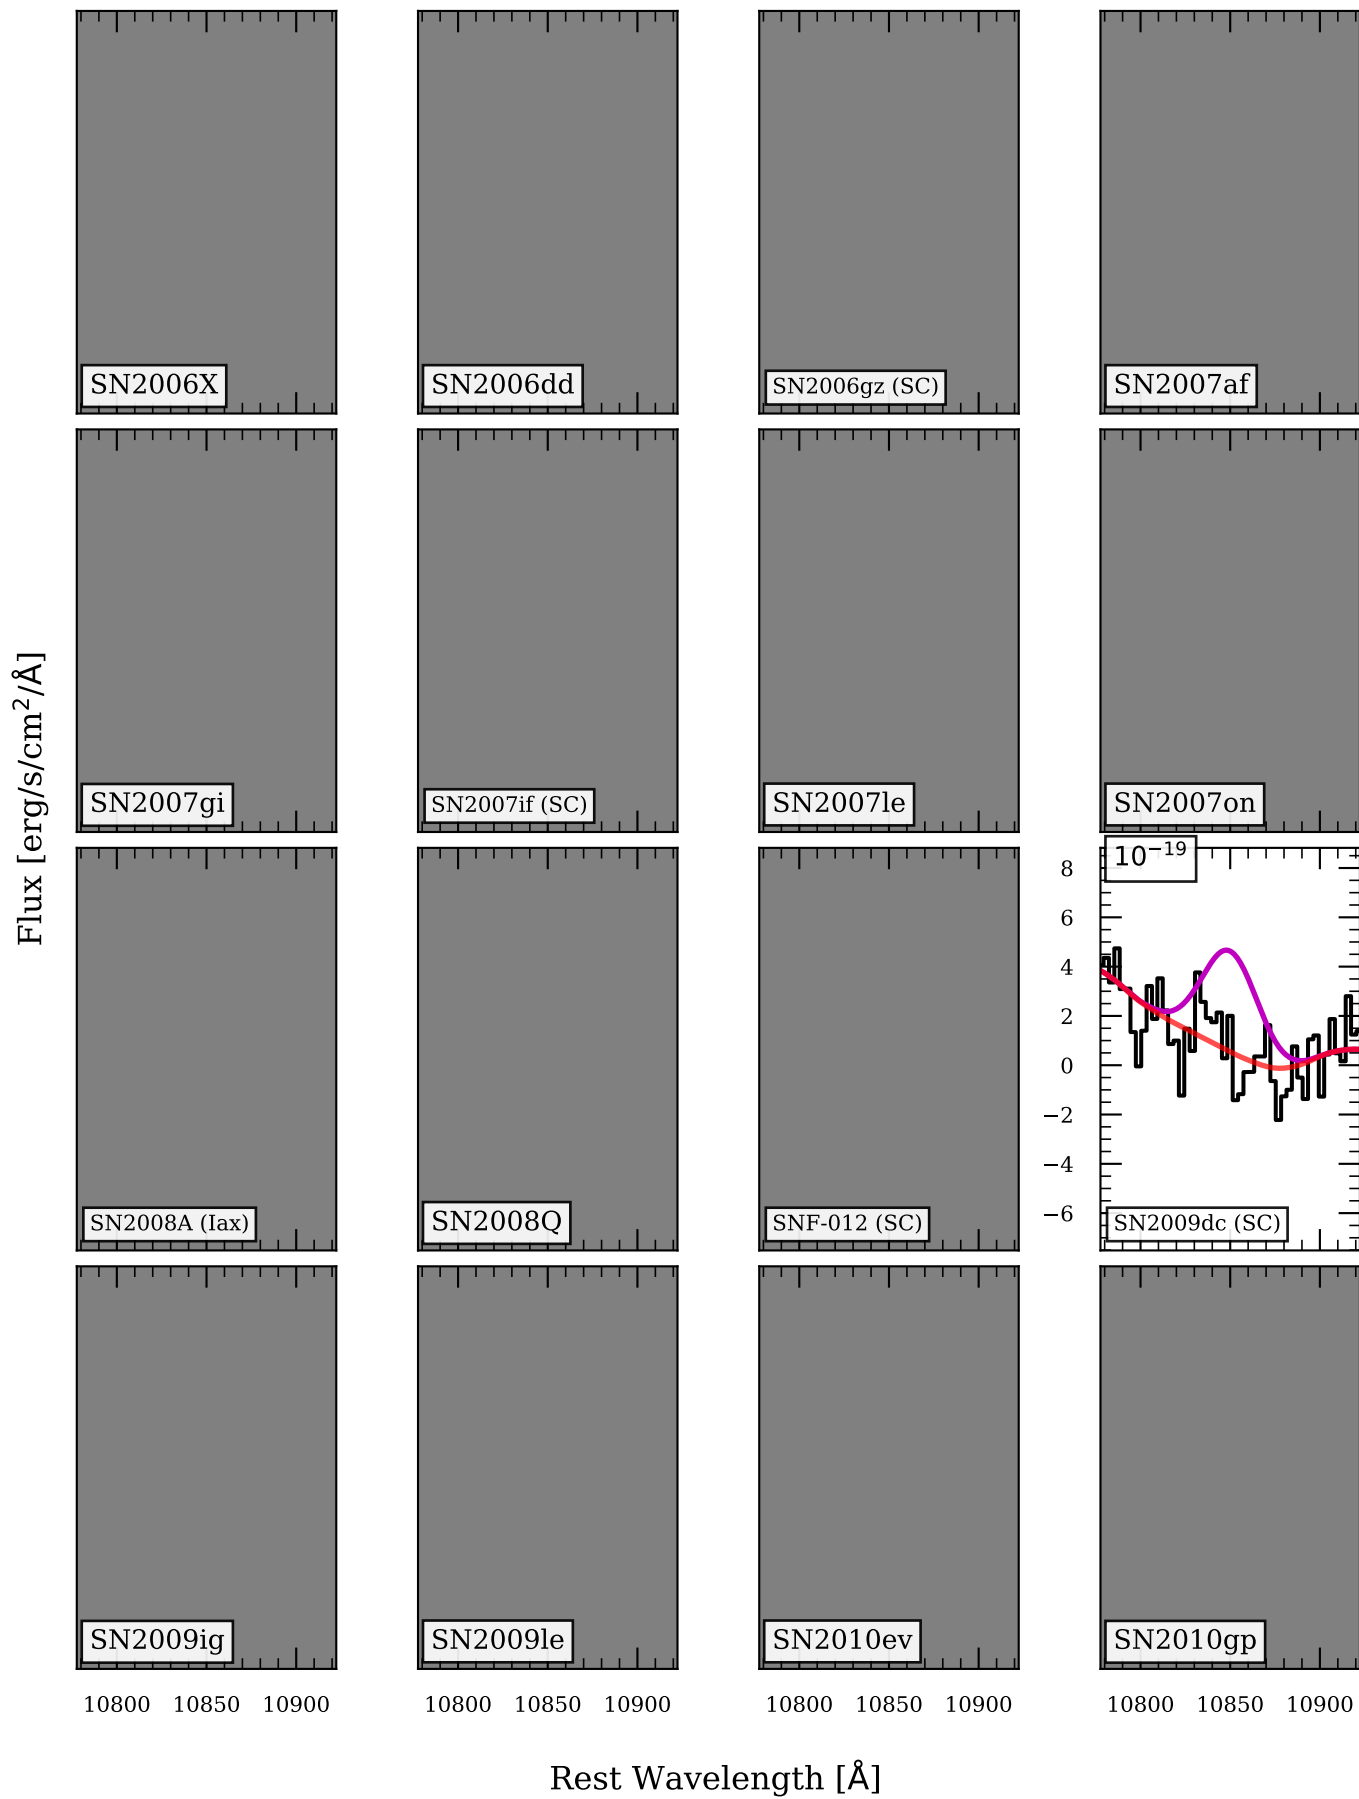

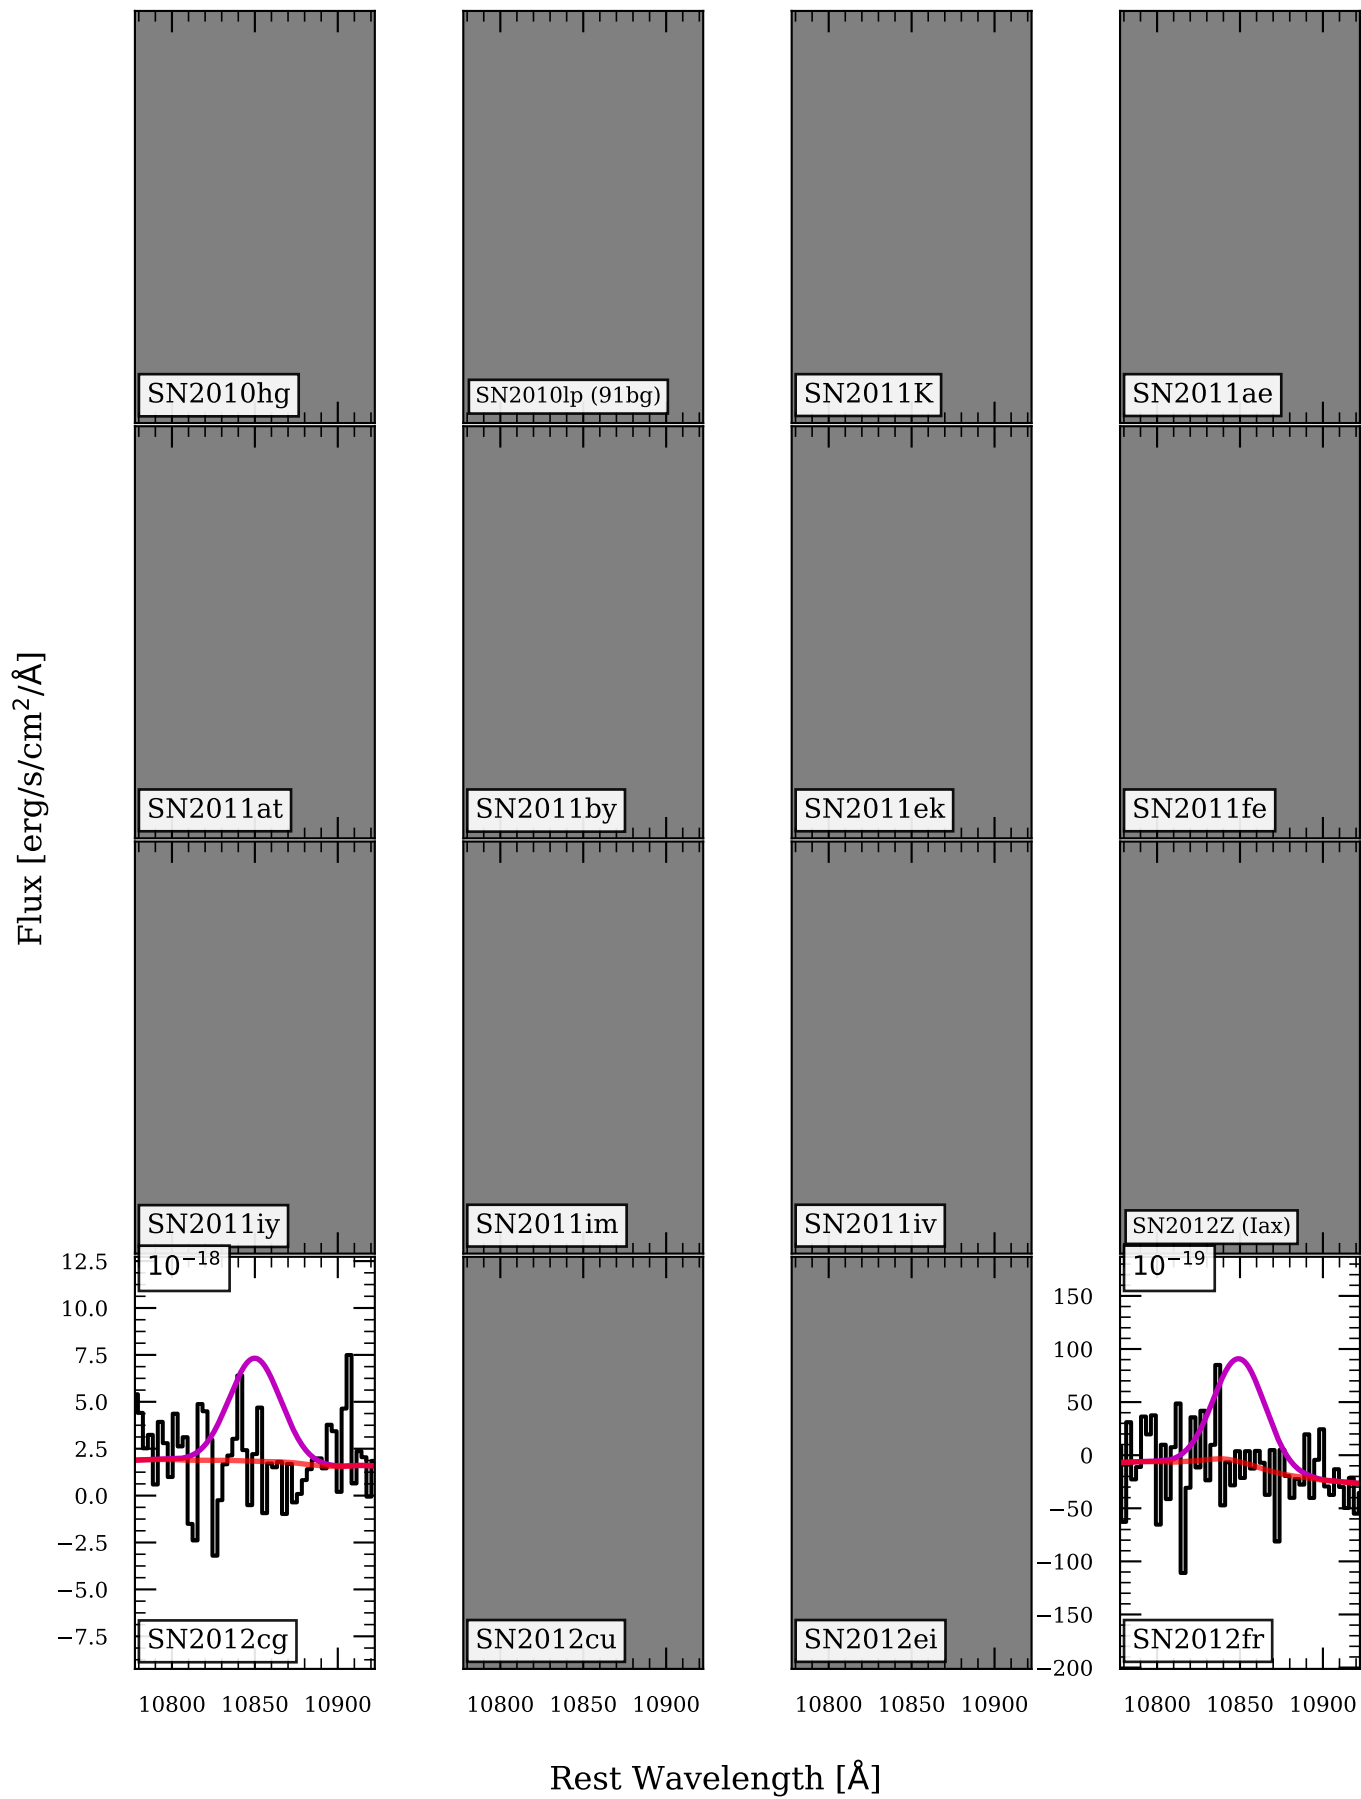

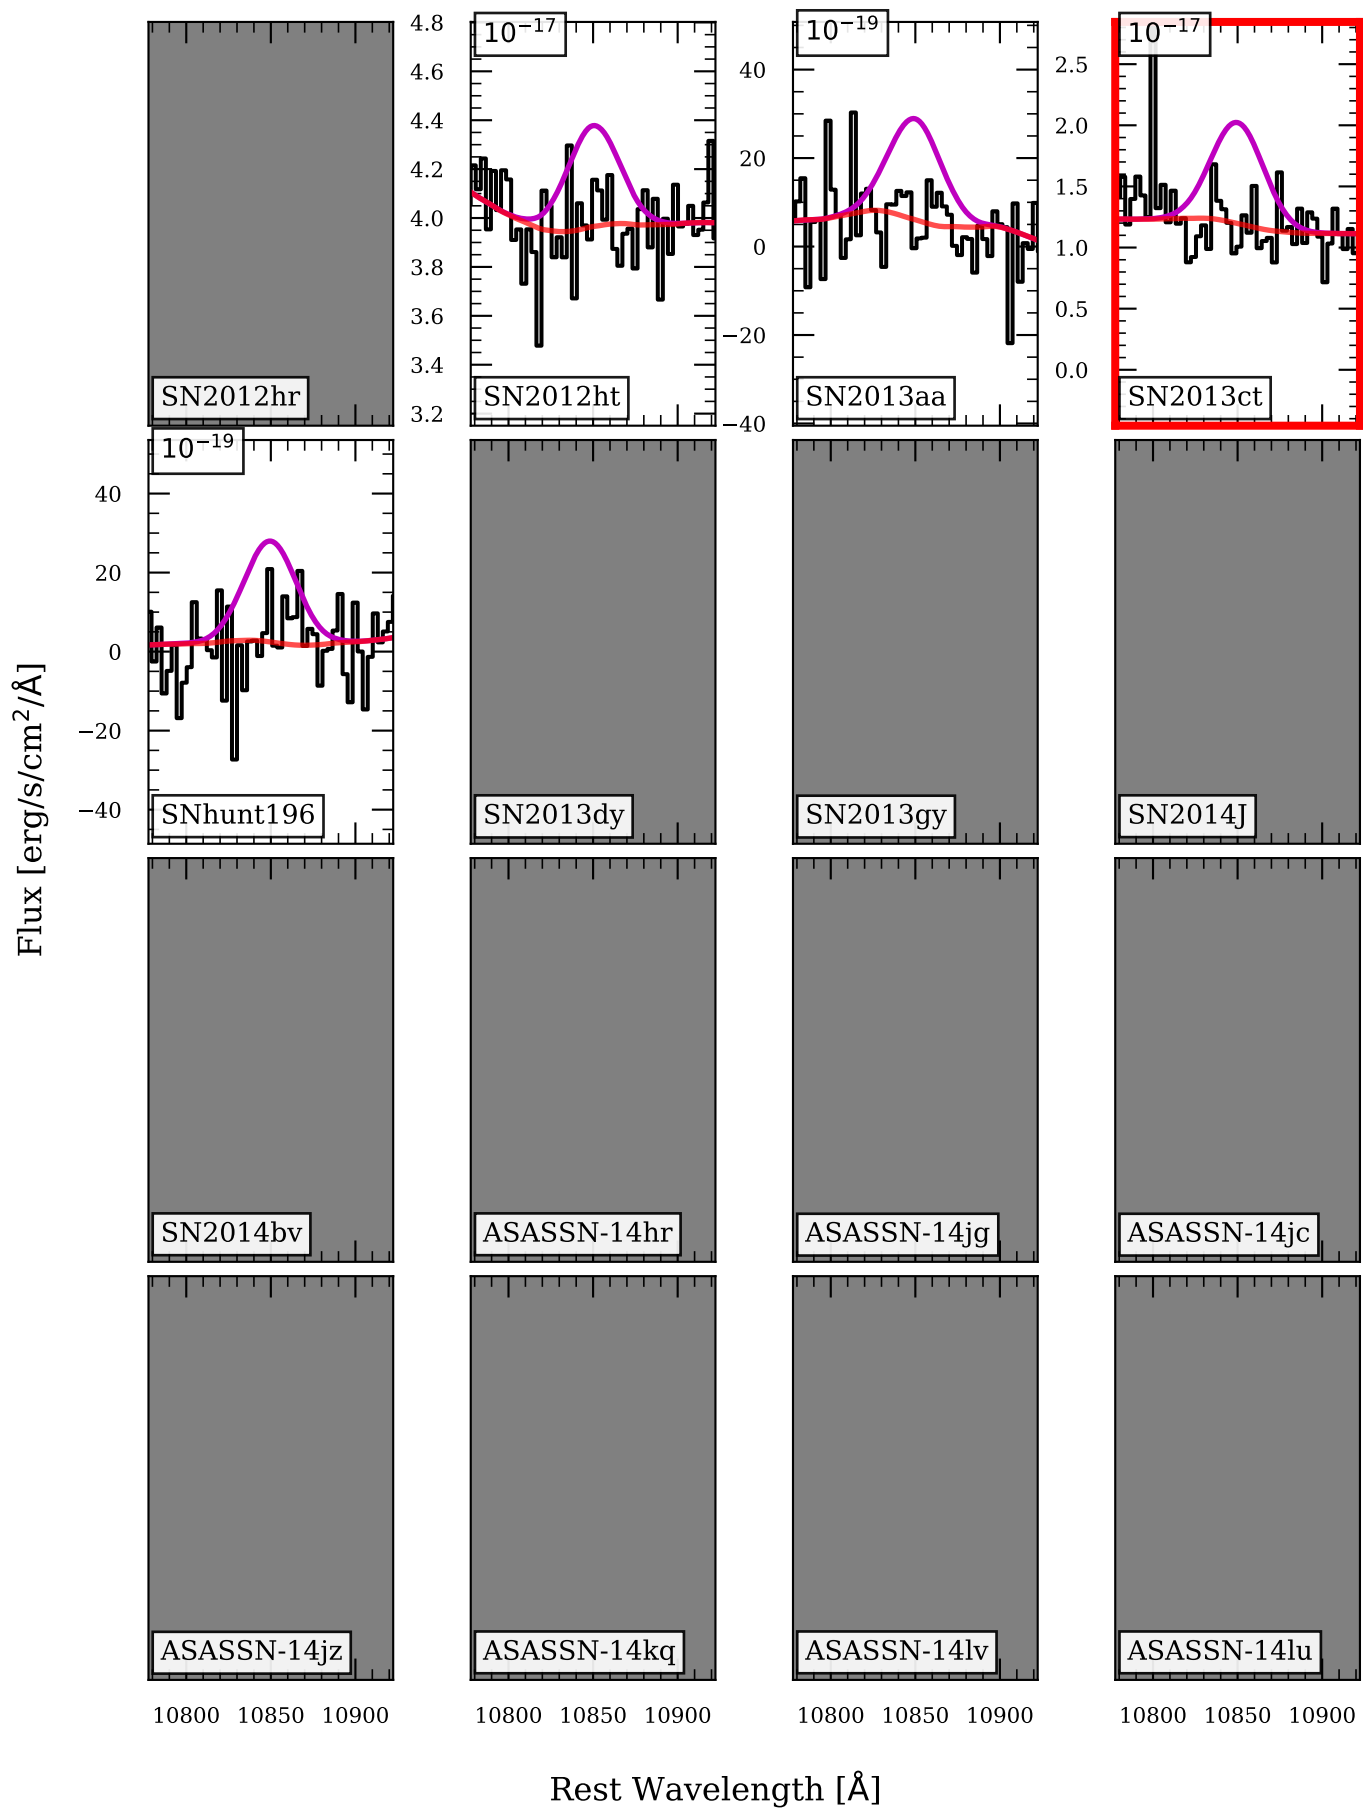

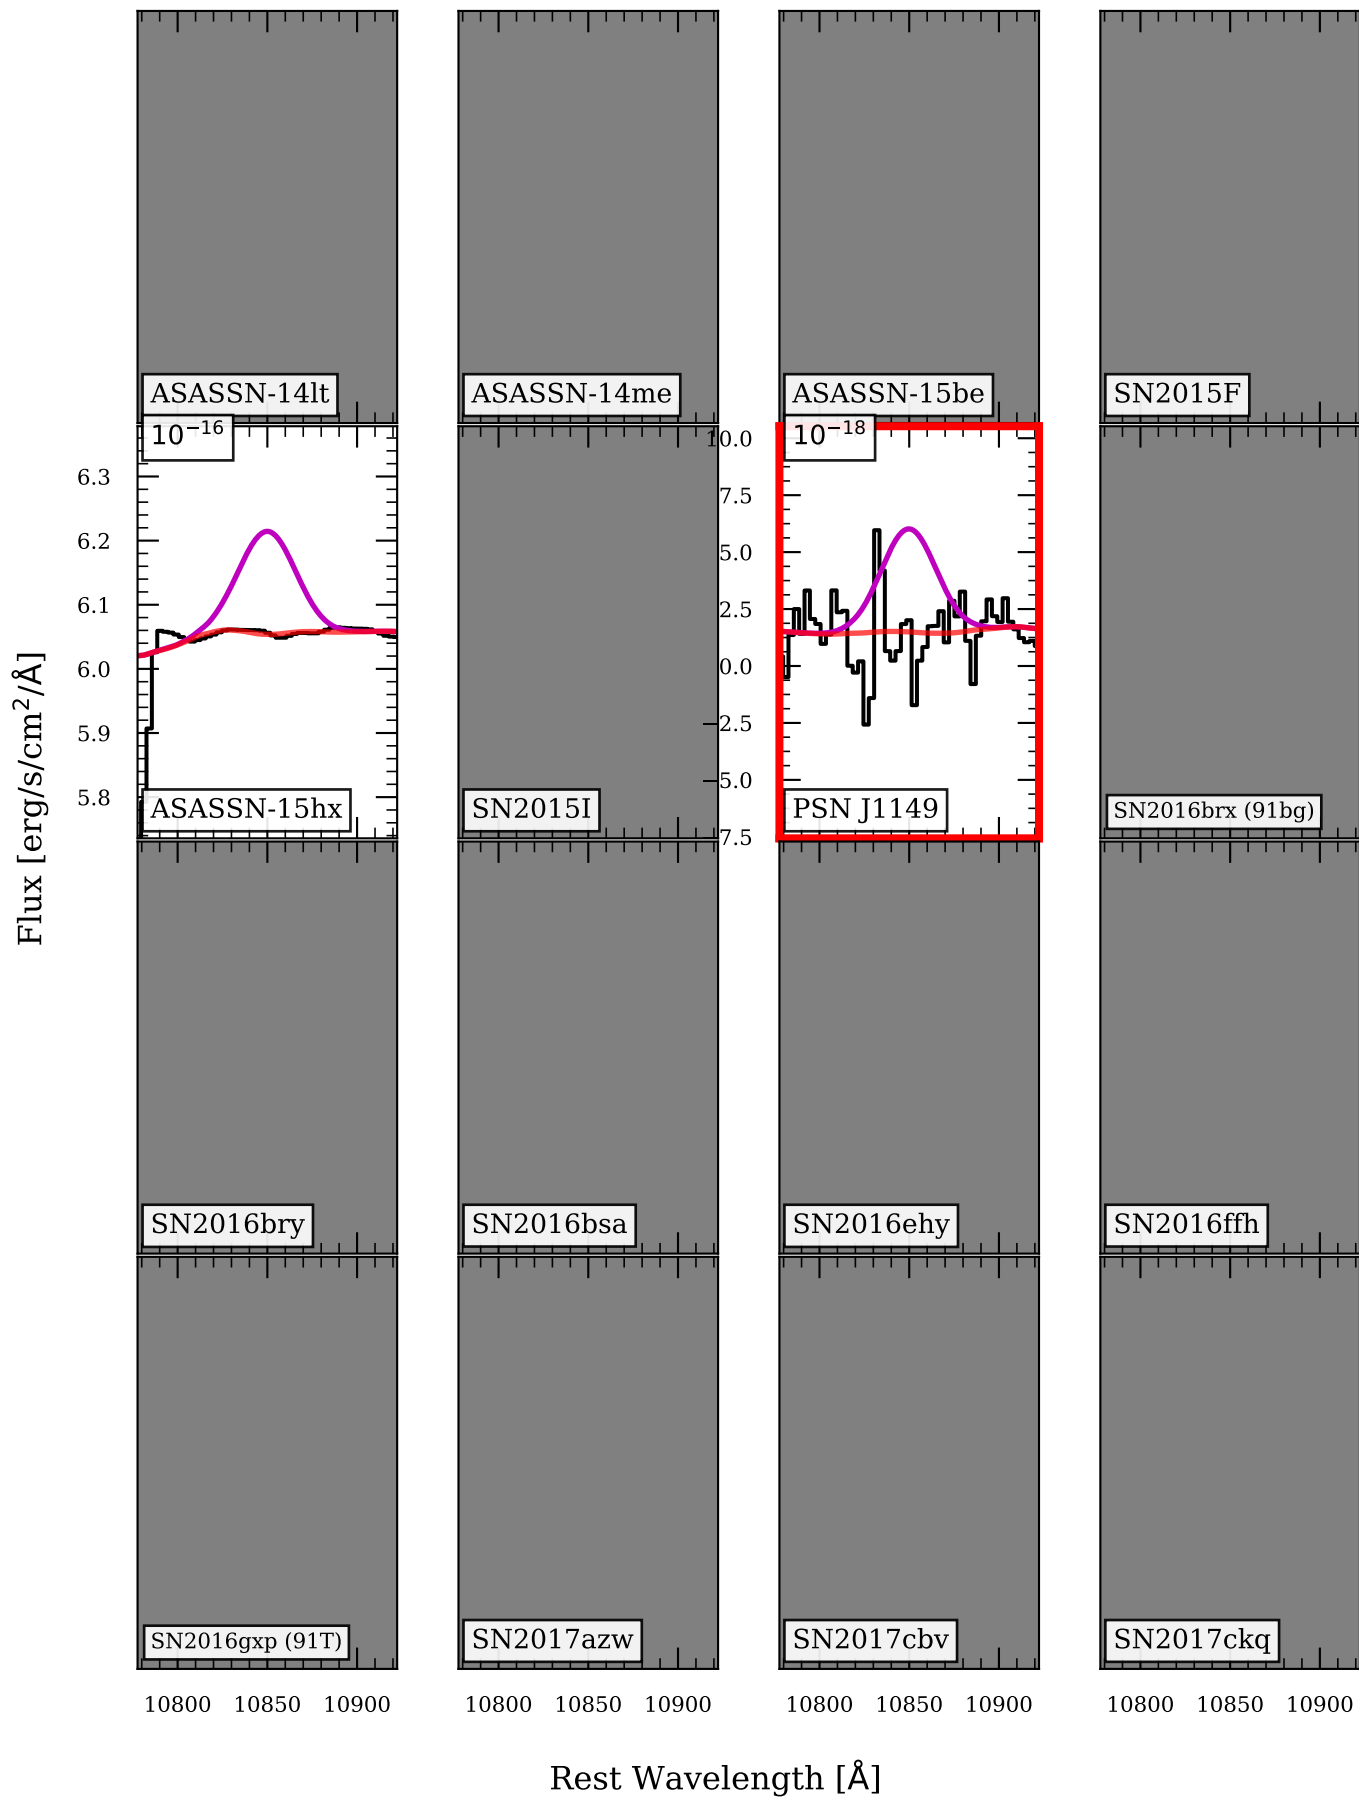

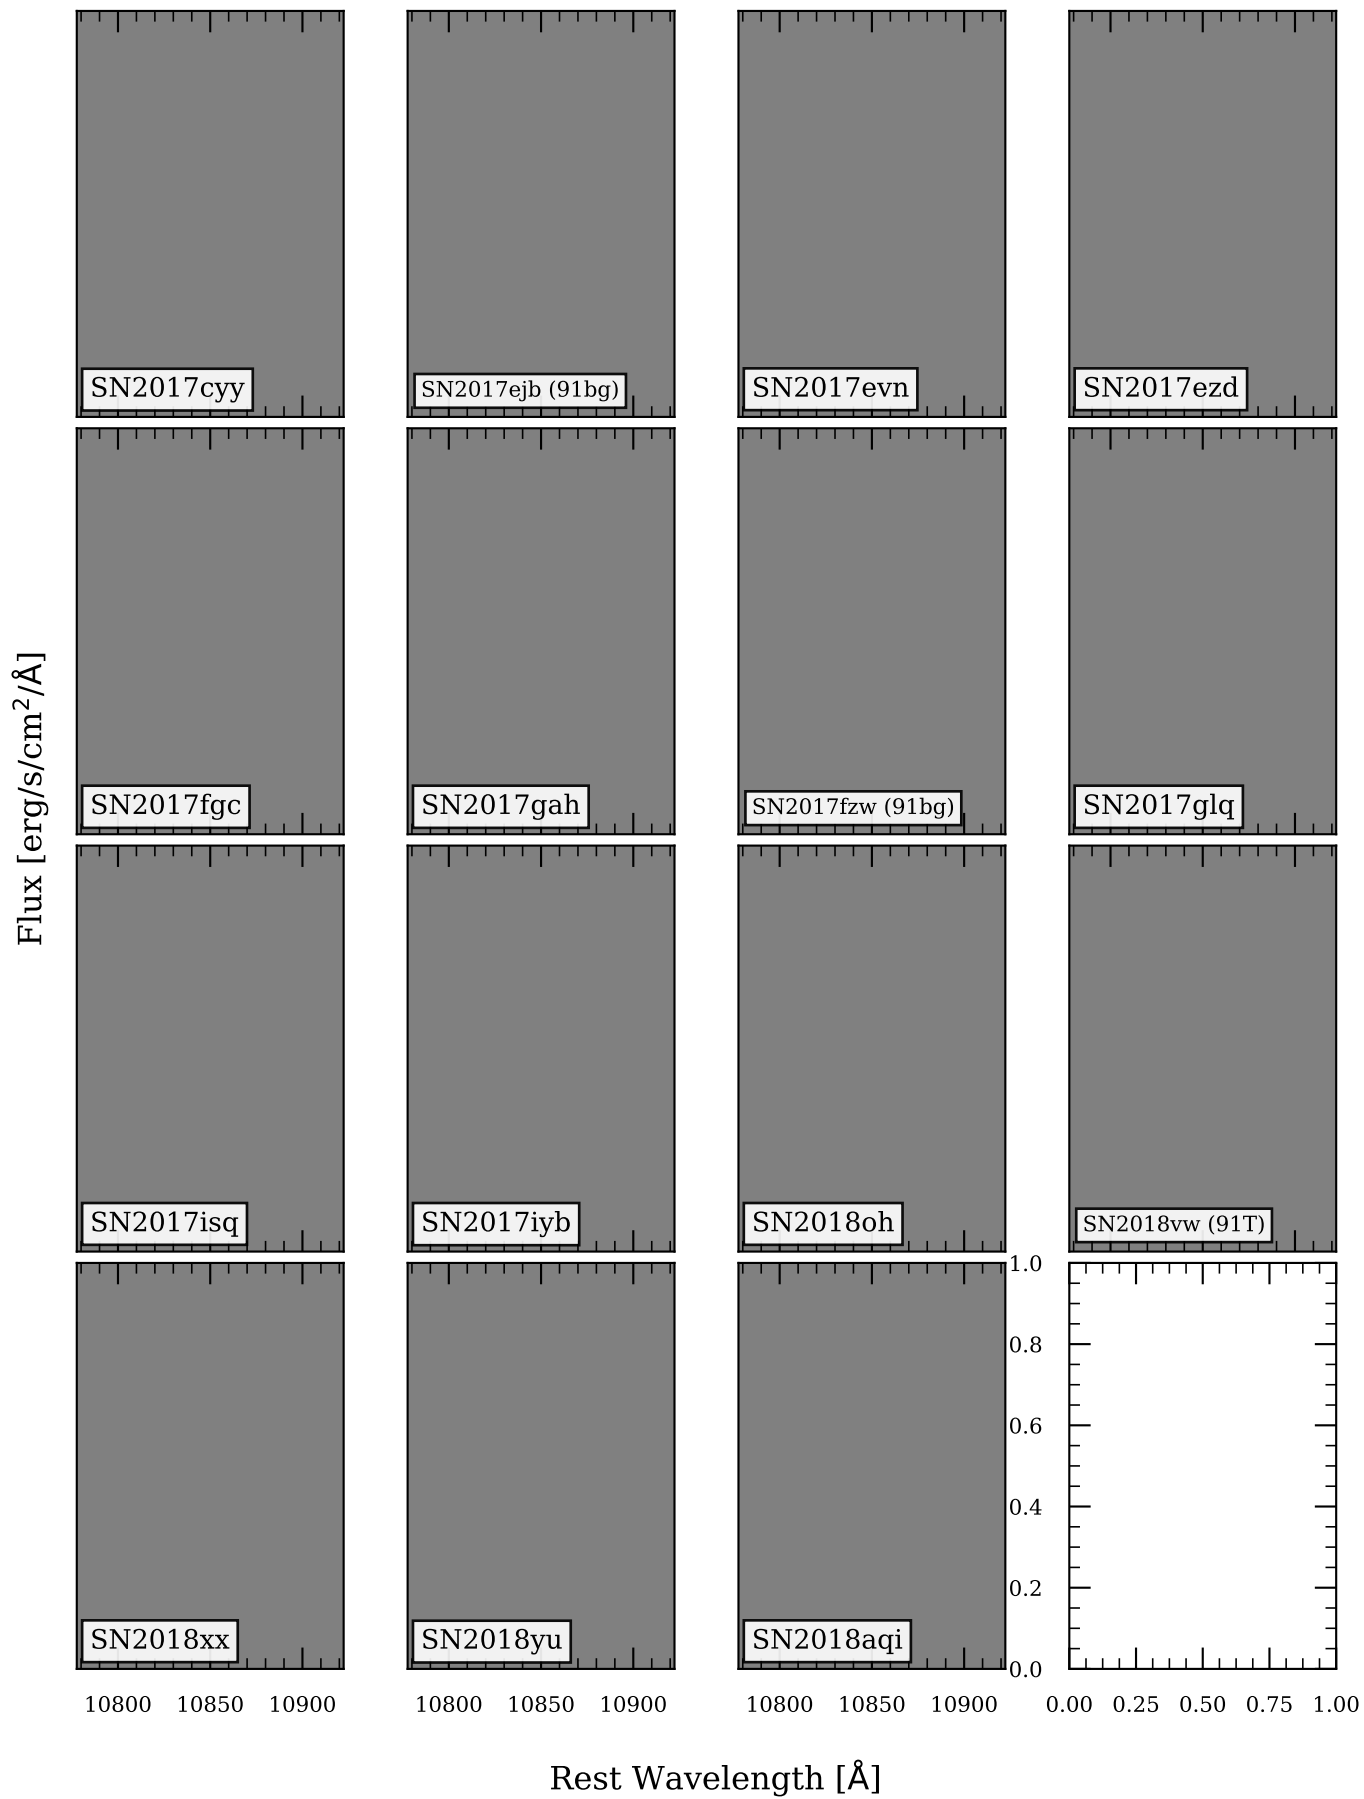

Supplement: Supplementary file 5 [file HeIc-final.pdf]
