# Supplementary material for: Nebular Spectra of 111 Type Ia Supernovae Disfavor Single Degenerate Progenitors
Source: arXiv:1903.05115 ancillary file (2019-10-31)

**Hel-d  
20590 Å**

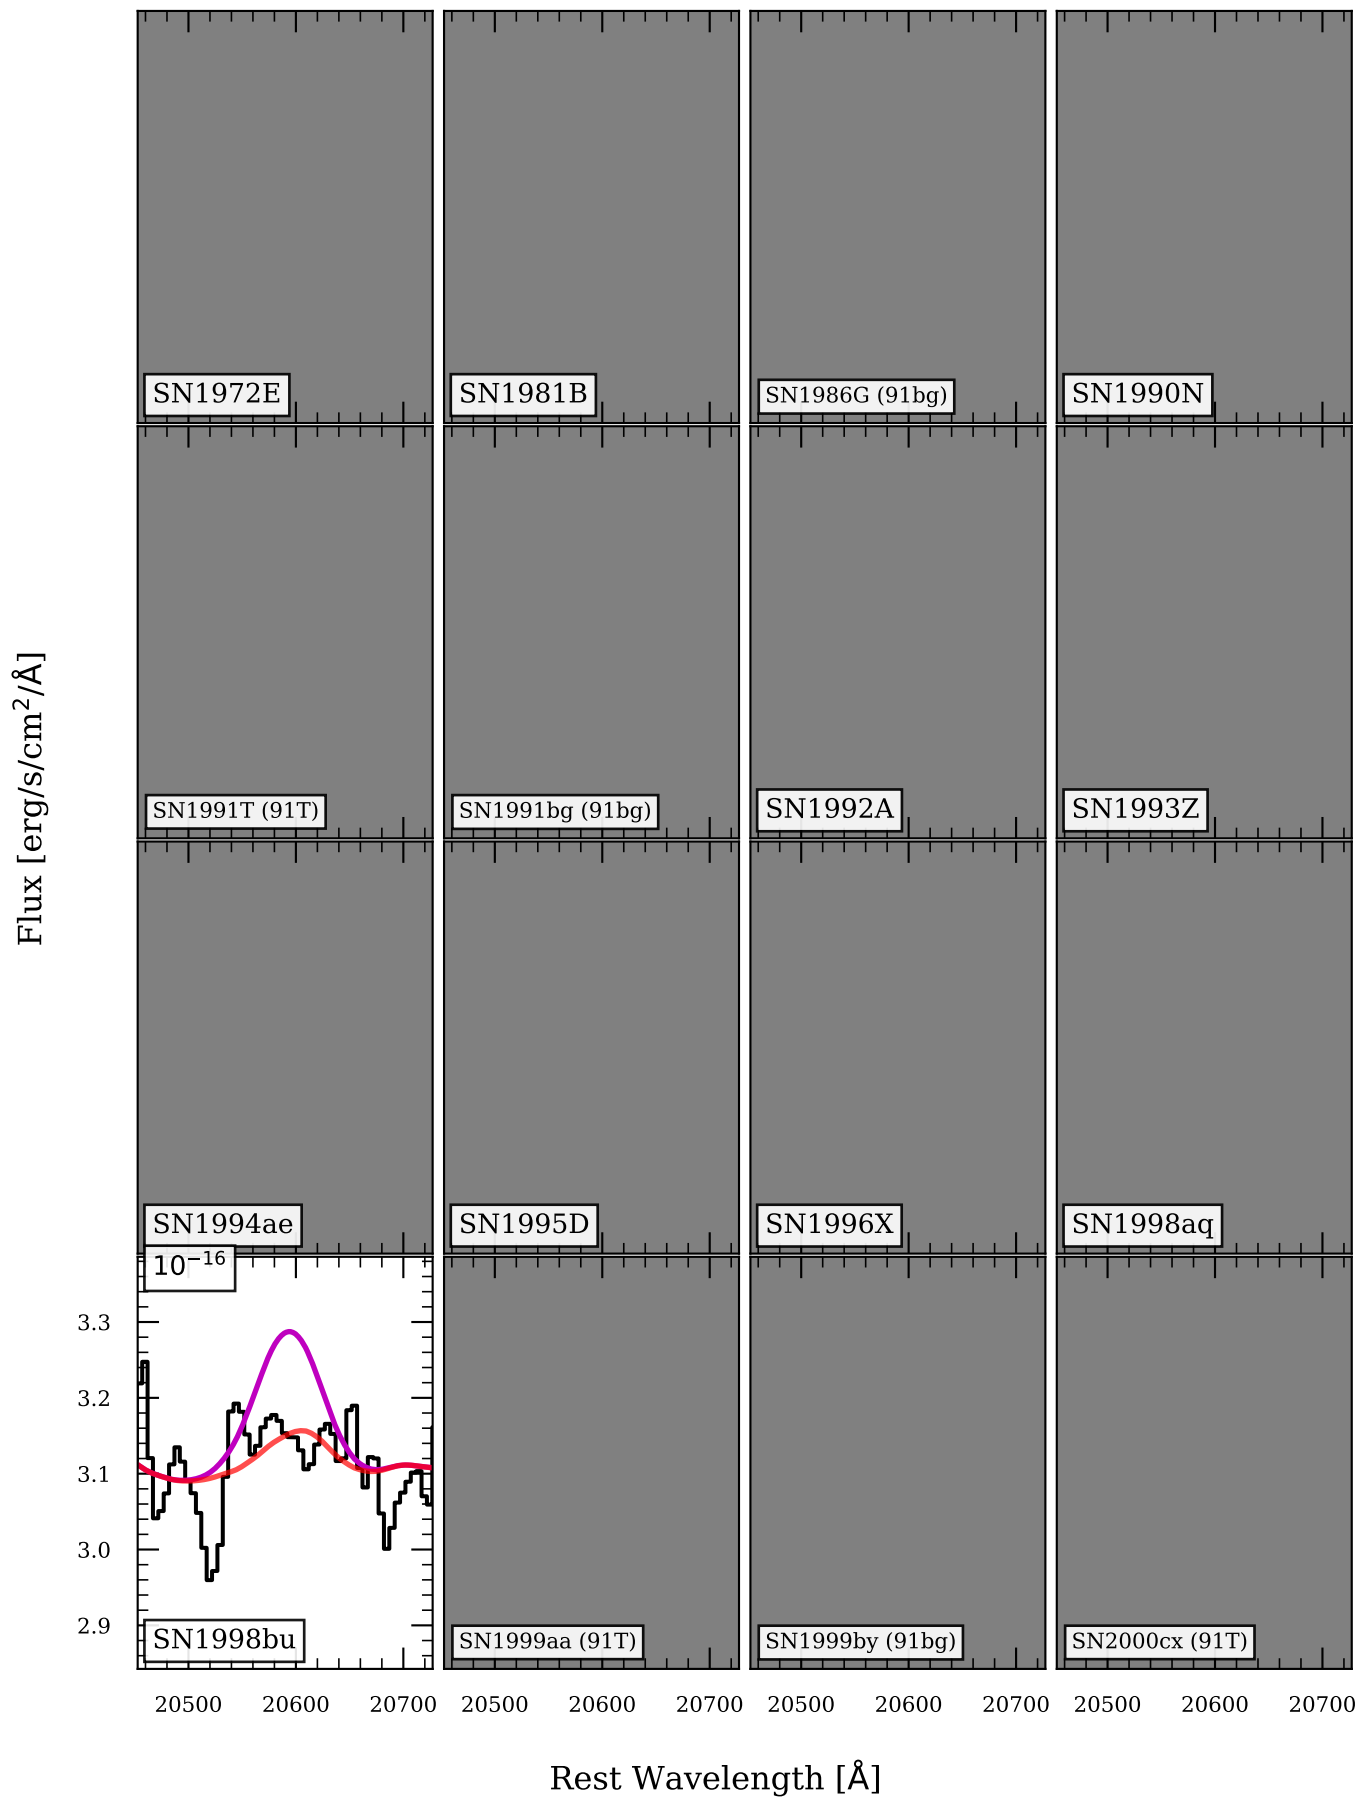

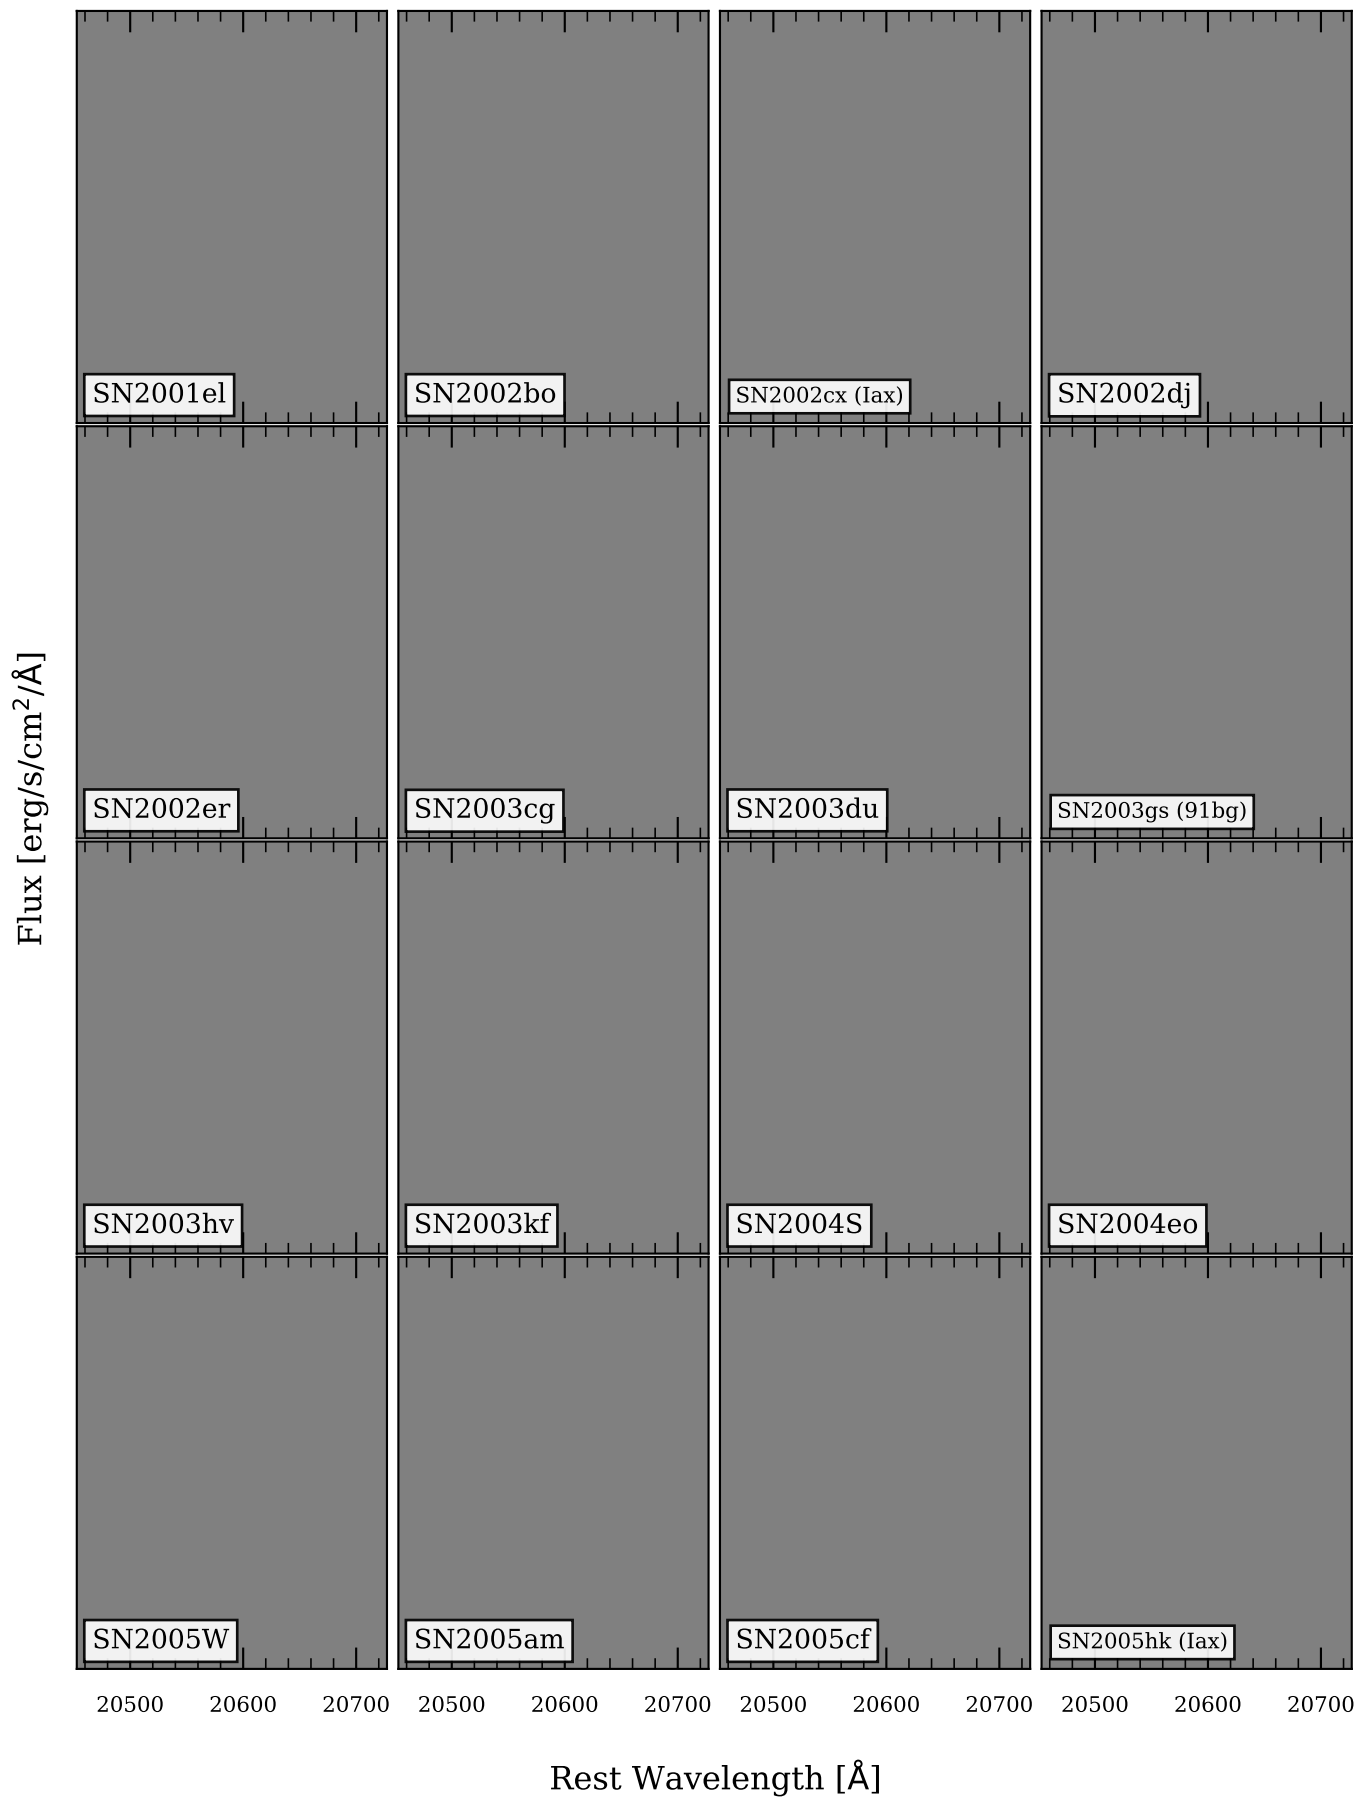

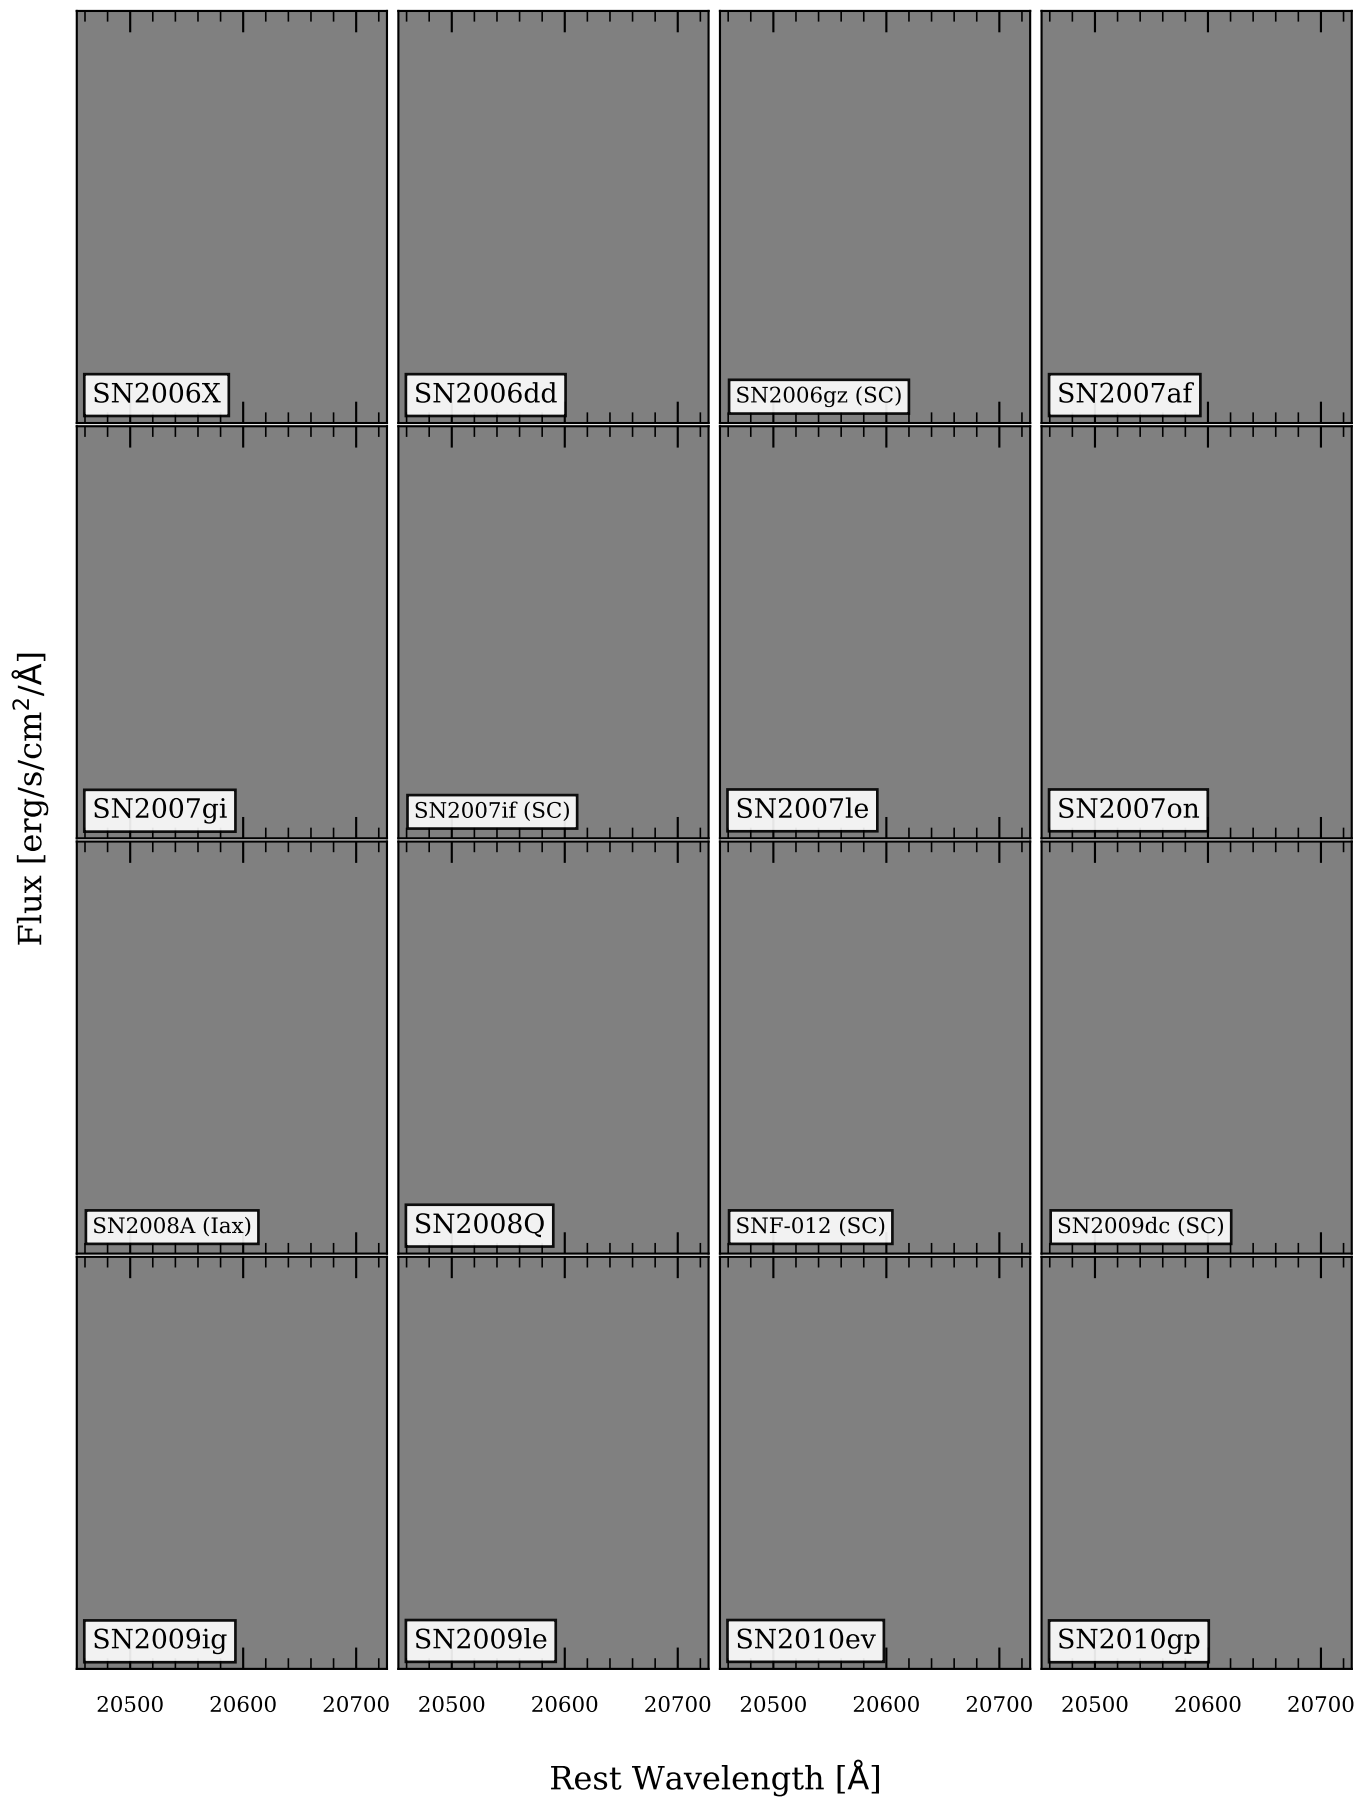

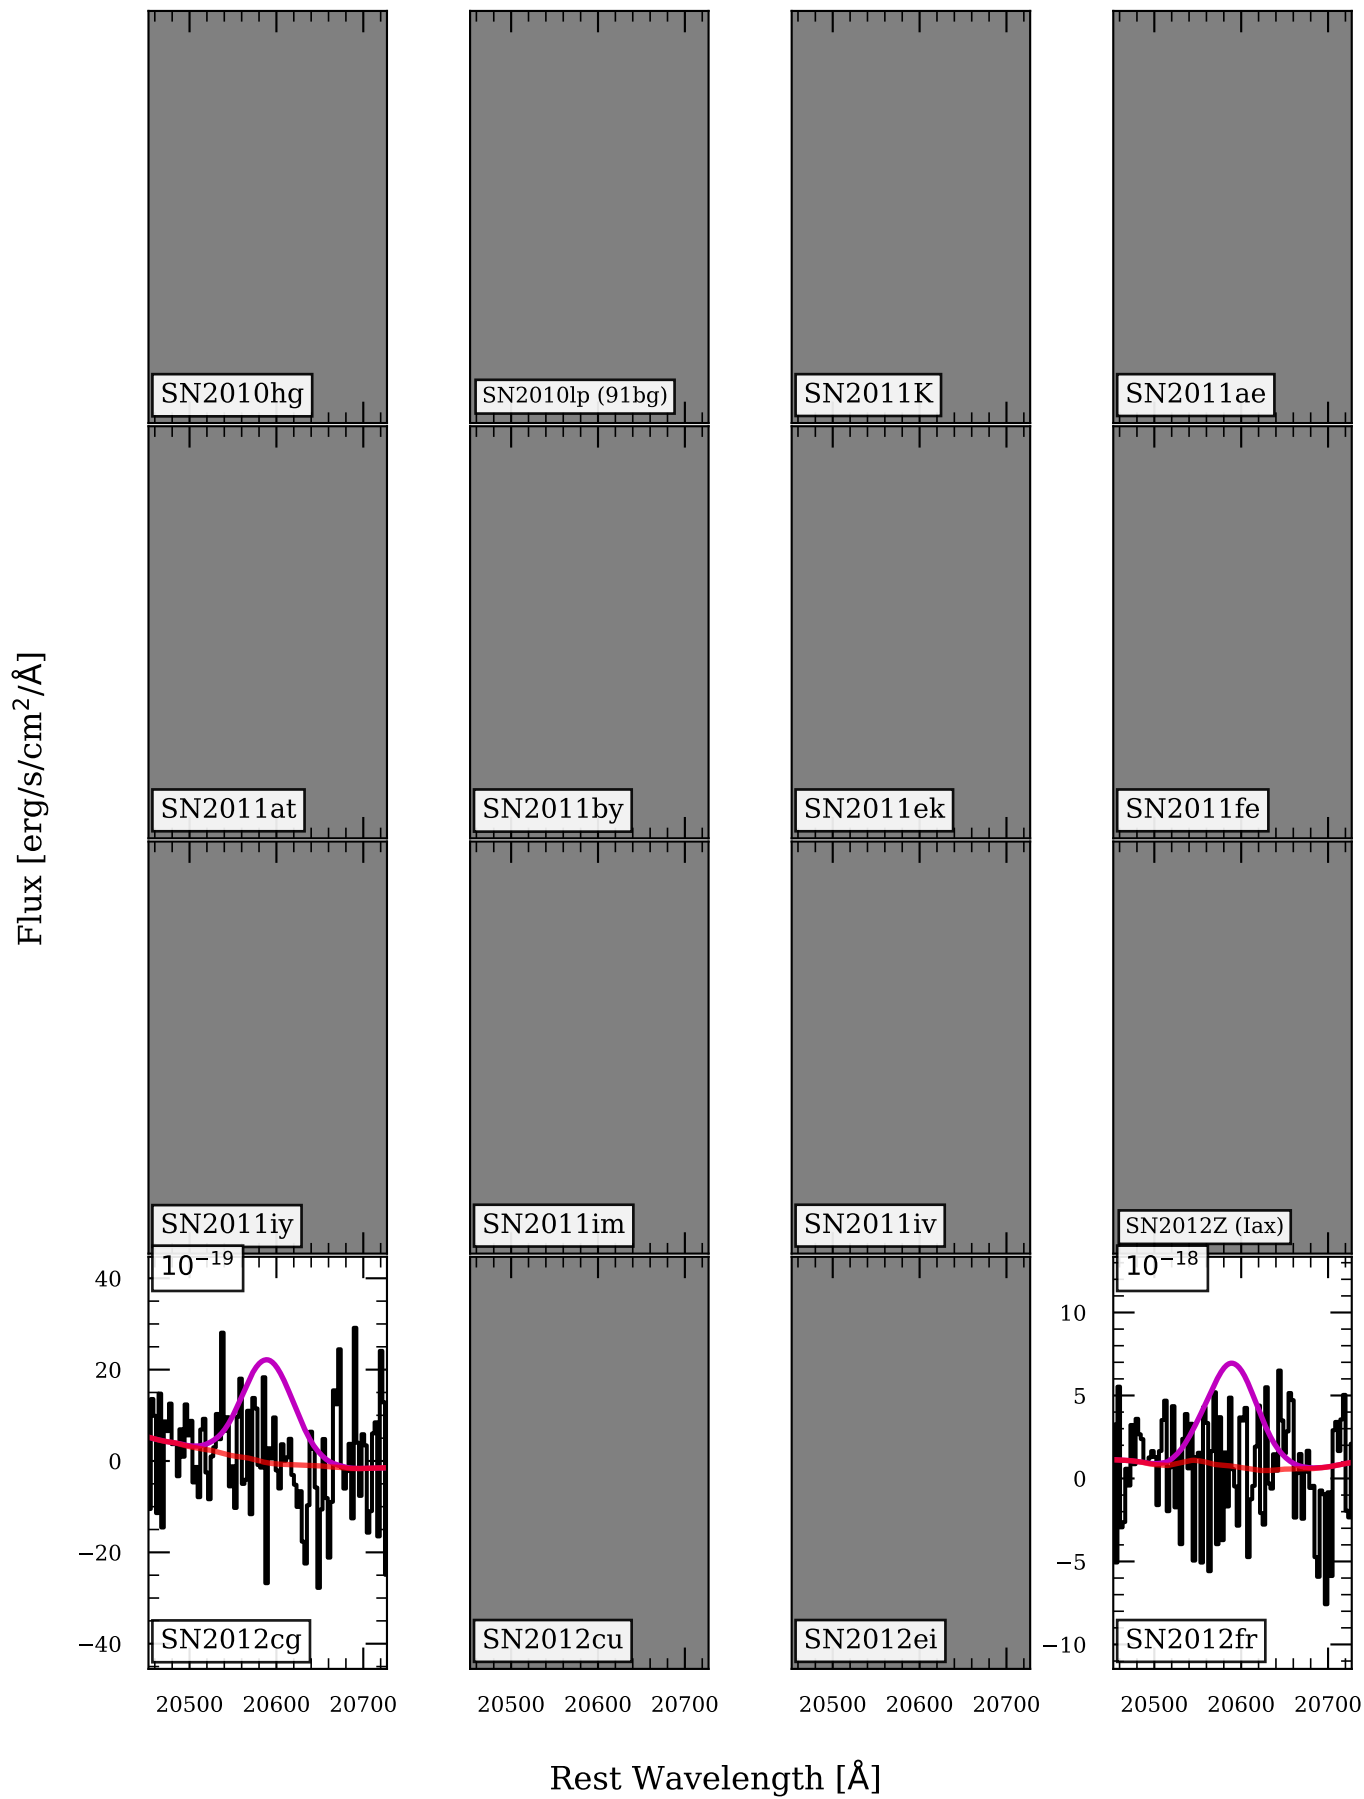

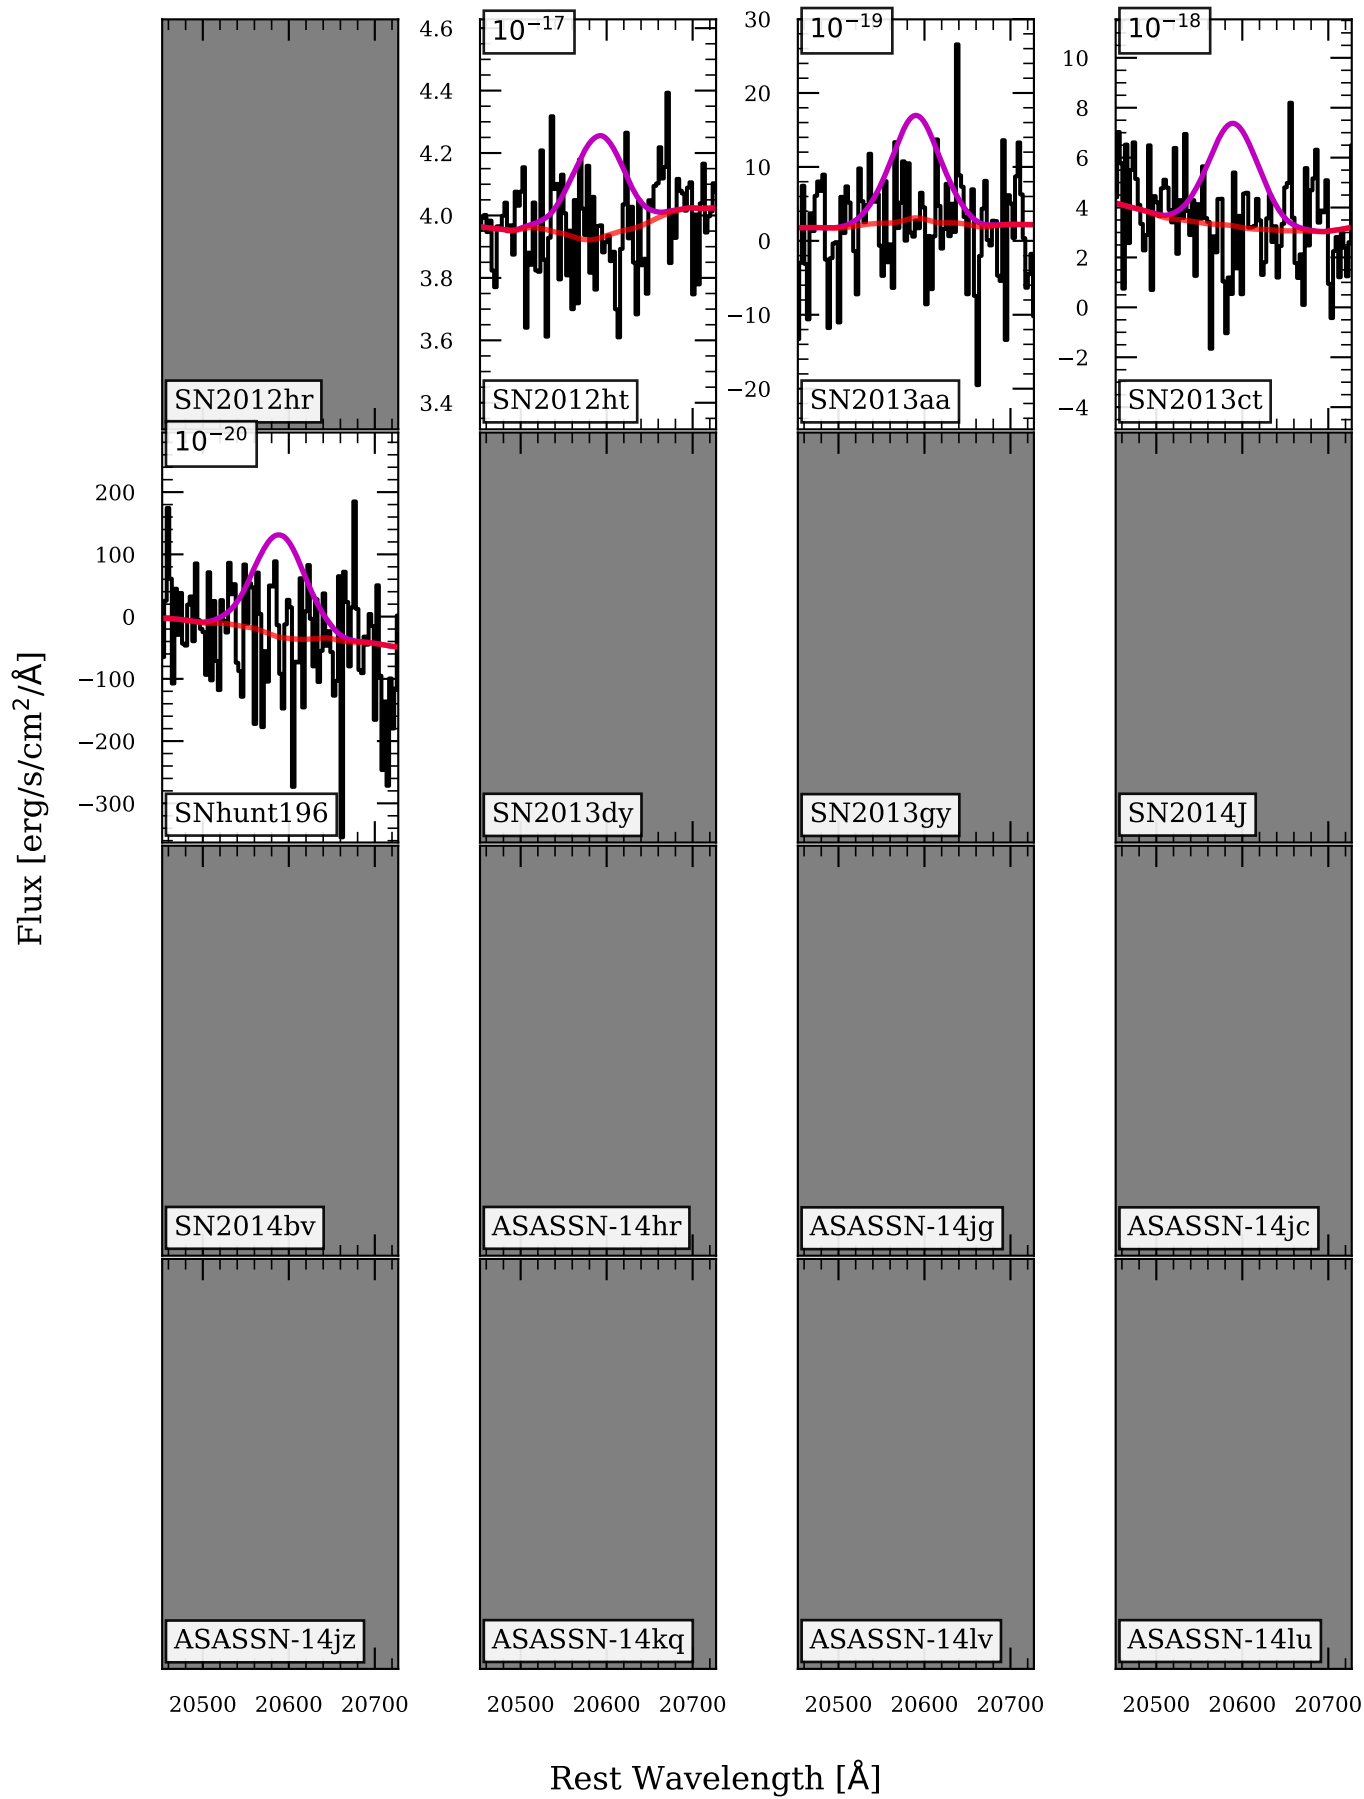

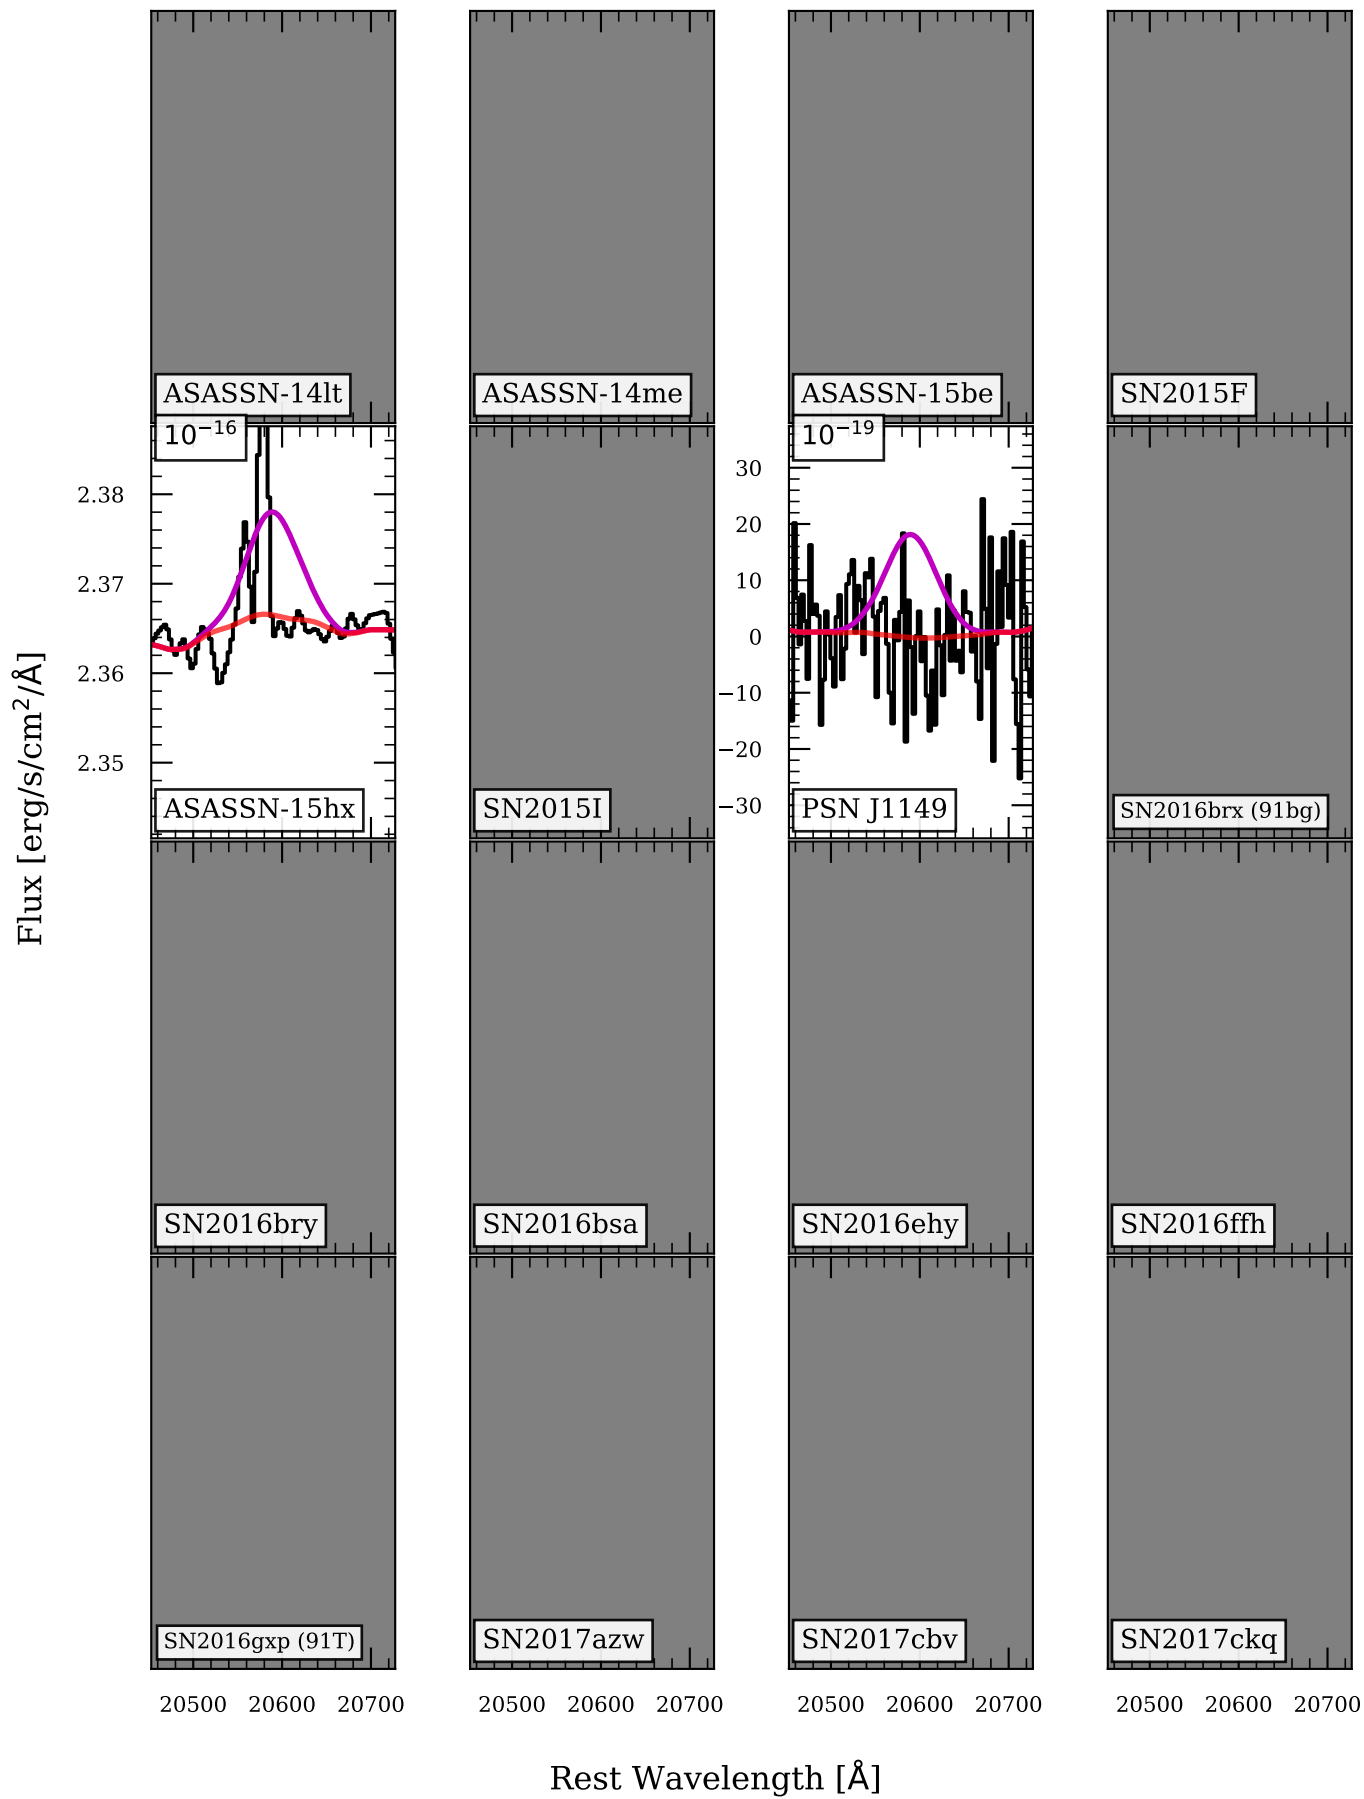

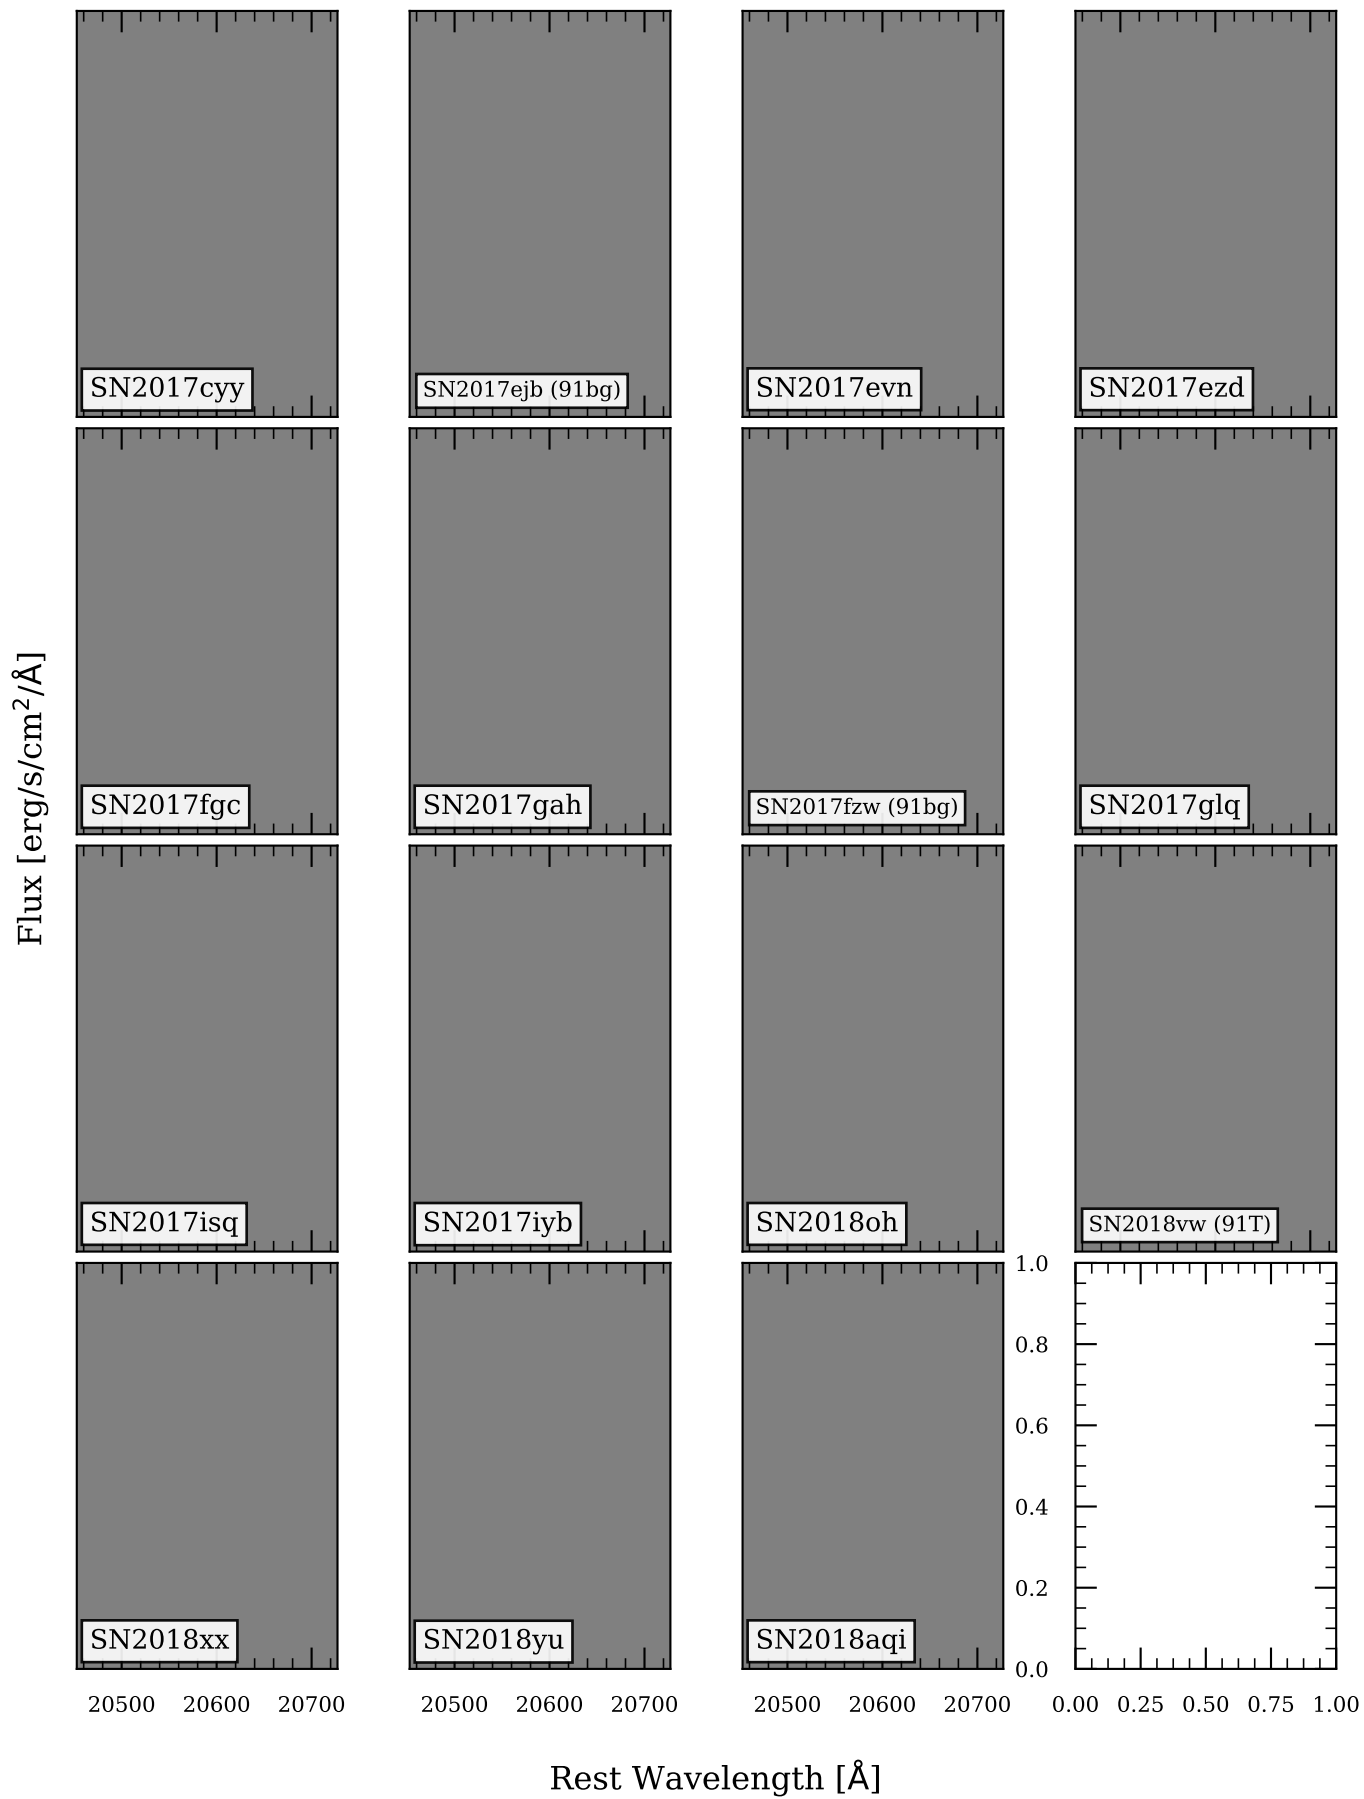

Supplement: Supplementary file 6 [file HeId-final.pdf]
