# Supplementary material for: Nebular Spectra of 111 Type Ia Supernovae Disfavor Single Degenerate Progenitors
Source: arXiv:1903.05115 ancillary file (2019-10-31)

**$\text{Pa}$**

**18750 Å**

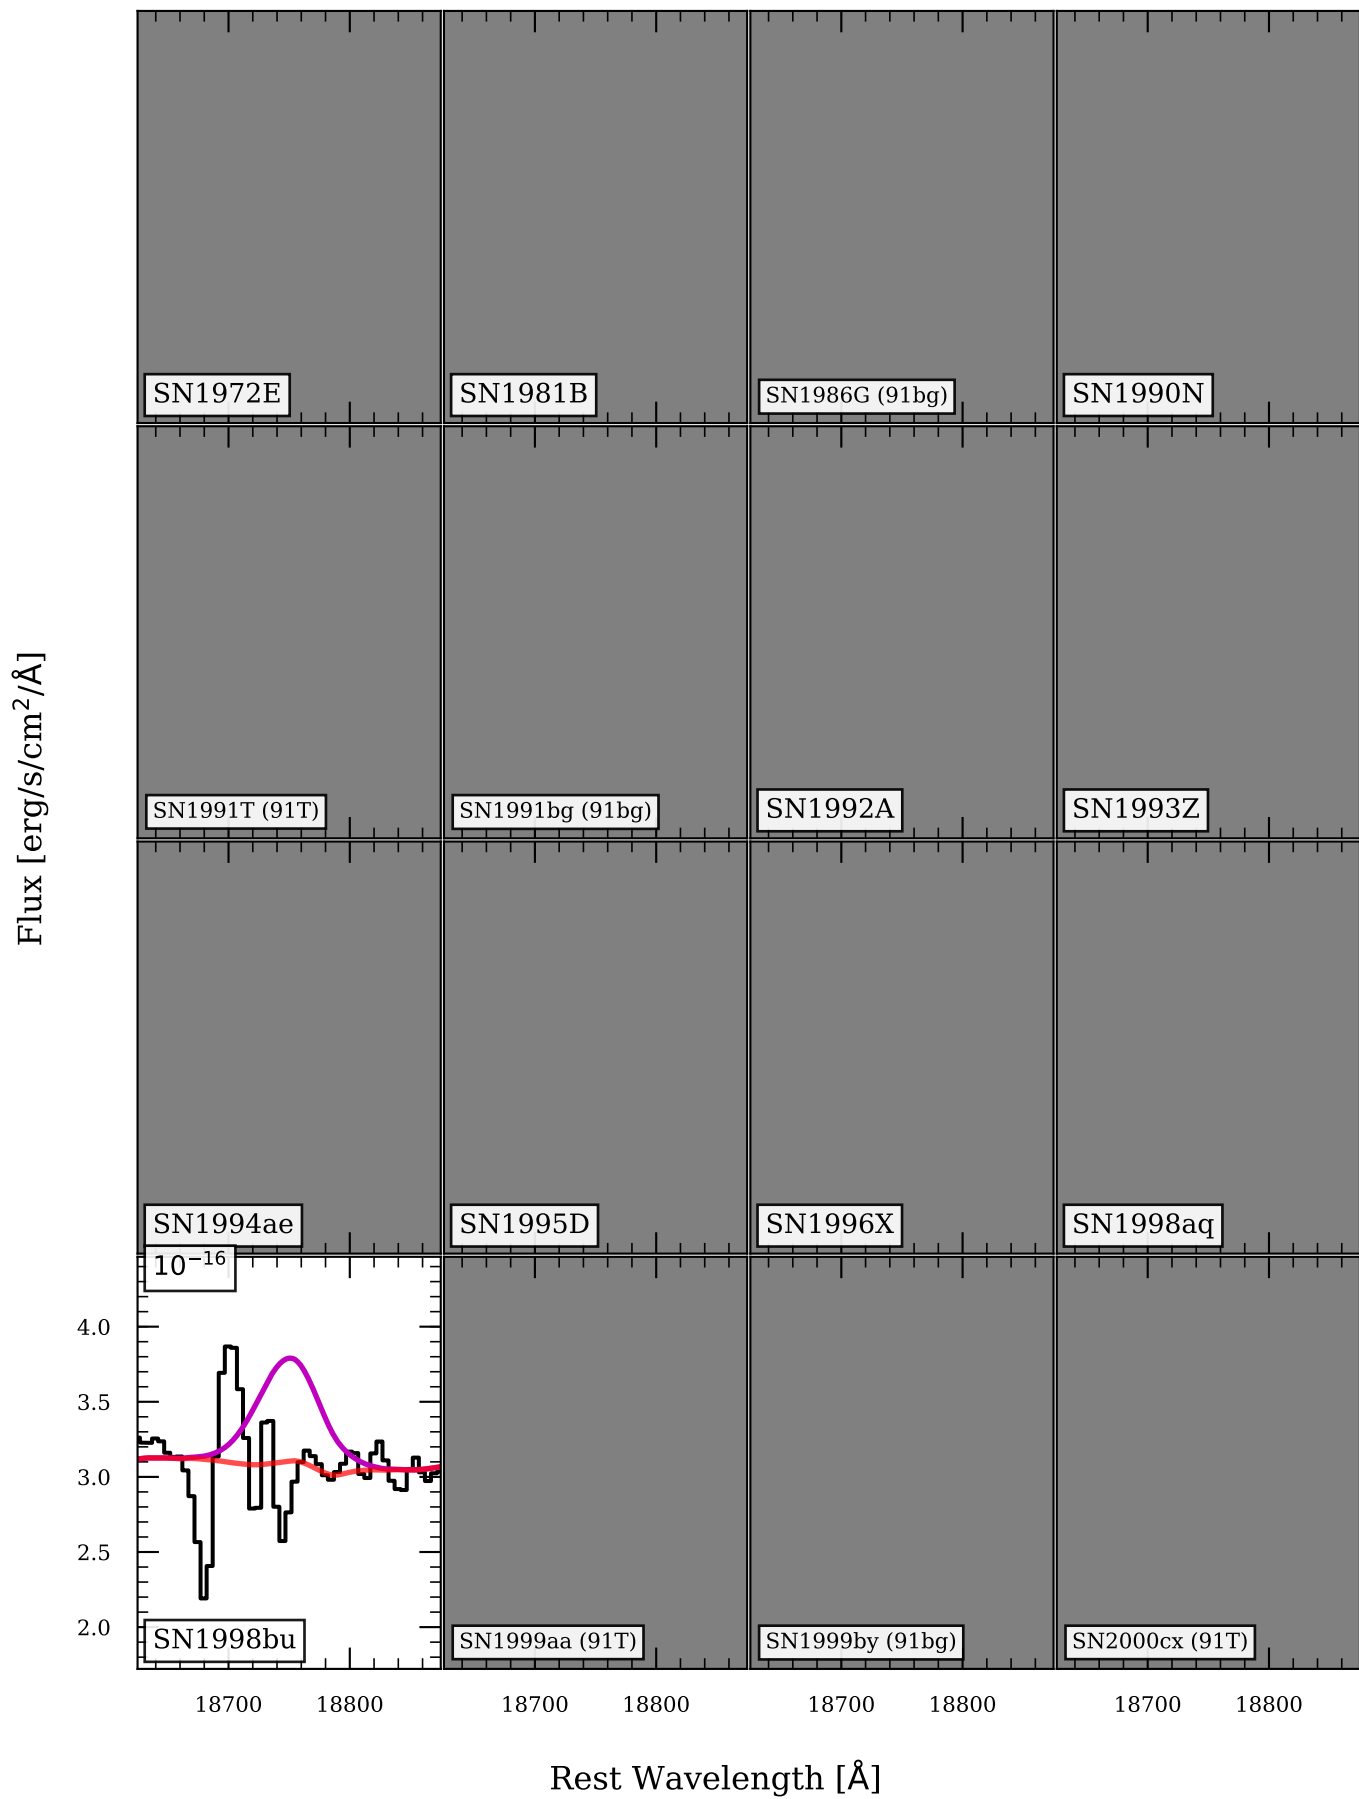

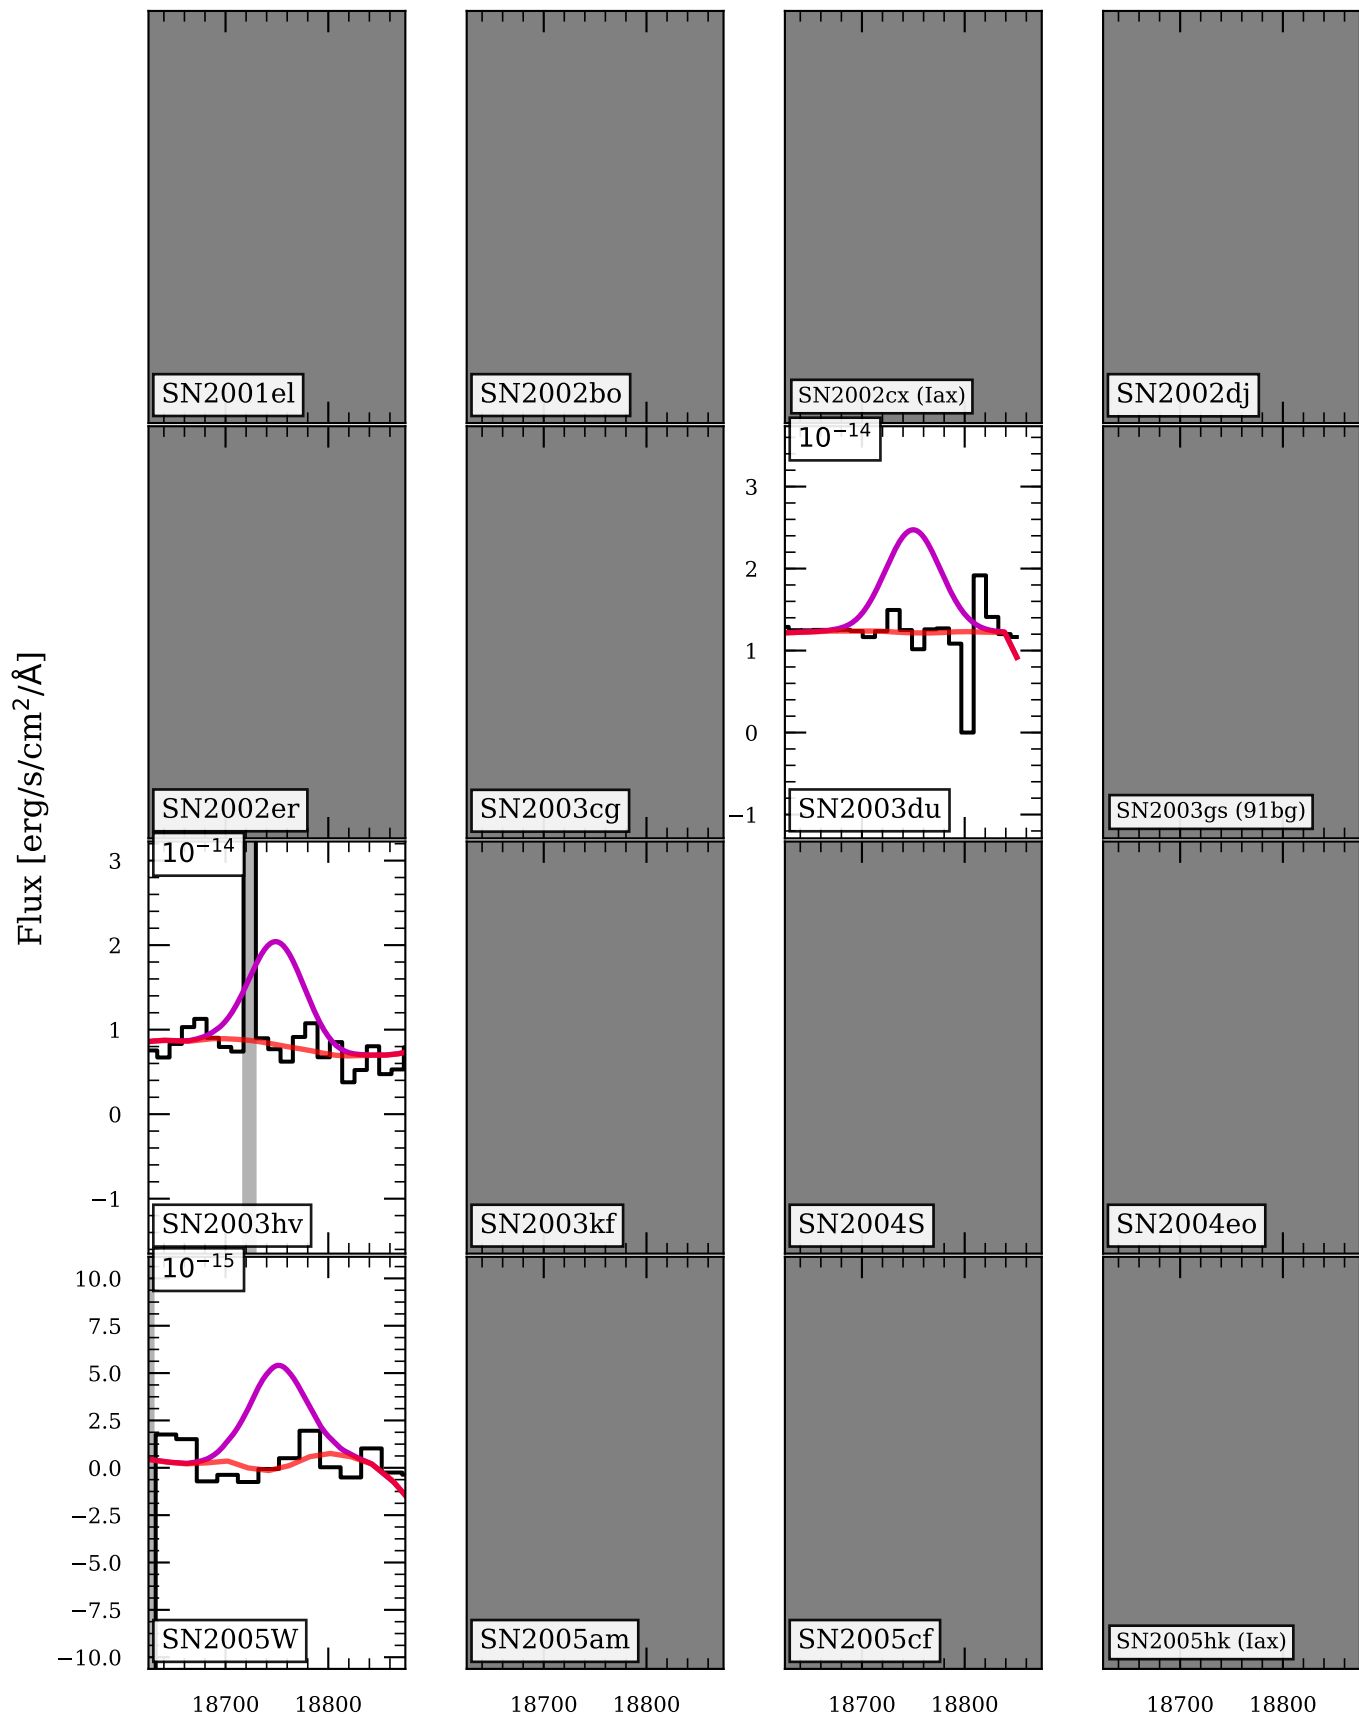

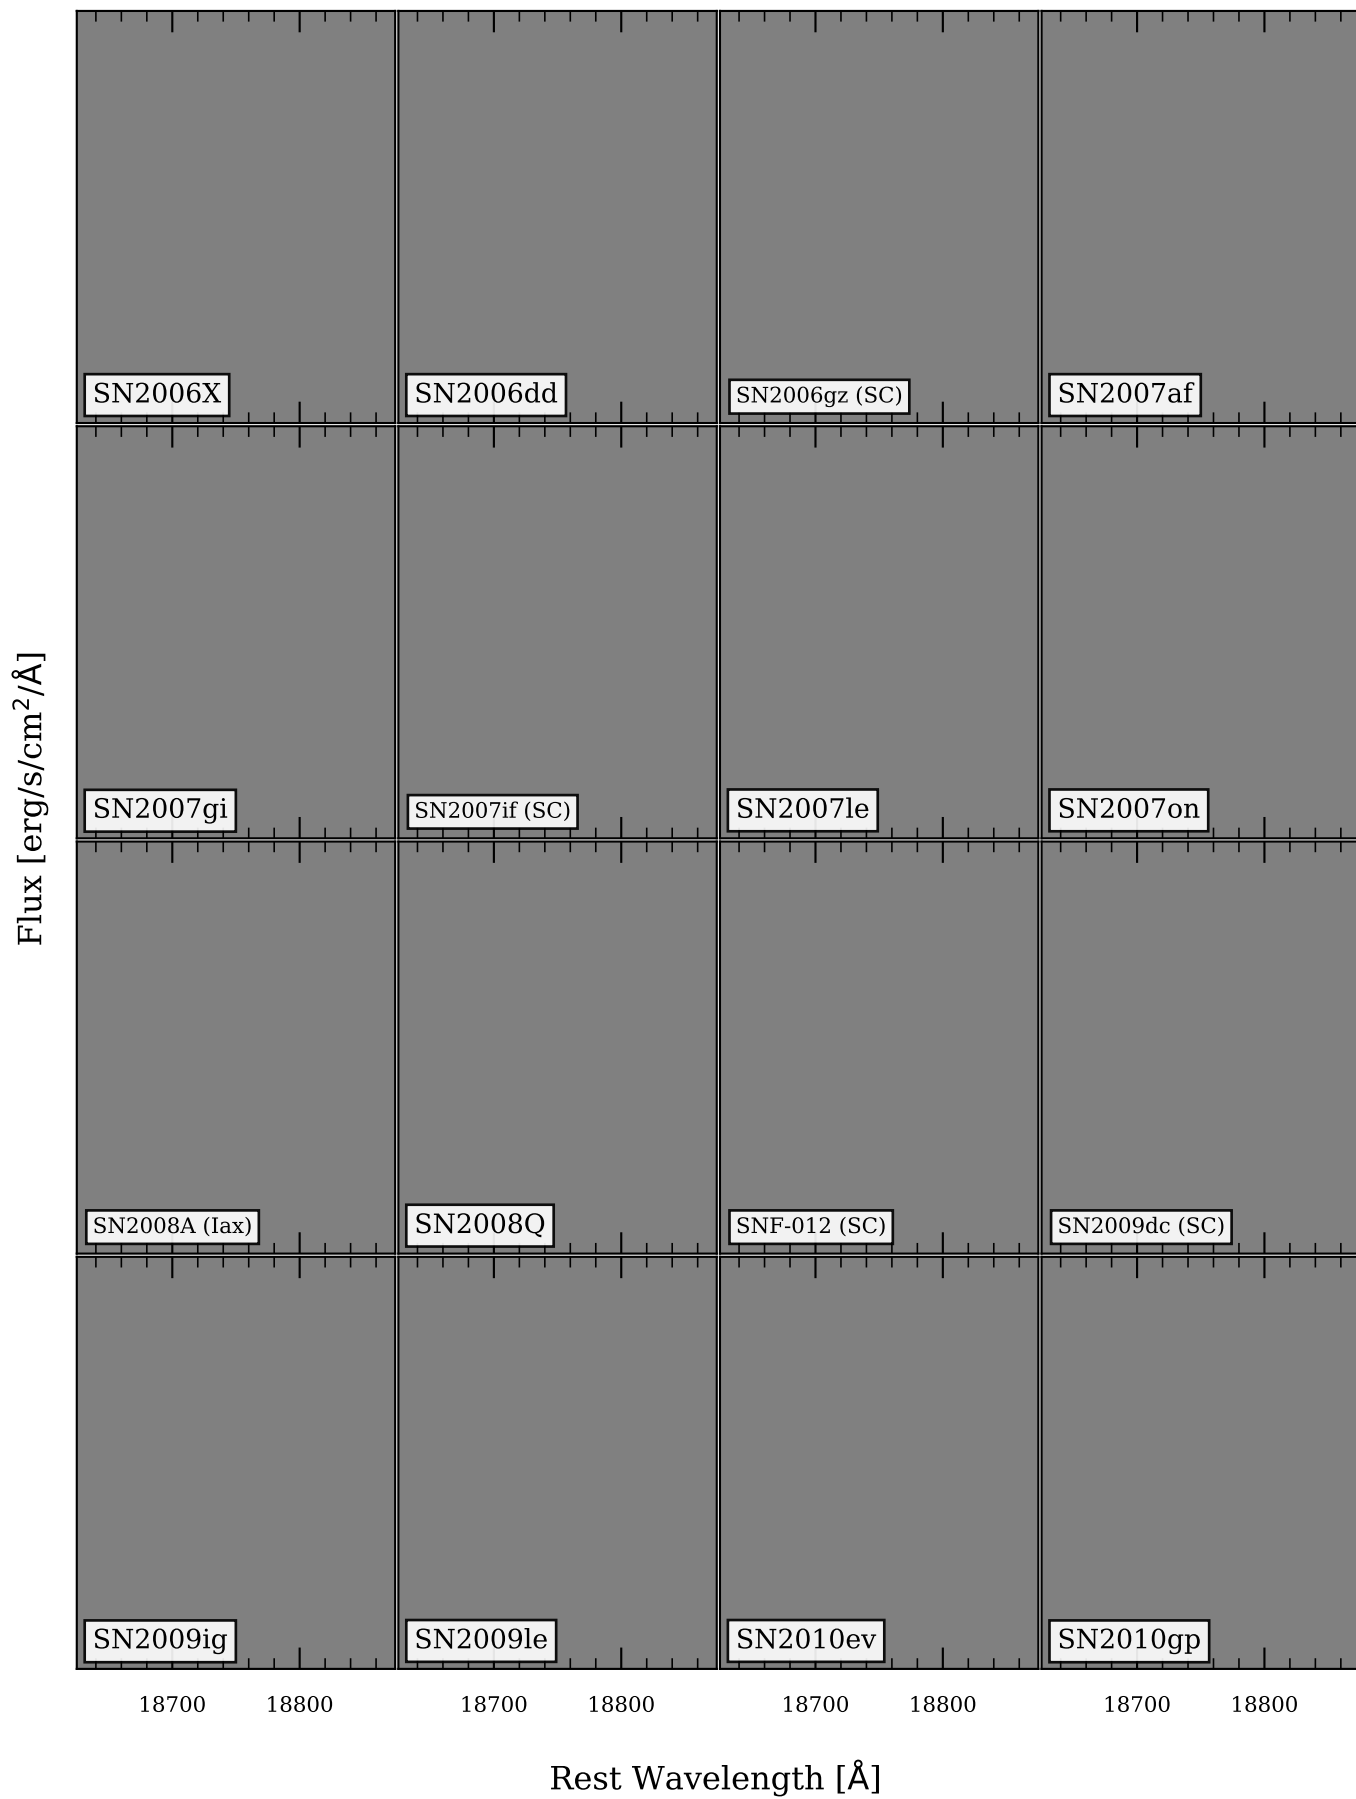

Flux [erg/s/cm<sup>2</sup>/Å]

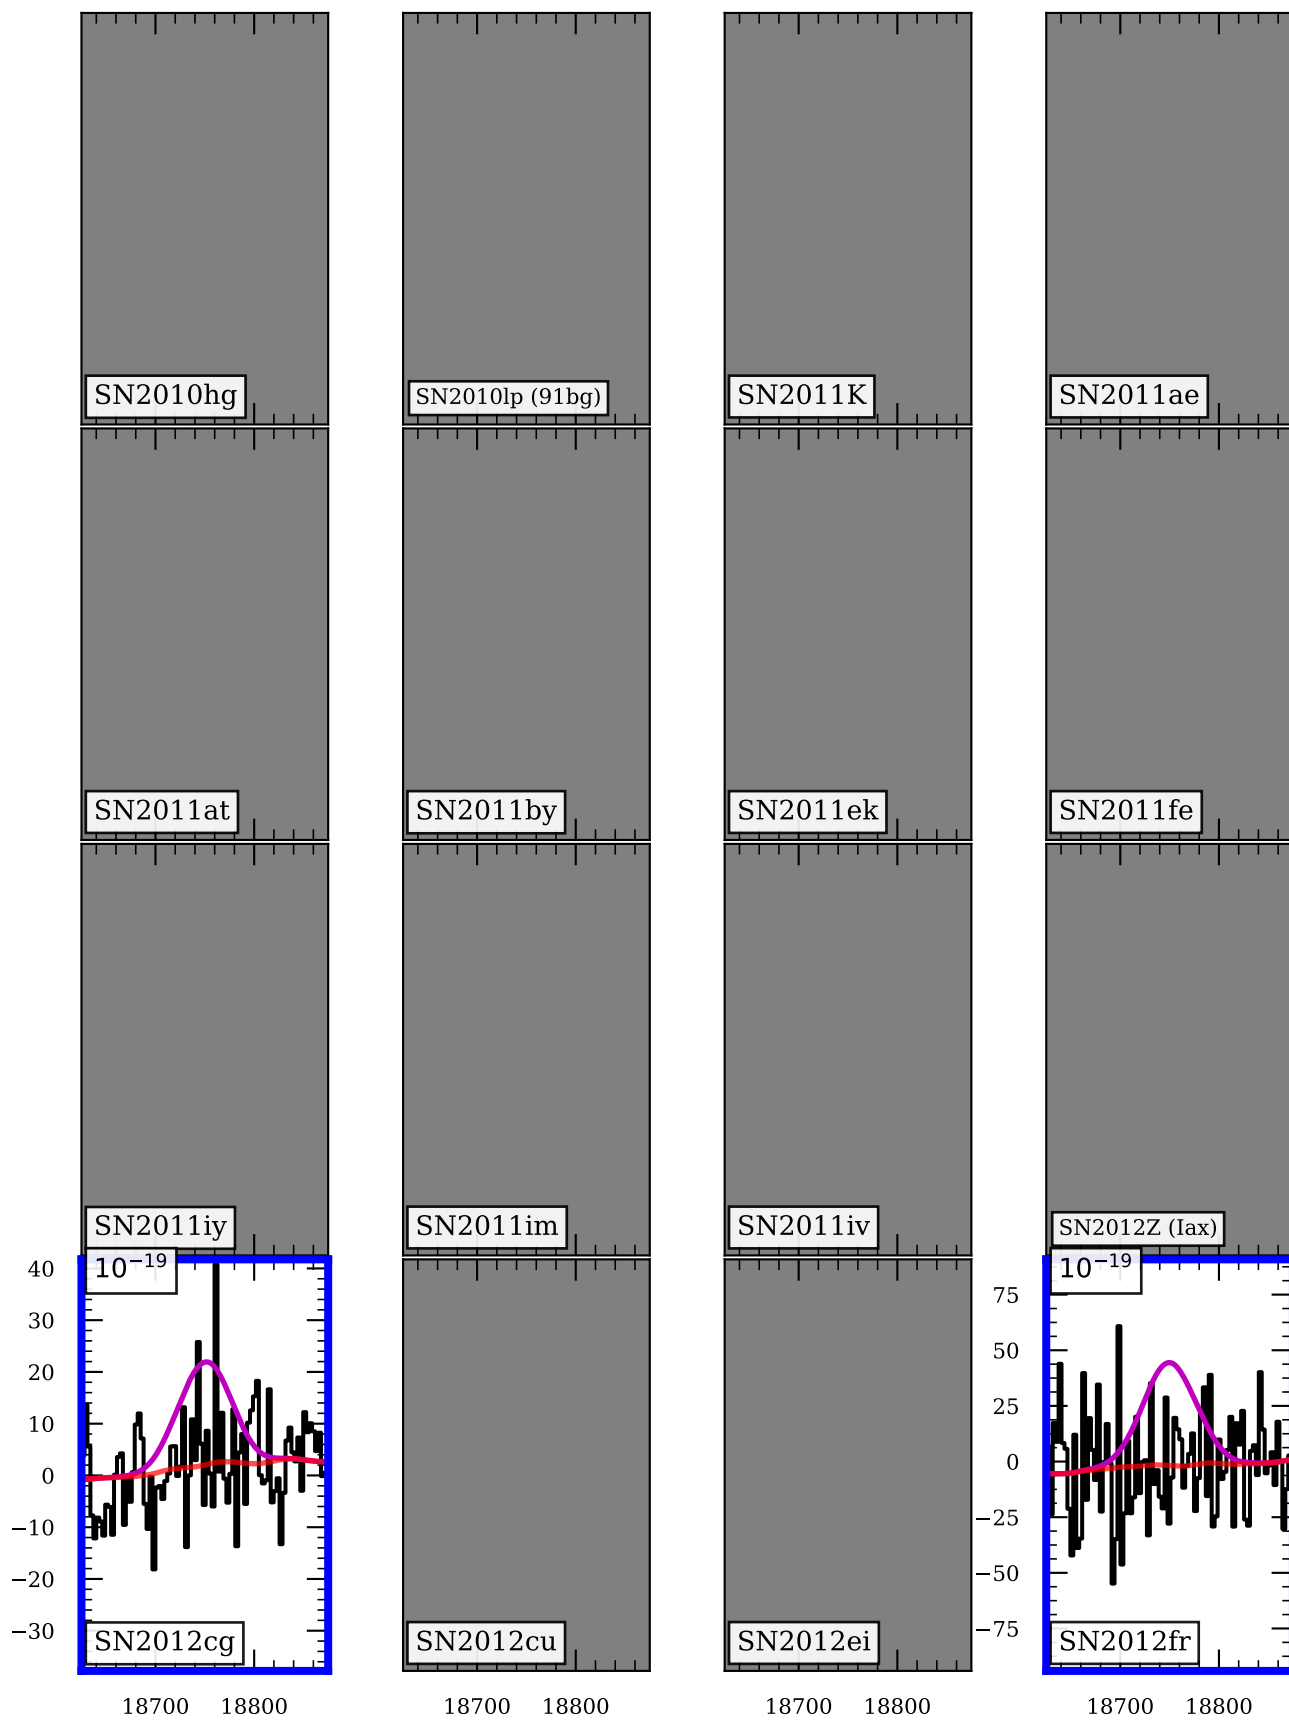

Rest Wavelength [Å]

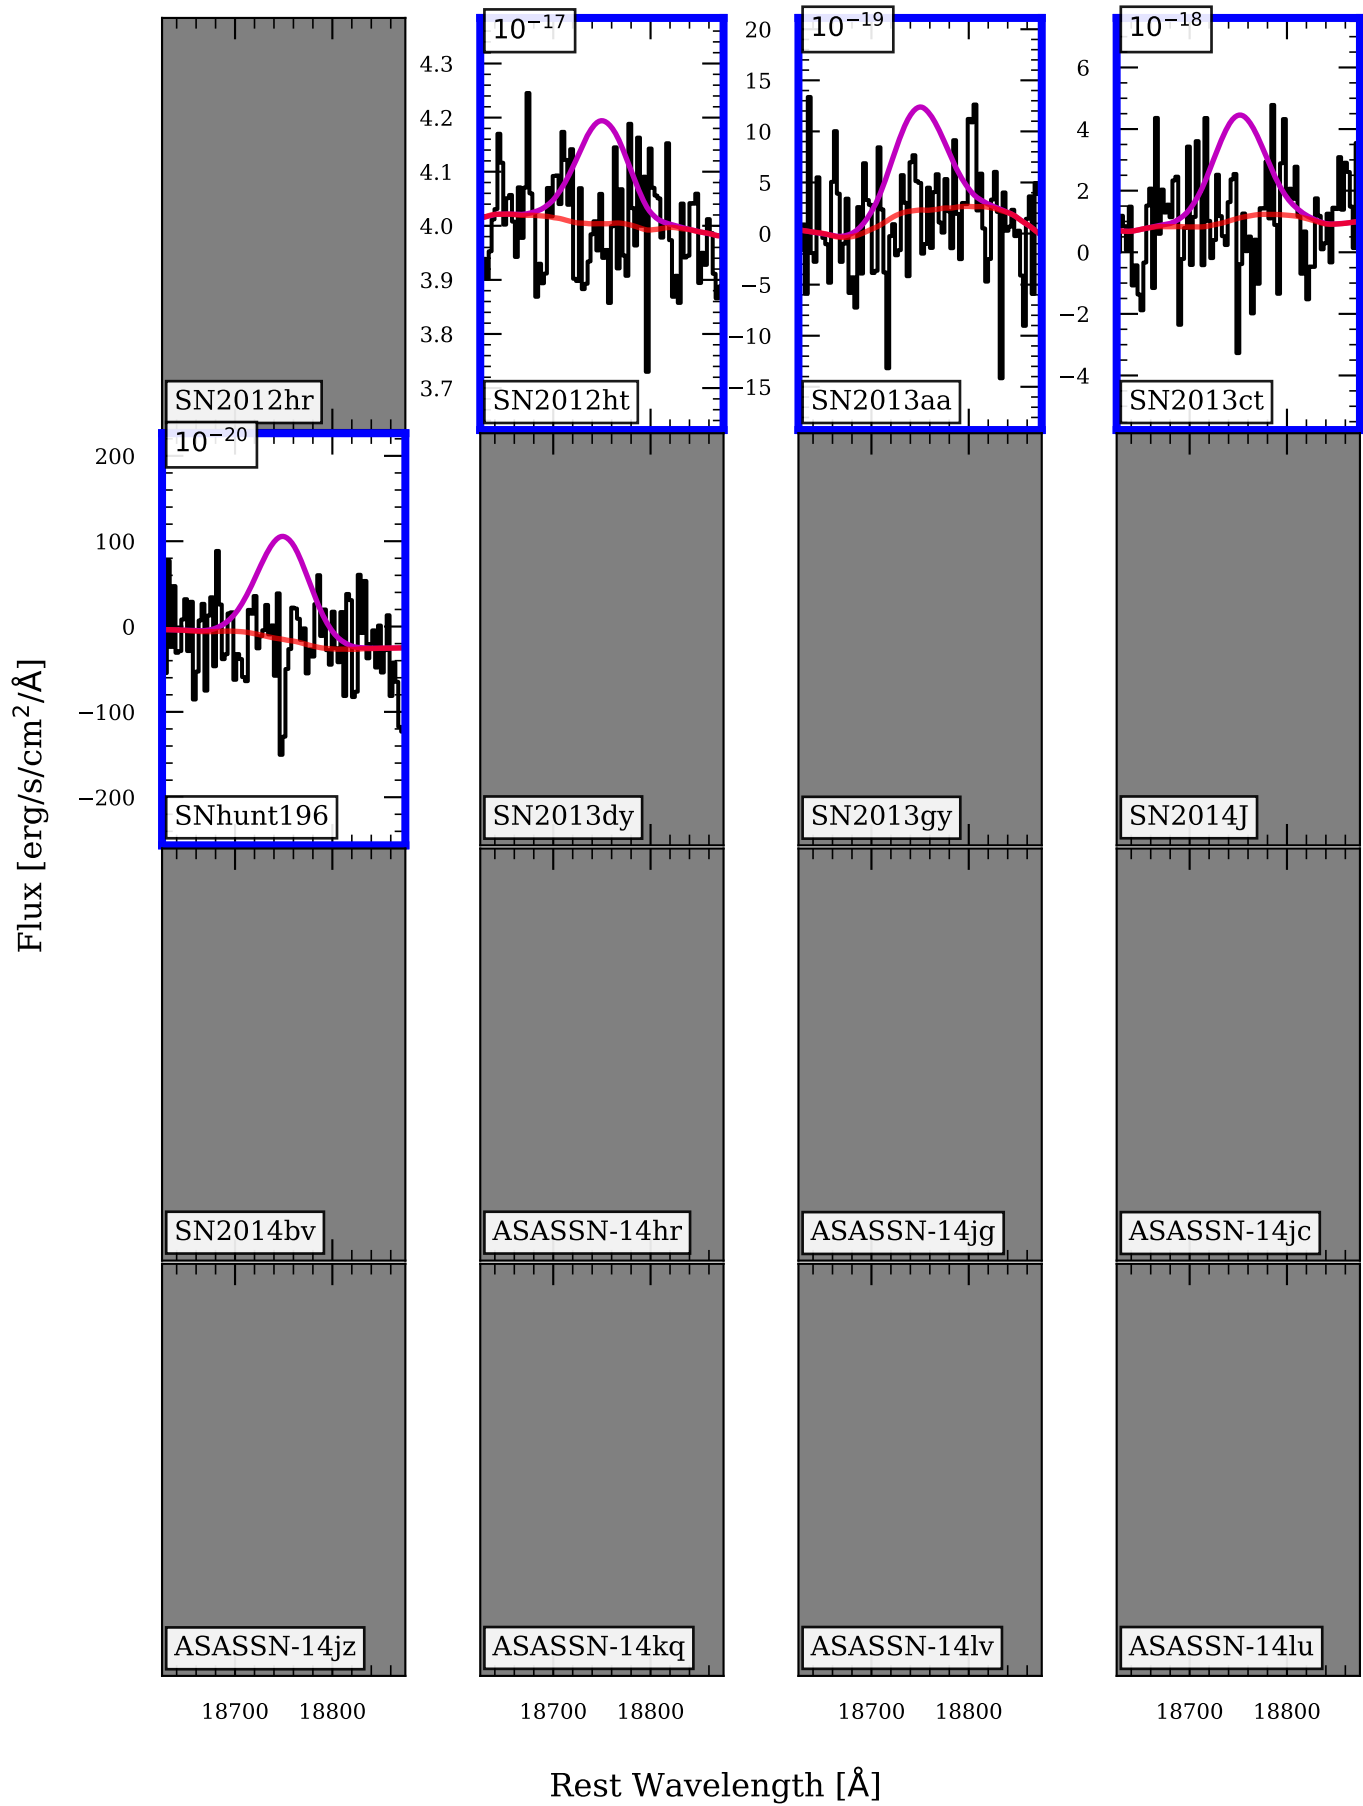

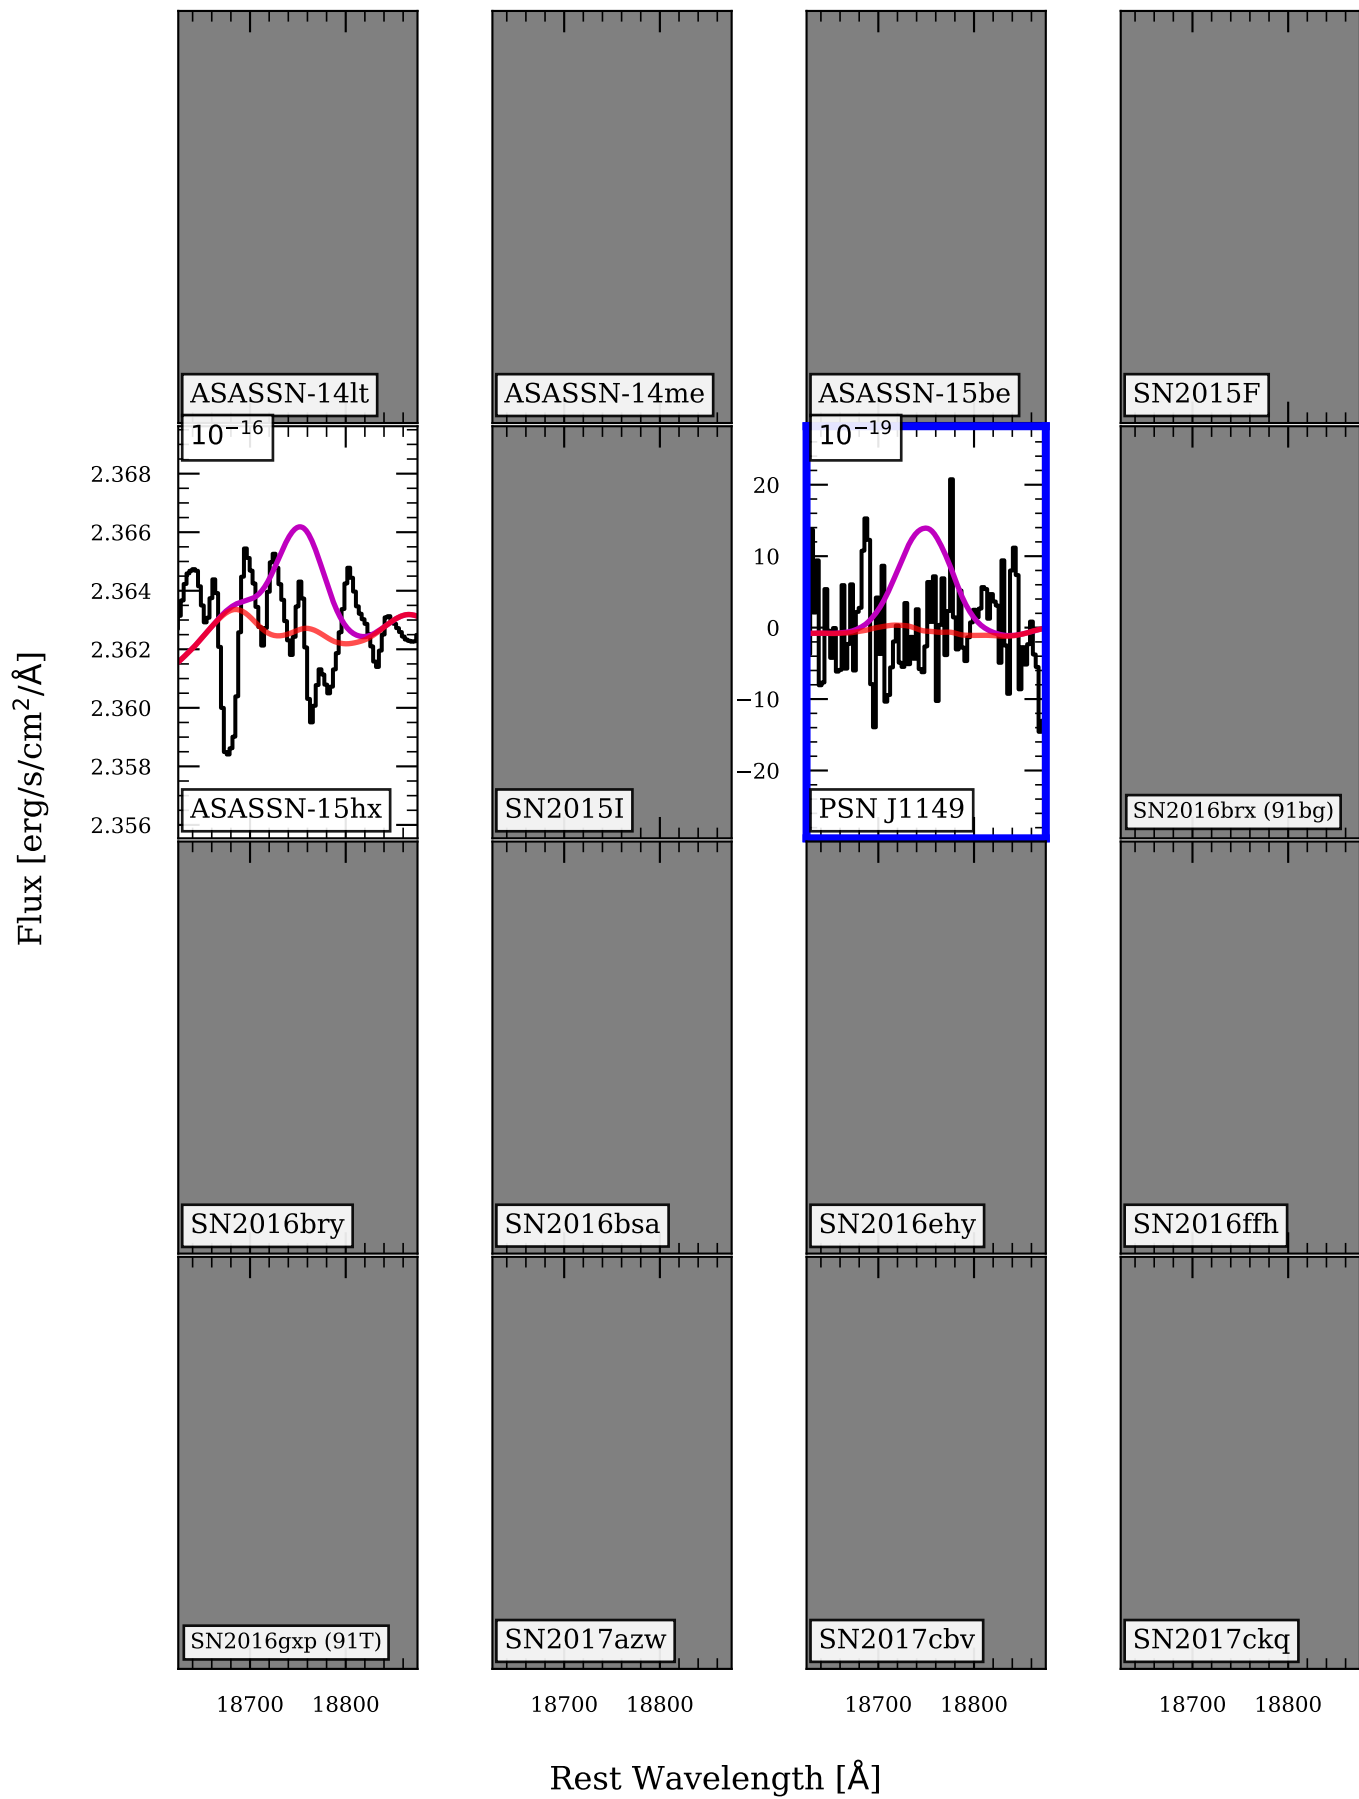

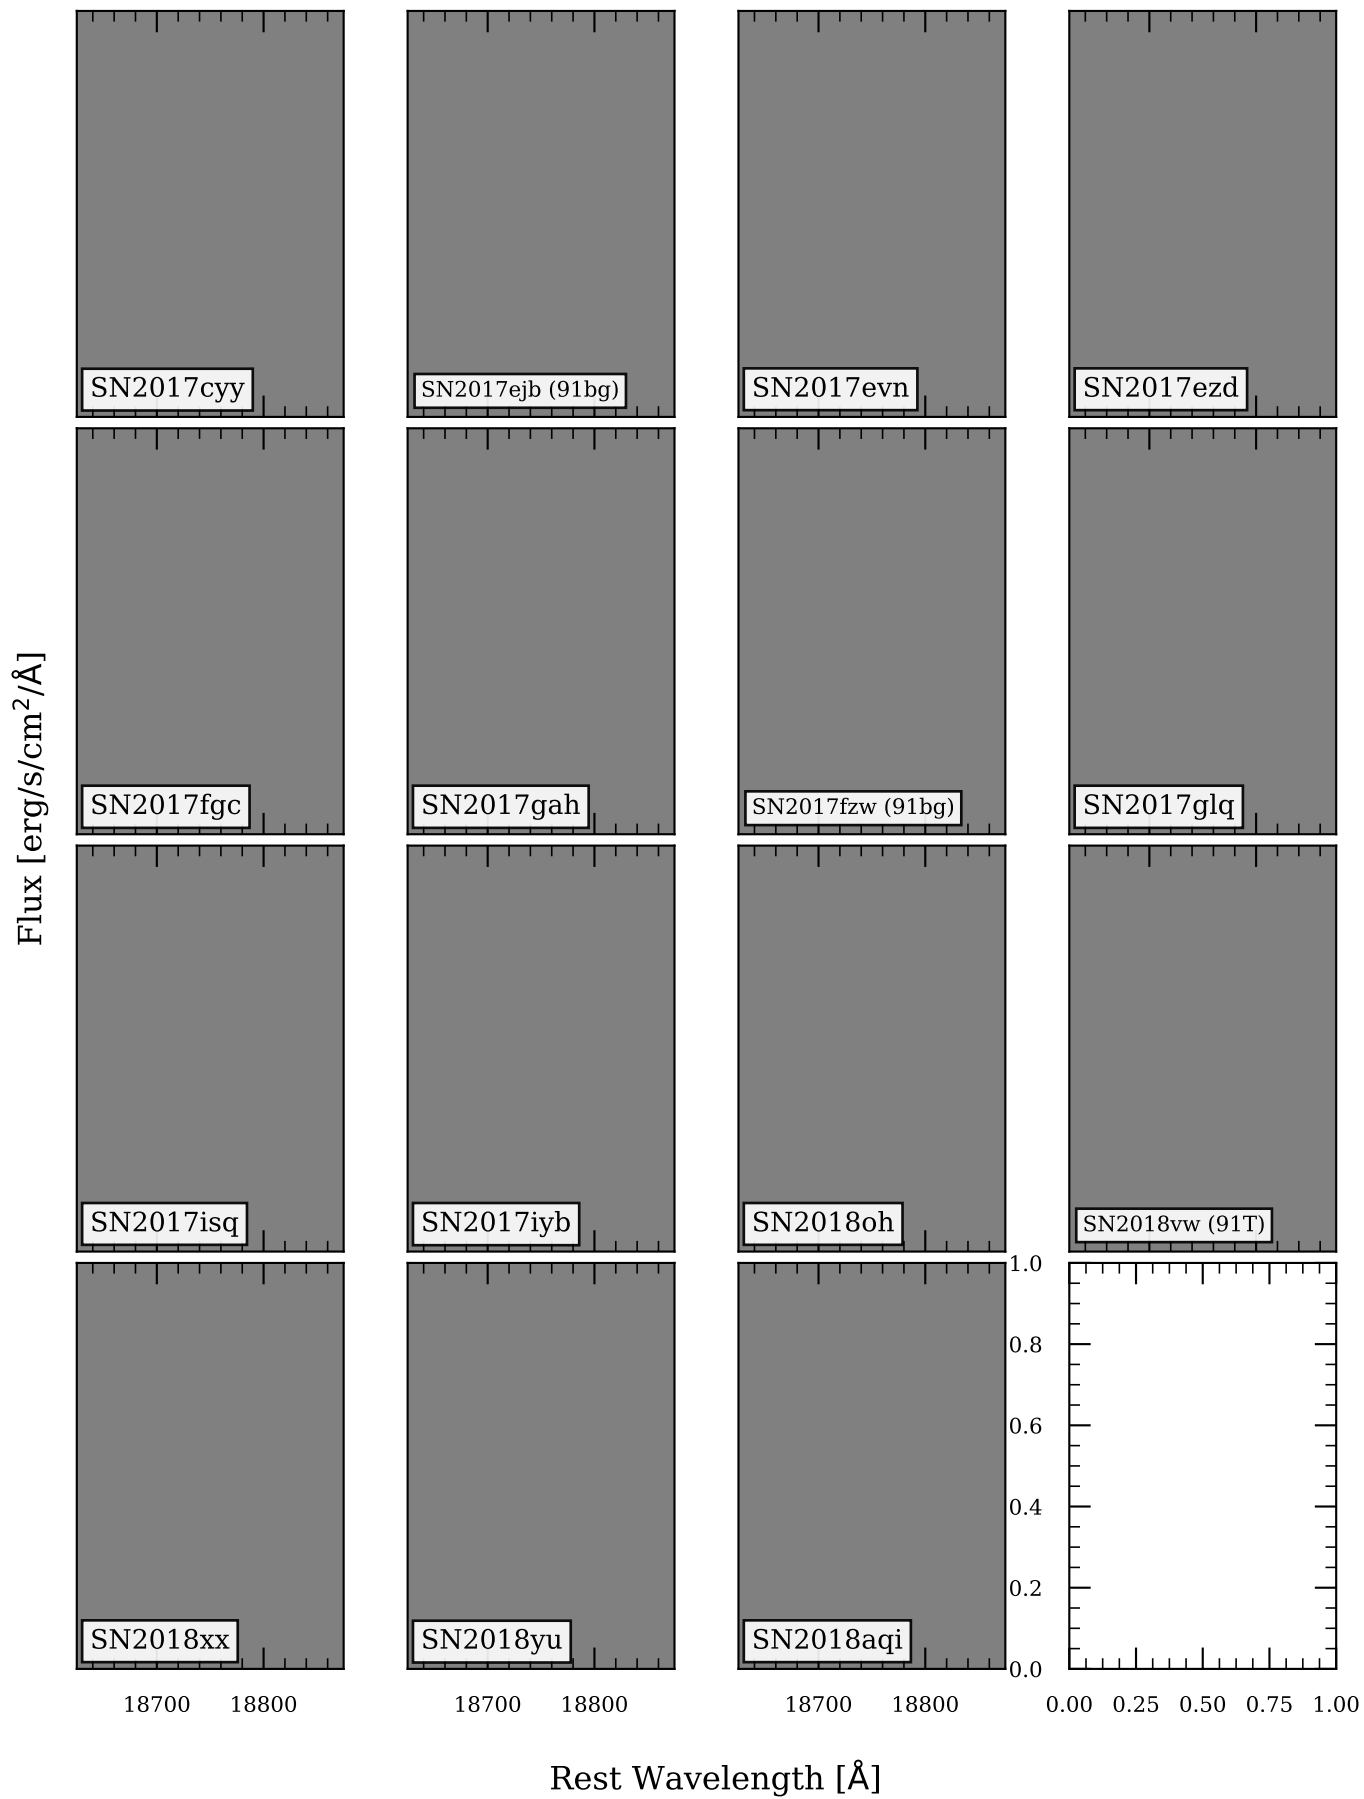

Supplement: Supplementary file 8 [file Pa-final.pdf]
