# Supplementary material for: Nebular Spectra of 111 Type Ia Supernovae Disfavor Single Degenerate Progenitors
Source: arXiv:1903.05115 ancillary file (2019-10-31)

**$P\beta$**

**12820 Å**

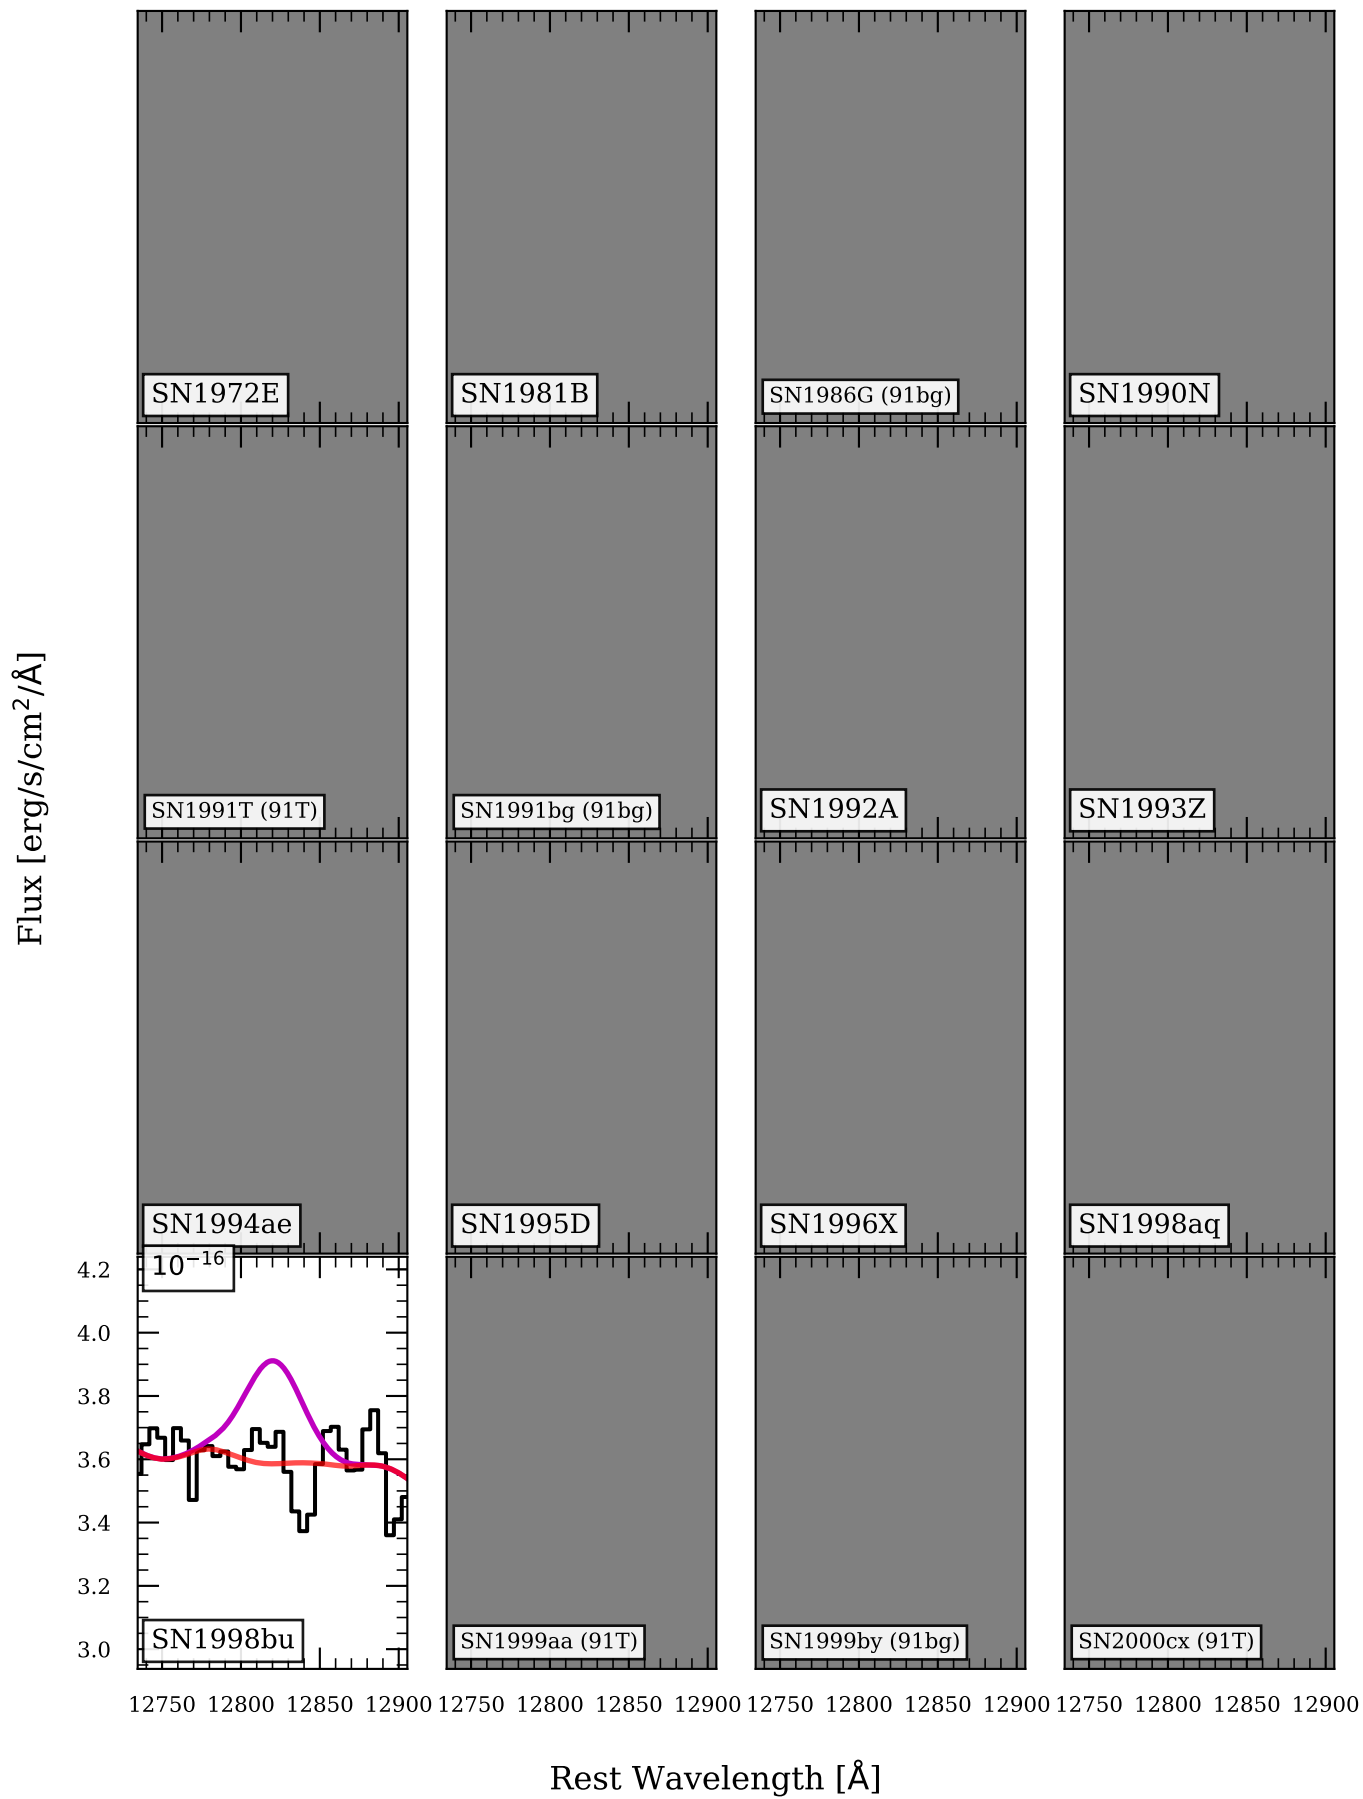

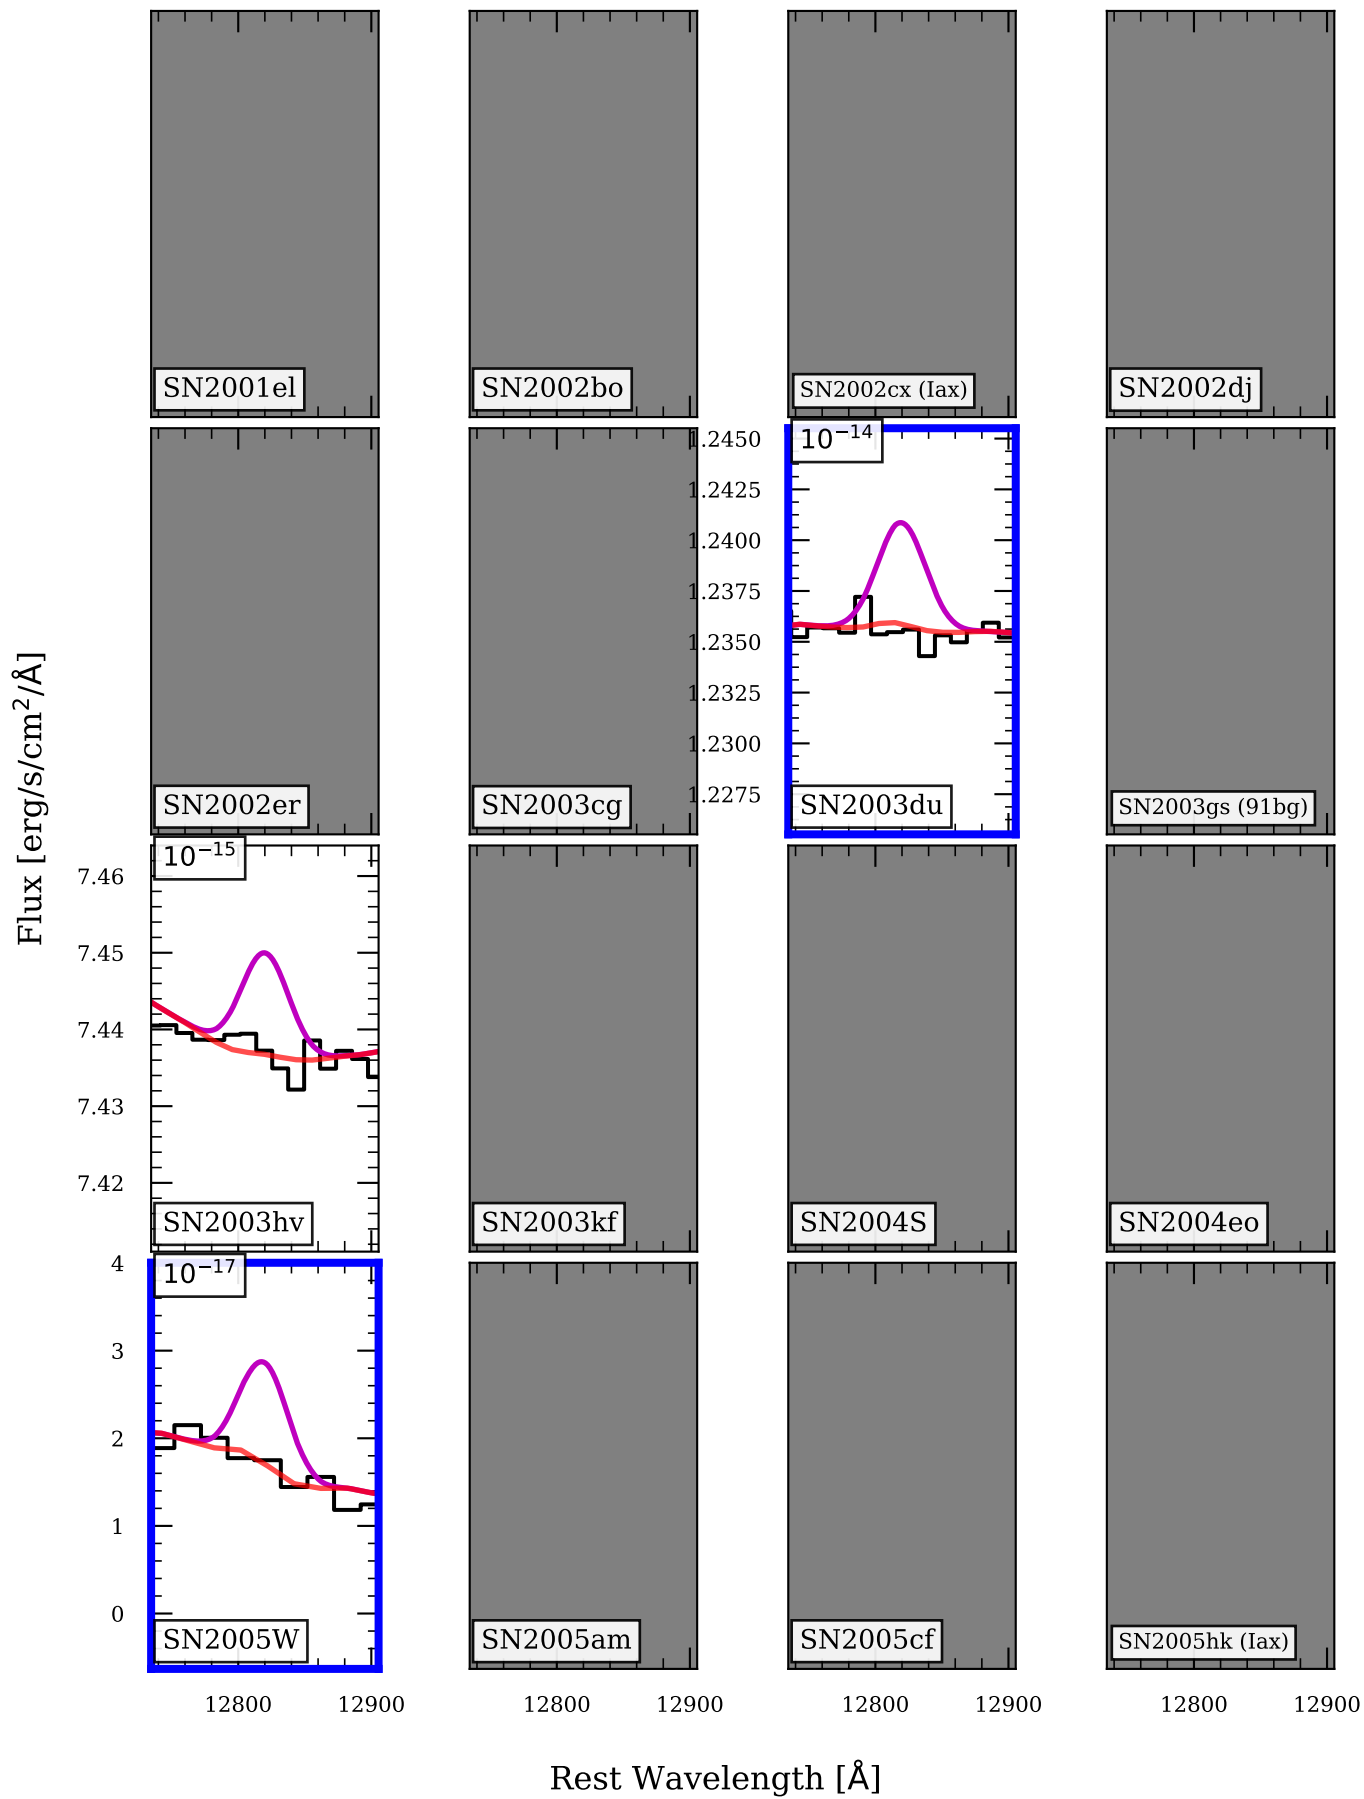

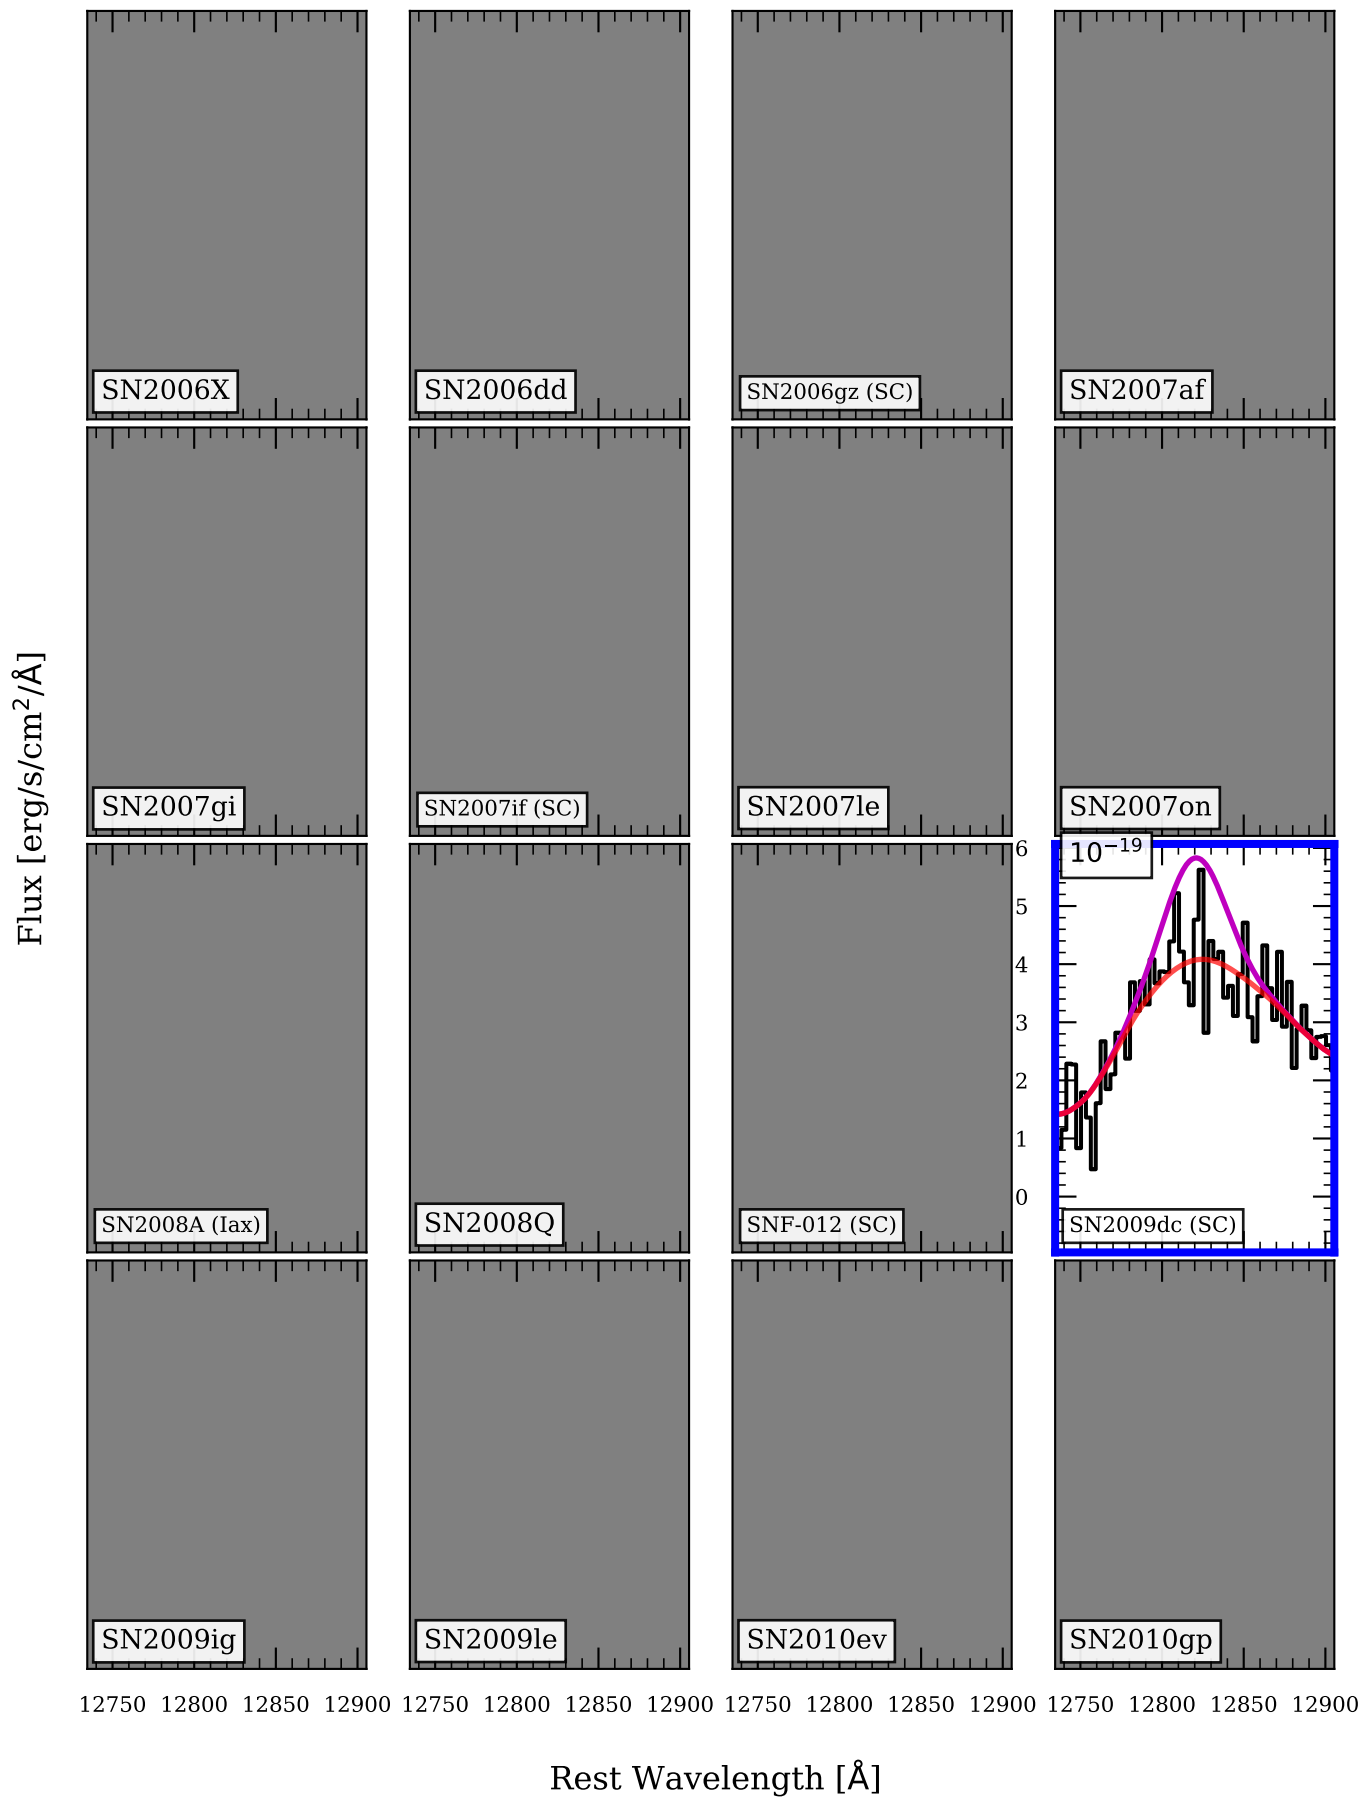

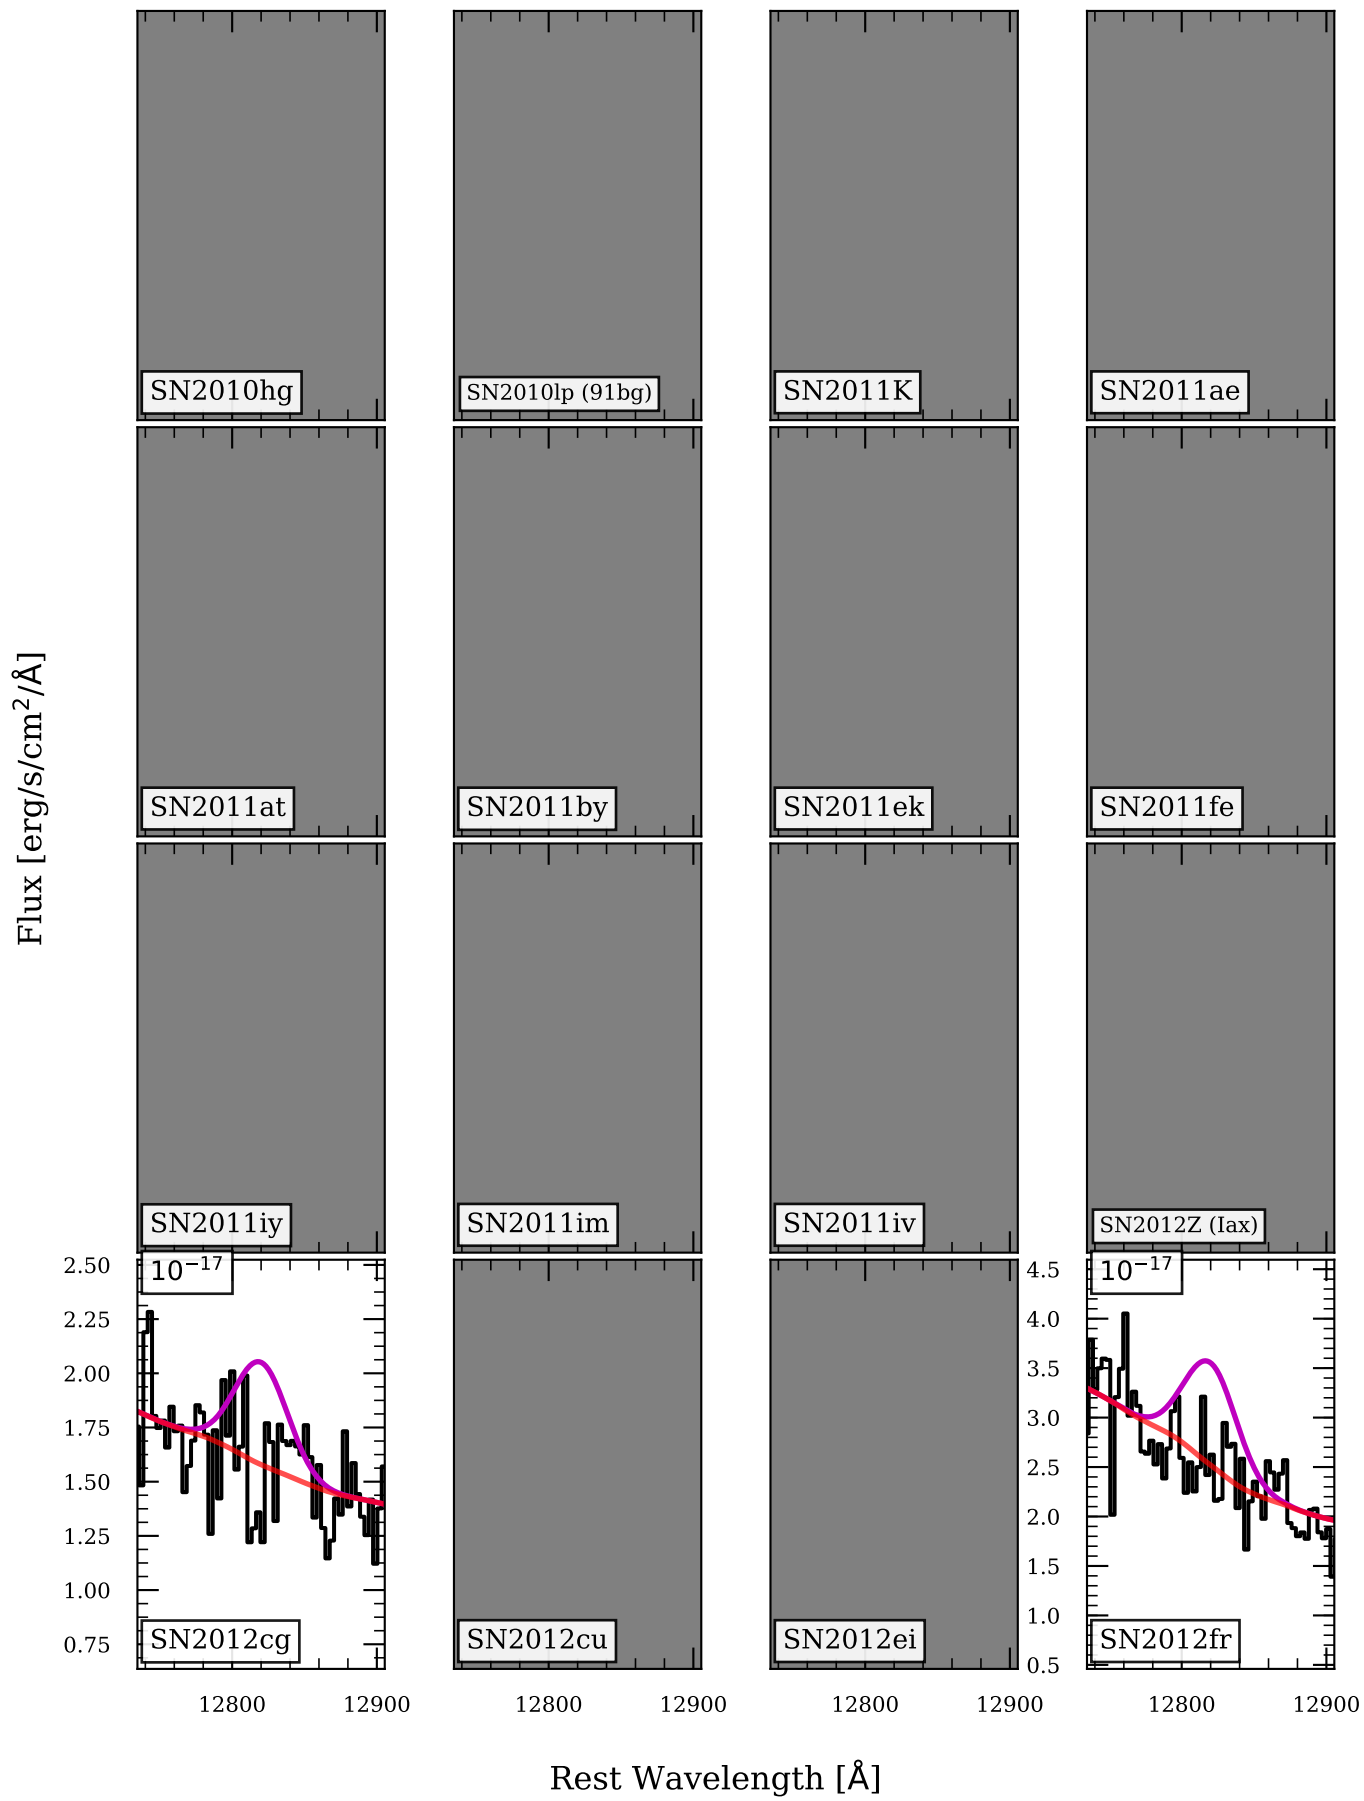

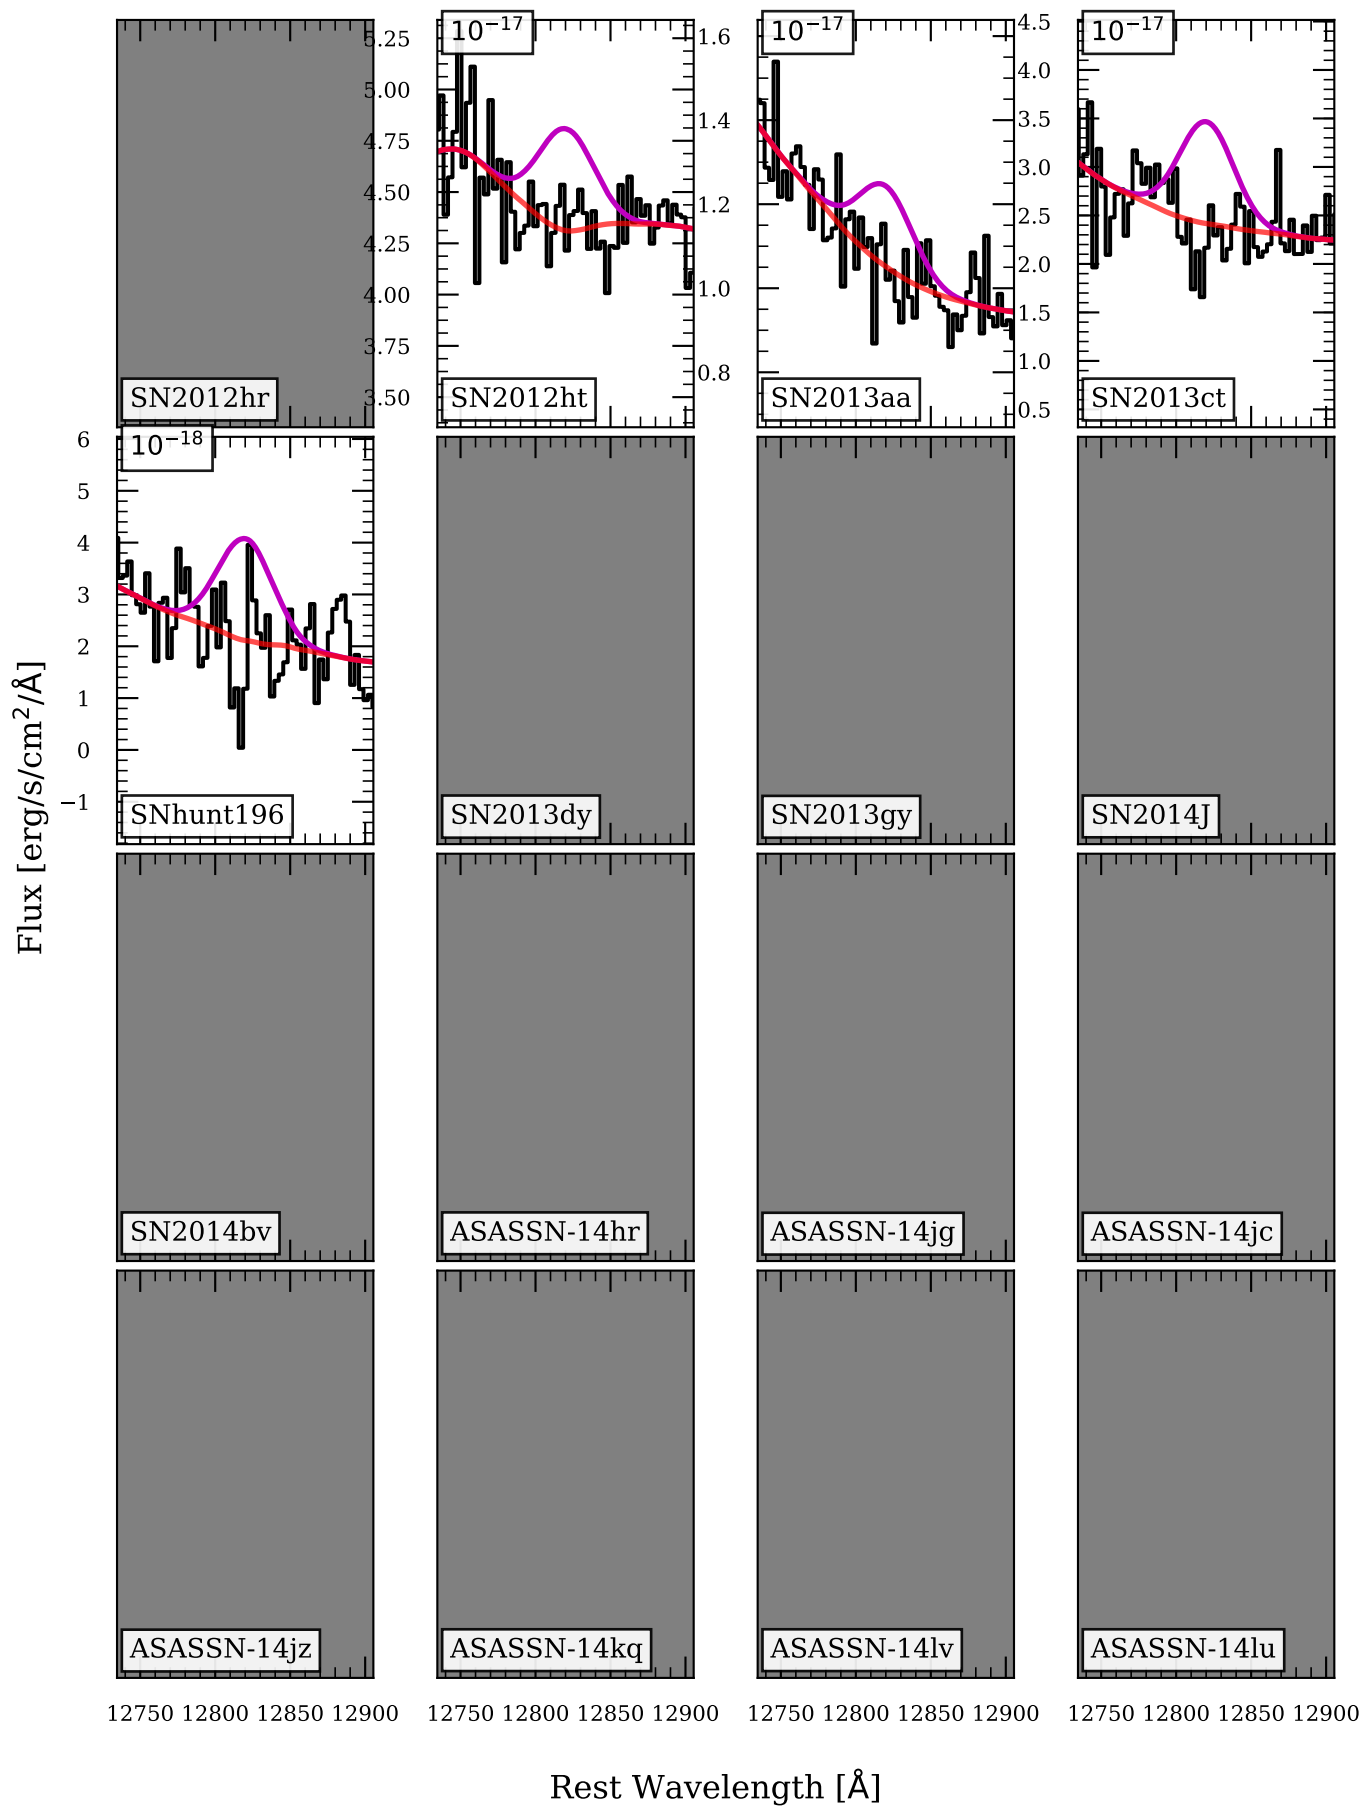

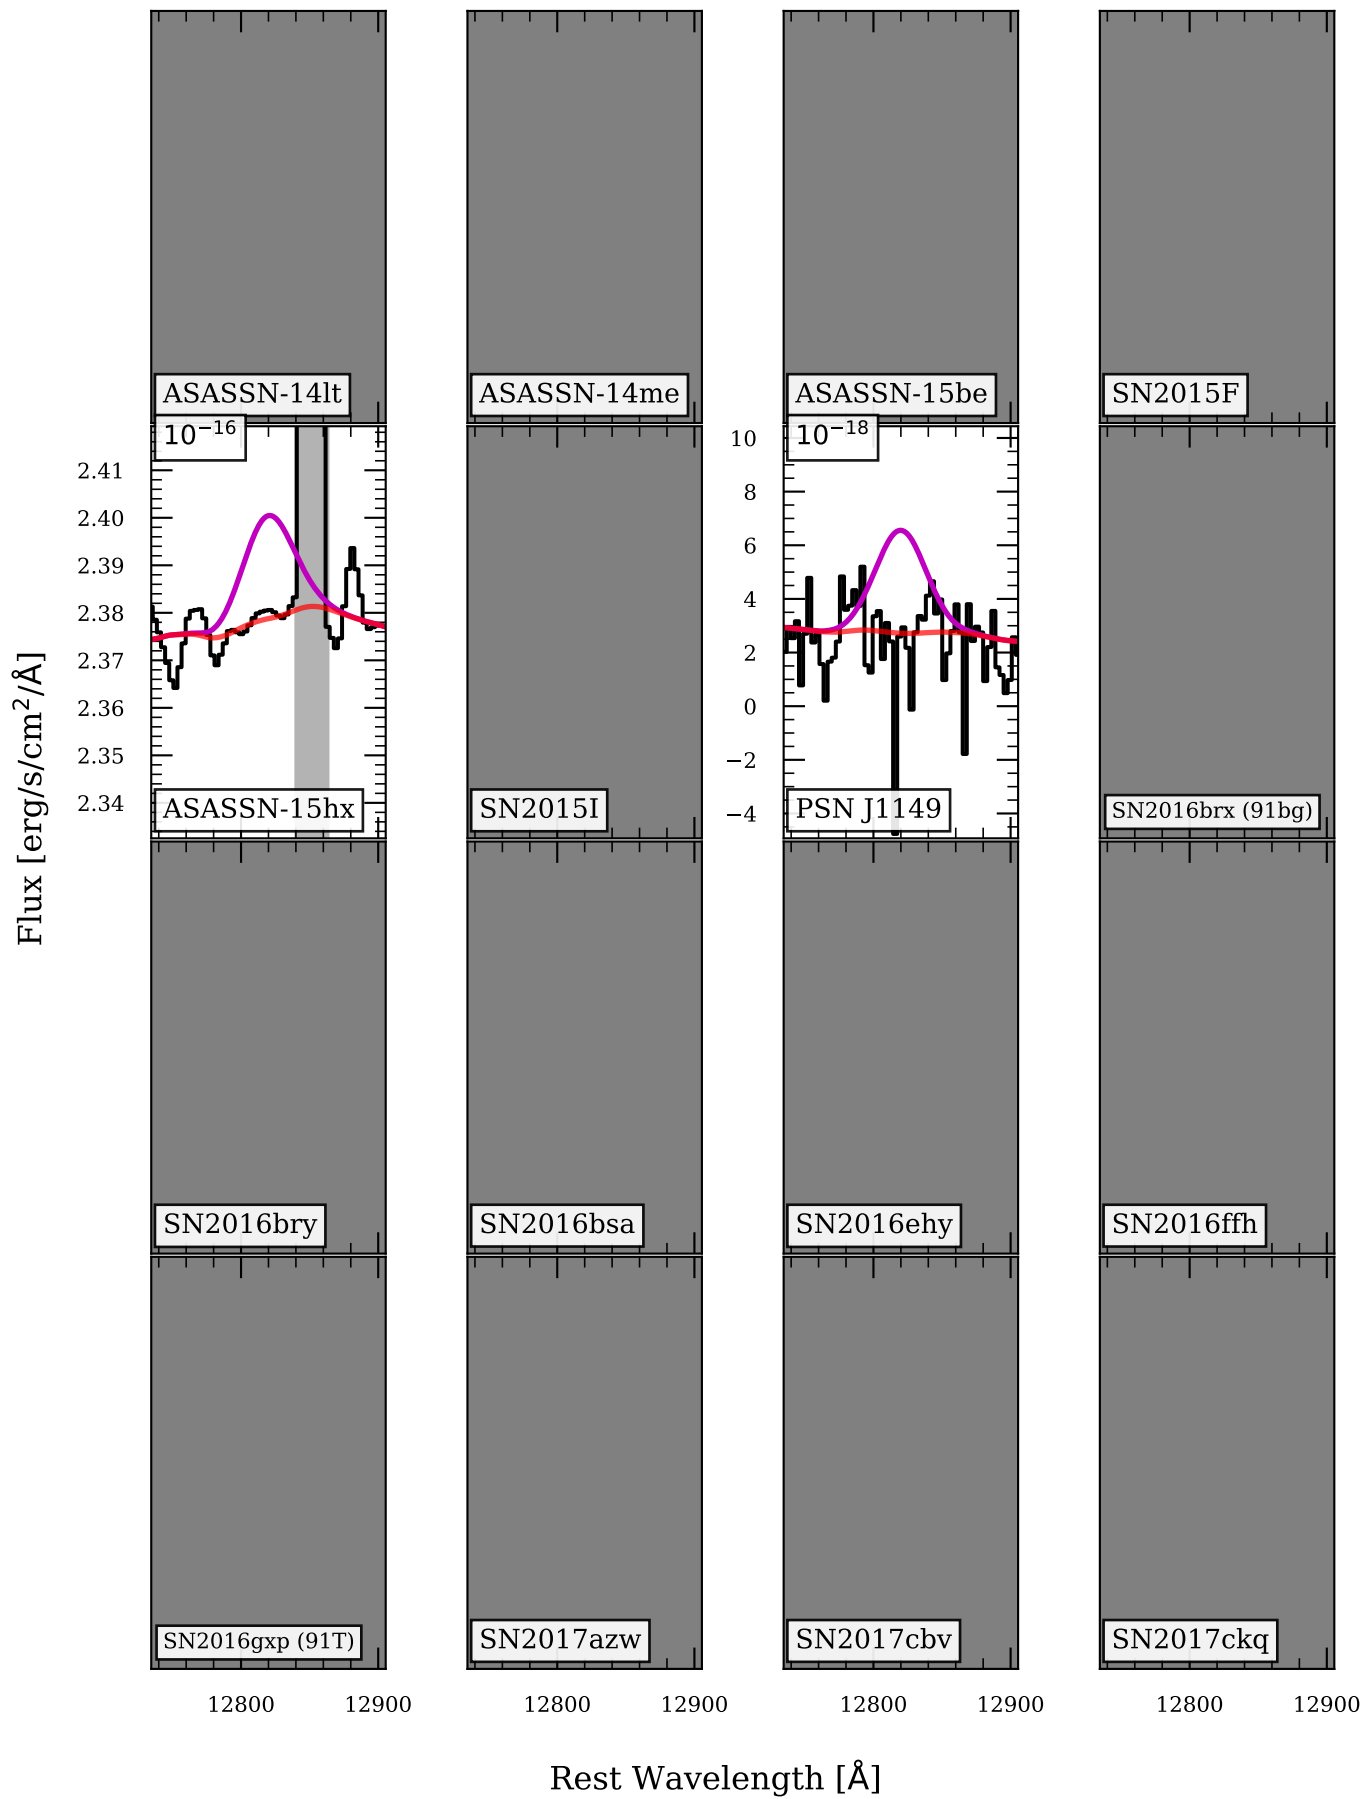

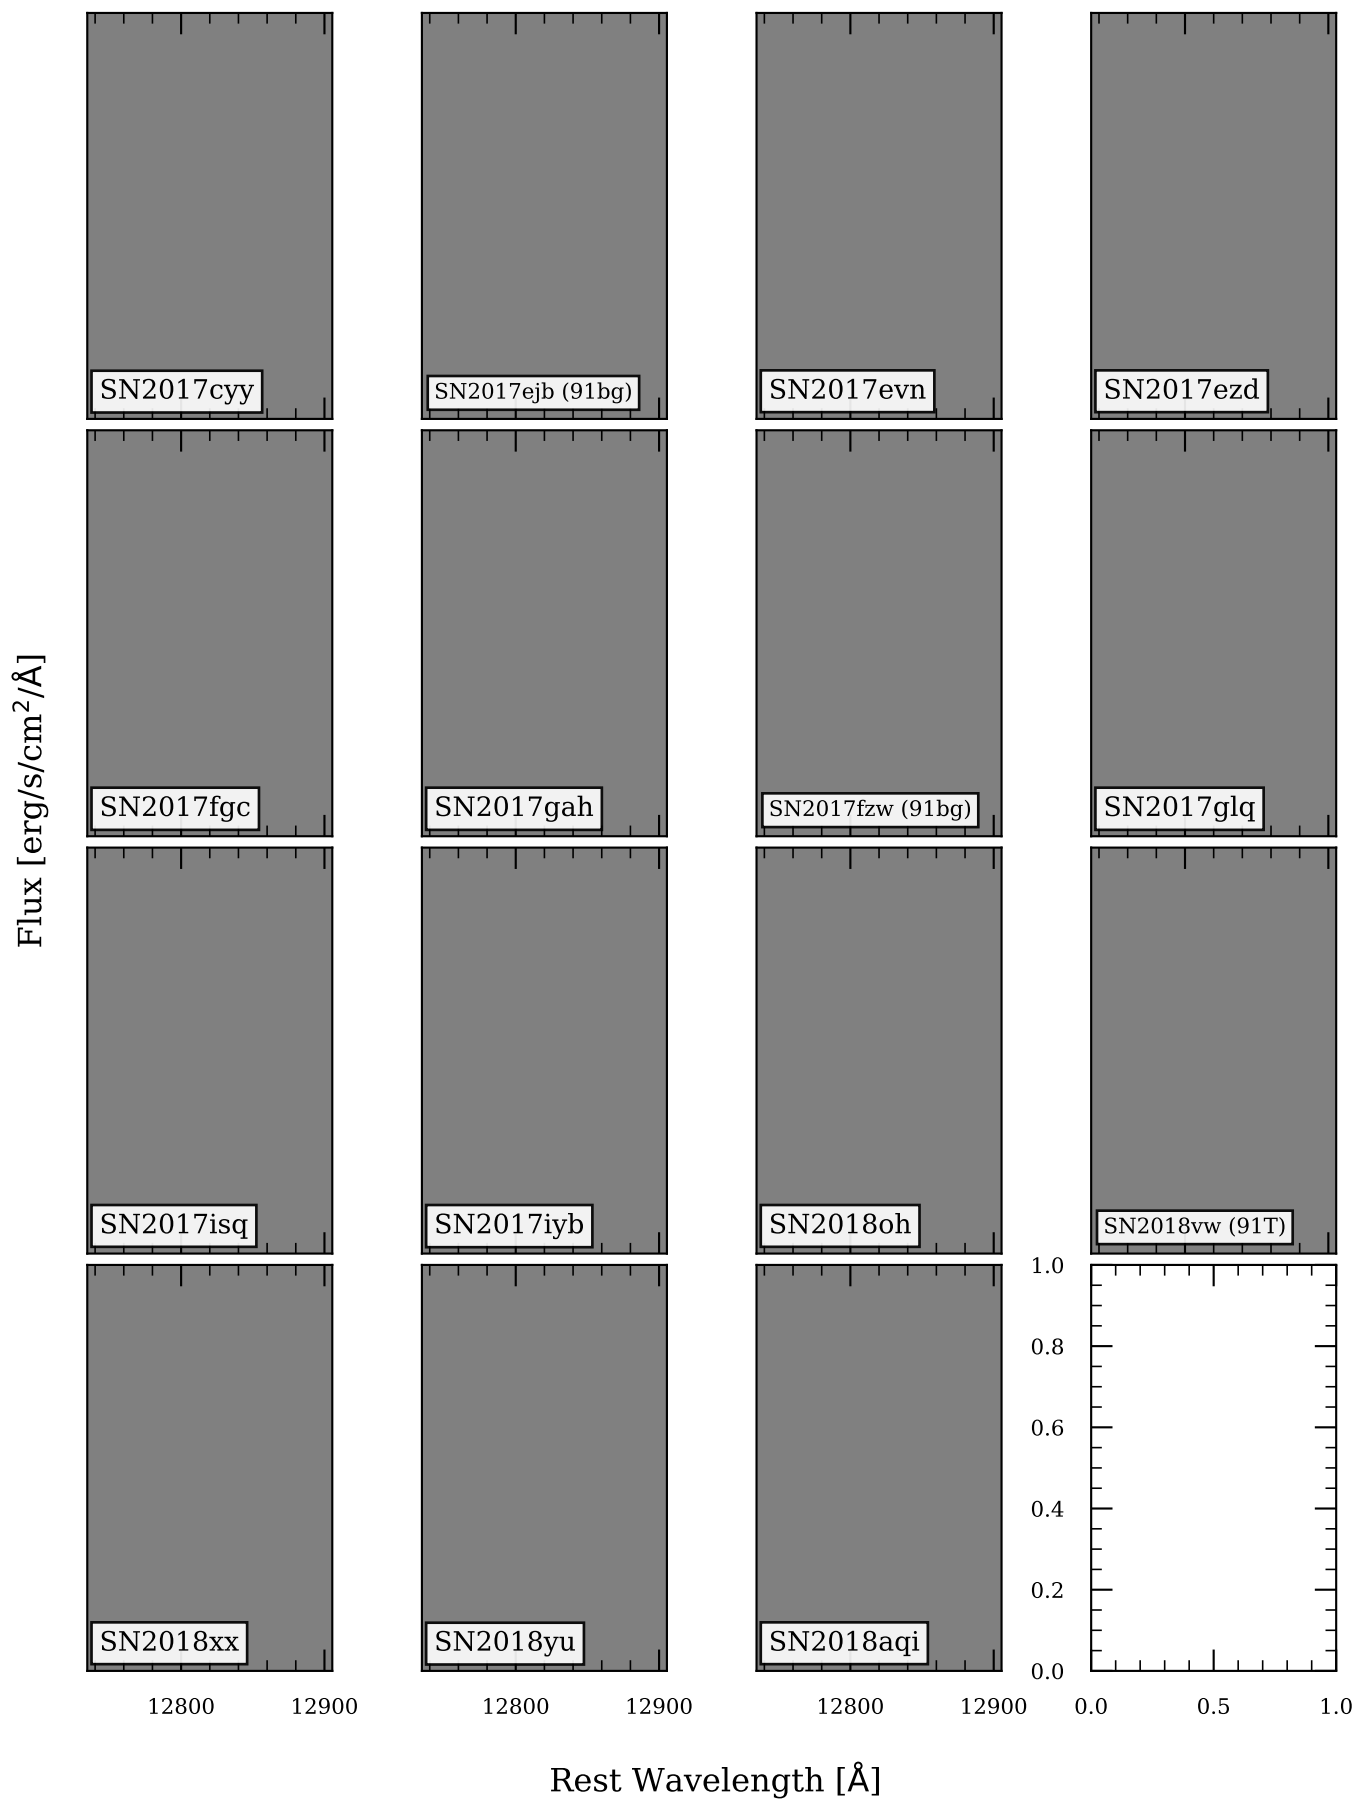

Supplement: Supplementary file 9 [file Pb-final.pdf]
